# Supplementary material for: Spin-Momentum Impedance and Filtering at a Spin-Coupled Absorbing Boundary
Source: arXiv:2606.25650 source file (2026-12-03)
Supplement: Supplementary file 1 [file 02_supplement.tex]

% Compile from a terminal with either
%   latexmk -pdf SupplementaryDoc_clean.tex
% or the explicit REVTeX sequence
%   pdflatex SupplementaryDoc_clean.tex
%   bibtex SupplementaryDoc_clean
%   pdflatex SupplementaryDoc_clean.tex
%   pdflatex SupplementaryDoc_clean.tex
% If a references.bib file is present, it is included automatically at the end.

\documentclass[aps,prl,preprint,superscriptaddress,longbibliography,nofootinbib,secnumarabic]{revtex4-2}

% Encoding and fonts
\usepackage[utf8]{inputenc}
\usepackage[T1]{fontenc}

% Mathematics
\usepackage{amsmath,amssymb,amsthm,bm,mathtools,mathrsfs}

% Figures, tables, units, and diagrams
\usepackage{graphicx}
\usepackage{placeins}
\usepackage{float}
\usepackage{booktabs,makecell}
\usepackage{siunitx}
\usepackage{tikz}

% Typography, colors, URLs, and hyperlinks
\usepackage{microtype}
\usepackage{xcolor}
\usepackage{url}
\usepackage{hyperref}
\usepackage{bookmark}
\usepackage{fancyhdr}
\usepackage[mathlines]{lineno}

\setlength{\headheight}{14.5pt}

\sisetup{detect-all}

\definecolor{BKorange}{HTML}{D55E00}
\definecolor{StrongBlue}{RGB}{0,130,250}
\definecolor{navylink}{RGB}{20,60,140}
\definecolor{RefBlue1}{RGB}{0,90,160}
\definecolor{RefTeal}{RGB}{0,110,130}

\hypersetup{
  colorlinks=true,
  linkcolor=RefBlue1,
  citecolor=RefBlue1,
  urlcolor=RefBlue1
}
\pdfstringdefDisableCommands{%
  \def\\{ }%
}

% Supplemental numbering

\setcounter{secnumdepth}{3}

\addtolength{\textwidth}{2.0cm}
\addtolength{\hoffset}{-1.0cm}
\addtolength{\textheight}{1.6cm}
\addtolength{\voffset}{-0.9cm}
\setlength{\footskip}{18pt}

% Small parameters
   % paraxiality (R/kappa)
           % density-floor regularizer

% Author/editor markup commands

%\newcommand{\RT}[1]{#1}

% Common mathematical notation

\renewcommand{\Im}{\operatorname{Im}}

% Short display-equation commands used throughout the notes
\newcommand{\be}{\begin{equation}}
\newcommand{\ee}{\end{equation}}

\theoremstyle{definition}

\allowdisplaybreaks

% Move footer page numbers upward to avoid clipping in PDF viewers/printers.
\makeatletter
\def\ps@plain{%
  \let\@mkboth\@gobbletwo
  \let\@oddhead\@empty
  \let\@evenhead\@empty
  \def\@oddfoot{\hfil\raisebox{12pt}{\thepage}\hfil}%
  \def\@evenfoot{\hfil\raisebox{12pt}{\thepage}\hfil}%
}
\makeatother

\begin{document}

\title{Supplementary Information for\texorpdfstring{\\}{ }
``Spin--Momentum Impedance and Filtering by a Spin-Coupled Absorbing Boundary Condition''}

\author{Alireza Jozani}
\affiliation{Departments of Physics and Mathematics, Eberhard-Karls-Universit\"at T\"ubingen,
Auf der Morgenstelle 10, 72076 Tübingen, Germany}

\date{June 24, 2026}

\maketitle
\pagestyle{fancy}
\thispagestyle{fancy}
\fancyhf{}
\fancyhead[R]{\thepage}
\renewcommand{\headrulewidth}{0pt}
\renewcommand{\footrulewidth}{0pt}

\section{Scope, notation, and relation to the main text}
\label{sec:SM_scope}

This Supplementary Information supports the main text's central claim: the spin-coupled absorbing boundary condition (spinor ABC) acts as a local two-branch spin--momentum filter. The result is not a
universal arrival-time law, but a detector-present boundary mechanism. For a
tangential Fourier wave vector \(\boldsymbol{\xi}\) at the detecting roof and detector
impedance parameter \(\kappa\), the spinor absorbing boundary has the two branches
\begin{equation}
\lambda_\pm(\boldsymbol{\xi})=i\kappa\pm|\boldsymbol{\xi}|.
\end{equation}
In a harmonic waveguide the transverse oscillator length is
\(\ell_\perp=\omega^{-1/2}\), so the typical tangential scale sampled at the roof is
\begin{equation}
|\boldsymbol{\xi}|\sim \ell_\perp^{-1}\sim\sqrt{\omega}.
\end{equation}
Therefore transverse confinement enters the detector-present timing statistics through
the local boundary symbol.

The organization is as follows. Section~\ref{sec:SM_numerics} gives the numerical model, grid scaling, and convergence checks. ~\ref{sec:SM_sweep} gives the full confinement sweep supporting Fig.~1 of the main text.~\ref{sec:SM_finite_window} investigates the finite-window bookkeeping for the restricted mean detection time statistic shown in Fig.~1(c).~\ref{sec:SM_bulk}  shows that the leading first-pass bulk flux is independent of \(\omega\). Sections~\ref{sec:SM_boundary_symbol} and~\ref{sec:SM_grid_symbol} derive and test the boundary-symbol mechanism, including the Duhamel estimate and finite-grid diagnostics.~\ref{sec:SM_return_closure} gives a reduced flux-balance and finite-guide memory closure explaining how the local boundary scale enters finite-window moments.  Sections~\ref{sec:SM_controls}--\ref{sec:SM_physical_scales} collect controls,
parameter scans, and physical scales.

The physical detector observable throughout this Supplement is the roof flux,
equivalently the norm loss of the nonunitary spinor-ABC evolution. Bohmian
trajectories, when shown as histograms, are used only as Monte Carlo samples of this
same detector-present flux law. They are not a separate no-detector arrival-time
proposal.

\section{Numerical model, grid scaling, and convergence}
\label{sec:SM_numerics}

We work in units $\hbar=m=1$ and solve the two-component time-dependent
Schrödinger equation in the finite box
\begin{equation}
        \Omega_\omega=[0,L_x(\omega)]\times[0,L_y(\omega)]\times[0,L],
\end{equation}
with
\begin{equation}
 i\partial_t\Psi
 =
 \left[
 -\frac12\Delta
 +\frac12\omega^2\bigl((x-x_c)^2+(y-y_c)^2\bigr)
 \right]\Psi,
 \qquad
 \Psi=
 \begin{pmatrix}
 \psi_\uparrow\\
 \psi_\downarrow
 \end{pmatrix}.
\end{equation}
The initial state is a normalized factorized packet,
\begin{equation}
\Psi_0(x,y,z)=\chi_\omega(x,y)\,\phi_0(z)\,\eta ,
\end{equation}
where the transverse factor is the harmonic ground-state profile, restricted and normalized in the
finite transverse box,
\begin{equation}
\chi_\omega(x,y)=\mathcal N_\perp(\omega)
\exp\!\left[-\frac{\omega}{2}\bigl((x-x_c)^2+(y-y_c)^2\bigr)\right],
\end{equation}
and the longitudinal factor is the right-moving Gaussian
\begin{equation}
\phi_0(z)=\mathcal N_z
\exp\!\left[-\frac{(z-z_c)^2}{4\sigma_\parallel^2}
+i k_z(z-z_c)\right],\qquad 0<z<L .
\end{equation}
The constants \(\mathcal N_\perp(\omega)\) and \(\mathcal N_z\) normalize the factors on their finite
numerical domains; equivalently, the full discrete state is normalized to unit norm before time
evolution. Unless stated otherwise,
\begin{equation}
\eta=
\begin{pmatrix}
\cos(\theta/2)\\ e^{i\varphi}\sin(\theta/2)
\end{pmatrix},
\qquad \theta=0,\quad \varphi=0 .
\end{equation}
In the confinement sweep only \(\omega\) is varied; the longitudinal packet, detector parameter,
initial spinor, grid prescription, and observation window are fixed as listed in Table~\ref{tab:SM_parameters}.  The lower face $z=0$ is a reflecting hard wall, implemented as a Dirichlet
boundary in the finite-difference scheme. The artificial transverse walls are
also Dirichlet. The detecting roof is
\begin{equation}
        \Sigma_L=\{z=L\},
\end{equation}
where we impose the spinor absorbing boundary condition
\begin{equation}
(\boldsymbol \sigma\cdot\boldsymbol \nabla)\Psi=i\kappa\sigma_z\Psi .
\end{equation}
For the Pauli current this boundary condition gives the outward roof flux
\begin{equation}
        j_z^P(x,y,L,t)=\kappa\,\Psi^\dagger\Psi(x,y,L,t)\ge 0.
\end{equation}
Hence the detector-present detection-time density is
\begin{equation}
        g(t;\omega)
        =
        \kappa\int_{\Sigma_L}\Psi^\dagger\Psi\,dx\,dy
        =
        -\frac{d}{dt}\|\Psi_t\|^2 .
        \label{eq:SM_roofflux}
\end{equation}
We denote the survival probability by
\begin{equation}
        S(t;\omega)=\|\Psi_t\|^2 .
\end{equation}
For a finite observation window $T_{\rm obs}$ we use
\begin{equation}
        D_{T_{\rm obs}}(\omega)
        =
        \int_0^{T_{\rm obs}}g(t;\omega)\,dt
\end{equation}
and
\begin{equation}
\mu^*(T_{\rm obs};\omega)
=\int_0^{T_{\rm obs}}S(t;\omega)\,dt
=\mathbb E[\min(\tau,T_{\rm obs})],
\label{eq:SM_RMST}
\end{equation}
where \(\tau\) is the random detector click time. The restricted mean detection time $\mu^*$ is used because for strong confinement a substantial fraction of the probability can remain undetected at the end of the finite simulation window.

The numerical evolution uses a Cartesian finite-difference Crank--Nicolson scheme with GMRES solves for the resulting non-Hermitian sparse systems. The spinor ABC is imposed by ghost-point elimination at the roof,
producing the top-layer spinor coupling associated with the tangential
derivatives in the boundary condition; this follows the implementation
described in Ref. [13] of the main text. Here we report only the present parameter choices, grid scaling, convergence checks, and diagnostics.

The transverse box is scaled with the oscillator length
\begin{equation}
        \ell_\perp=\omega^{-1/2}.
\end{equation}
Specifically,
\begin{equation}
        L_x(\omega)=L_y(\omega)=\ell_{\rm box}\ell_\perp
        =
        \frac{\ell_{\rm box}}{\sqrt{\omega}},
        \qquad
        \ell_{\rm box}=10.
        \label{eq:SM_scaledbox}
\end{equation}
With $N_x=N_y=N_\perp$, the transverse mesh width satisfies
\begin{equation}
        \frac{h_\perp}{\ell_\perp}
        =
        \frac{\ell_{\rm box}}{N_\perp}.
\end{equation}
Therefore both the wall distance in oscillator units and the transverse resolution in
oscillator units are fixed across the confinement sweep. This prevents the
observed $\omega$-dependence from being a lateral-wall or transverse-resolution
artifact.

\begin{table}[H]
\caption{Reference parameters for the confinement sweep shown in the main text and
in Fig.~\ref{fig:SM_sweep}. Only $\omega$ is varied.}
\label{tab:SM_parameters}
\begingroup
\setlength{\tabcolsep}{3.5pt}
\renewcommand{\arraystretch}{0.75}
\makebox[\linewidth][c]{%
\begin{minipage}{0.66\linewidth}
\begin{ruledtabular}
\begin{tabular}{@{}ll@{}}
Quantity & Value \\
\hline
Transverse box size & $L_x=L_y=\ell_{\rm box}/\sqrt{\omega}$, $\ell_{\rm box}=10$ \\
Longitudinal box size & $L=L_z=20$ \\
Transverse center & $x_c=L_x/2,\; y_c=L_y/2$ \\
Initial longitudinal center & $z_c=10$ \\
Detector parameter & $\kappa=\pi$ \\
Longitudinal wave number & $k_z=\pi$ \\
Longitudinal width & $\sigma_\parallel=0.5$ \\
Initial spinor & $\theta=0,\;\phi=0$, unless otherwise stated \\
Reference transverse grid & $N_x=N_y=100$ \\
Reference longitudinal grid & $N_z=1500$ \\
Reference time step & $\Delta t=2\times 10^{-4}$ \\
Observation window & $T_{\rm obs}=20$ \\
Varied parameter & $\omega$ \\
\end{tabular}
\end{ruledtabular}
\end{minipage}%
}
\endgroup
\end{table}

As a representative convergence check, we use the strongest confinement shown in
the main text, $\omega=300$. This is the most demanding point of the main sweep
because the transverse oscillator length is smallest and the delayed oscillatory
sector is largest. We independently refine the transverse grid, the longitudinal
grid, and the time step, while monitoring $D_{20}$ and $\mu^*(20)$.

\begin{table}[H]
\begingroup
\small
\setlength{\tabcolsep}{3pt}
\renewcommand{\arraystretch}{0.75}
\caption{Representative convergence checks for $\mu^*(20)$ at $\omega=300$.
The first row is the reference run used in Fig.~\ref{fig:SM_sweep}. The relative
change is
$\epsilon_{\rm rel}
=|\mu^*_{\rm ref}-\mu^*_{\rm refined}|/|\mu^*_{\rm refined}|\times100\%$.
All runs use $\kappa=k_z=\pi$, $\sigma_\parallel=0.5$, and $T_{\rm obs}=20$.}
\label{tab:SM_convergence}
\begin{ruledtabular}
\begin{tabular}{@{}lccccc@{}}
Run & $N_x=N_y$ & $N_z$ & $\Delta t$ & $D_{20}$ & $\mu^*(20)$ \\
\hline
Reference & 100 & 1500 & $2\times10^{-4}$ & 0.42 & 14.783 \\
Transverse refinement & 120 & 1500 & $2\times10^{-4}$ & 0.42 & 14.791 \\
Longitudinal refinement & 100 & 2000 & $2\times10^{-4}$ & 0.42 & 14.841 \\
Time-step refinement & 100 & 1500 & $1\times10^{-4}$ & 0.42 & 14.782 \\
\end{tabular}
\end{ruledtabular}
\endgroup
\end{table}

The largest change in $\mu^*(20)$ in Table~\ref{tab:SM_convergence} occurs under
longitudinal refinement and is below $0.4\%$. This is small compared with the
confinement-induced change over the sweep and does not affect the qualitative
conclusion: increasing $\omega$ suppresses the prompt peak, reduces the
finite-window detected fraction, and enhances the delayed detection time sector.

\section{Full confinement sweep supporting Fig.~1}
\label{sec:SM_sweep}

Here the full confinement sweep in Fig.~1 of the main text is given. Only \(\omega\) is varied. The longitudinal packet, detector parameter, initial spinor, and observation window are fixed as in Table~\ref{tab:SM_parameters}. The plotted density is the detector-present roof-flux density \(g(t;\omega)\). The red curve is the detector-free one-dimensional Gaussian comparison current through \(z=L\) for the same longitudinal packet, with the transverse factor integrated out. It is not a detector model and is not used in the fit; it is the analogue of the comparison curve used in Ref.~[13].

\begin{figure}[H]
  \centering
  % Row 1
  \begin{minipage}[t]{0.48\linewidth}
    \centering
    \includegraphics[width=\linewidth]{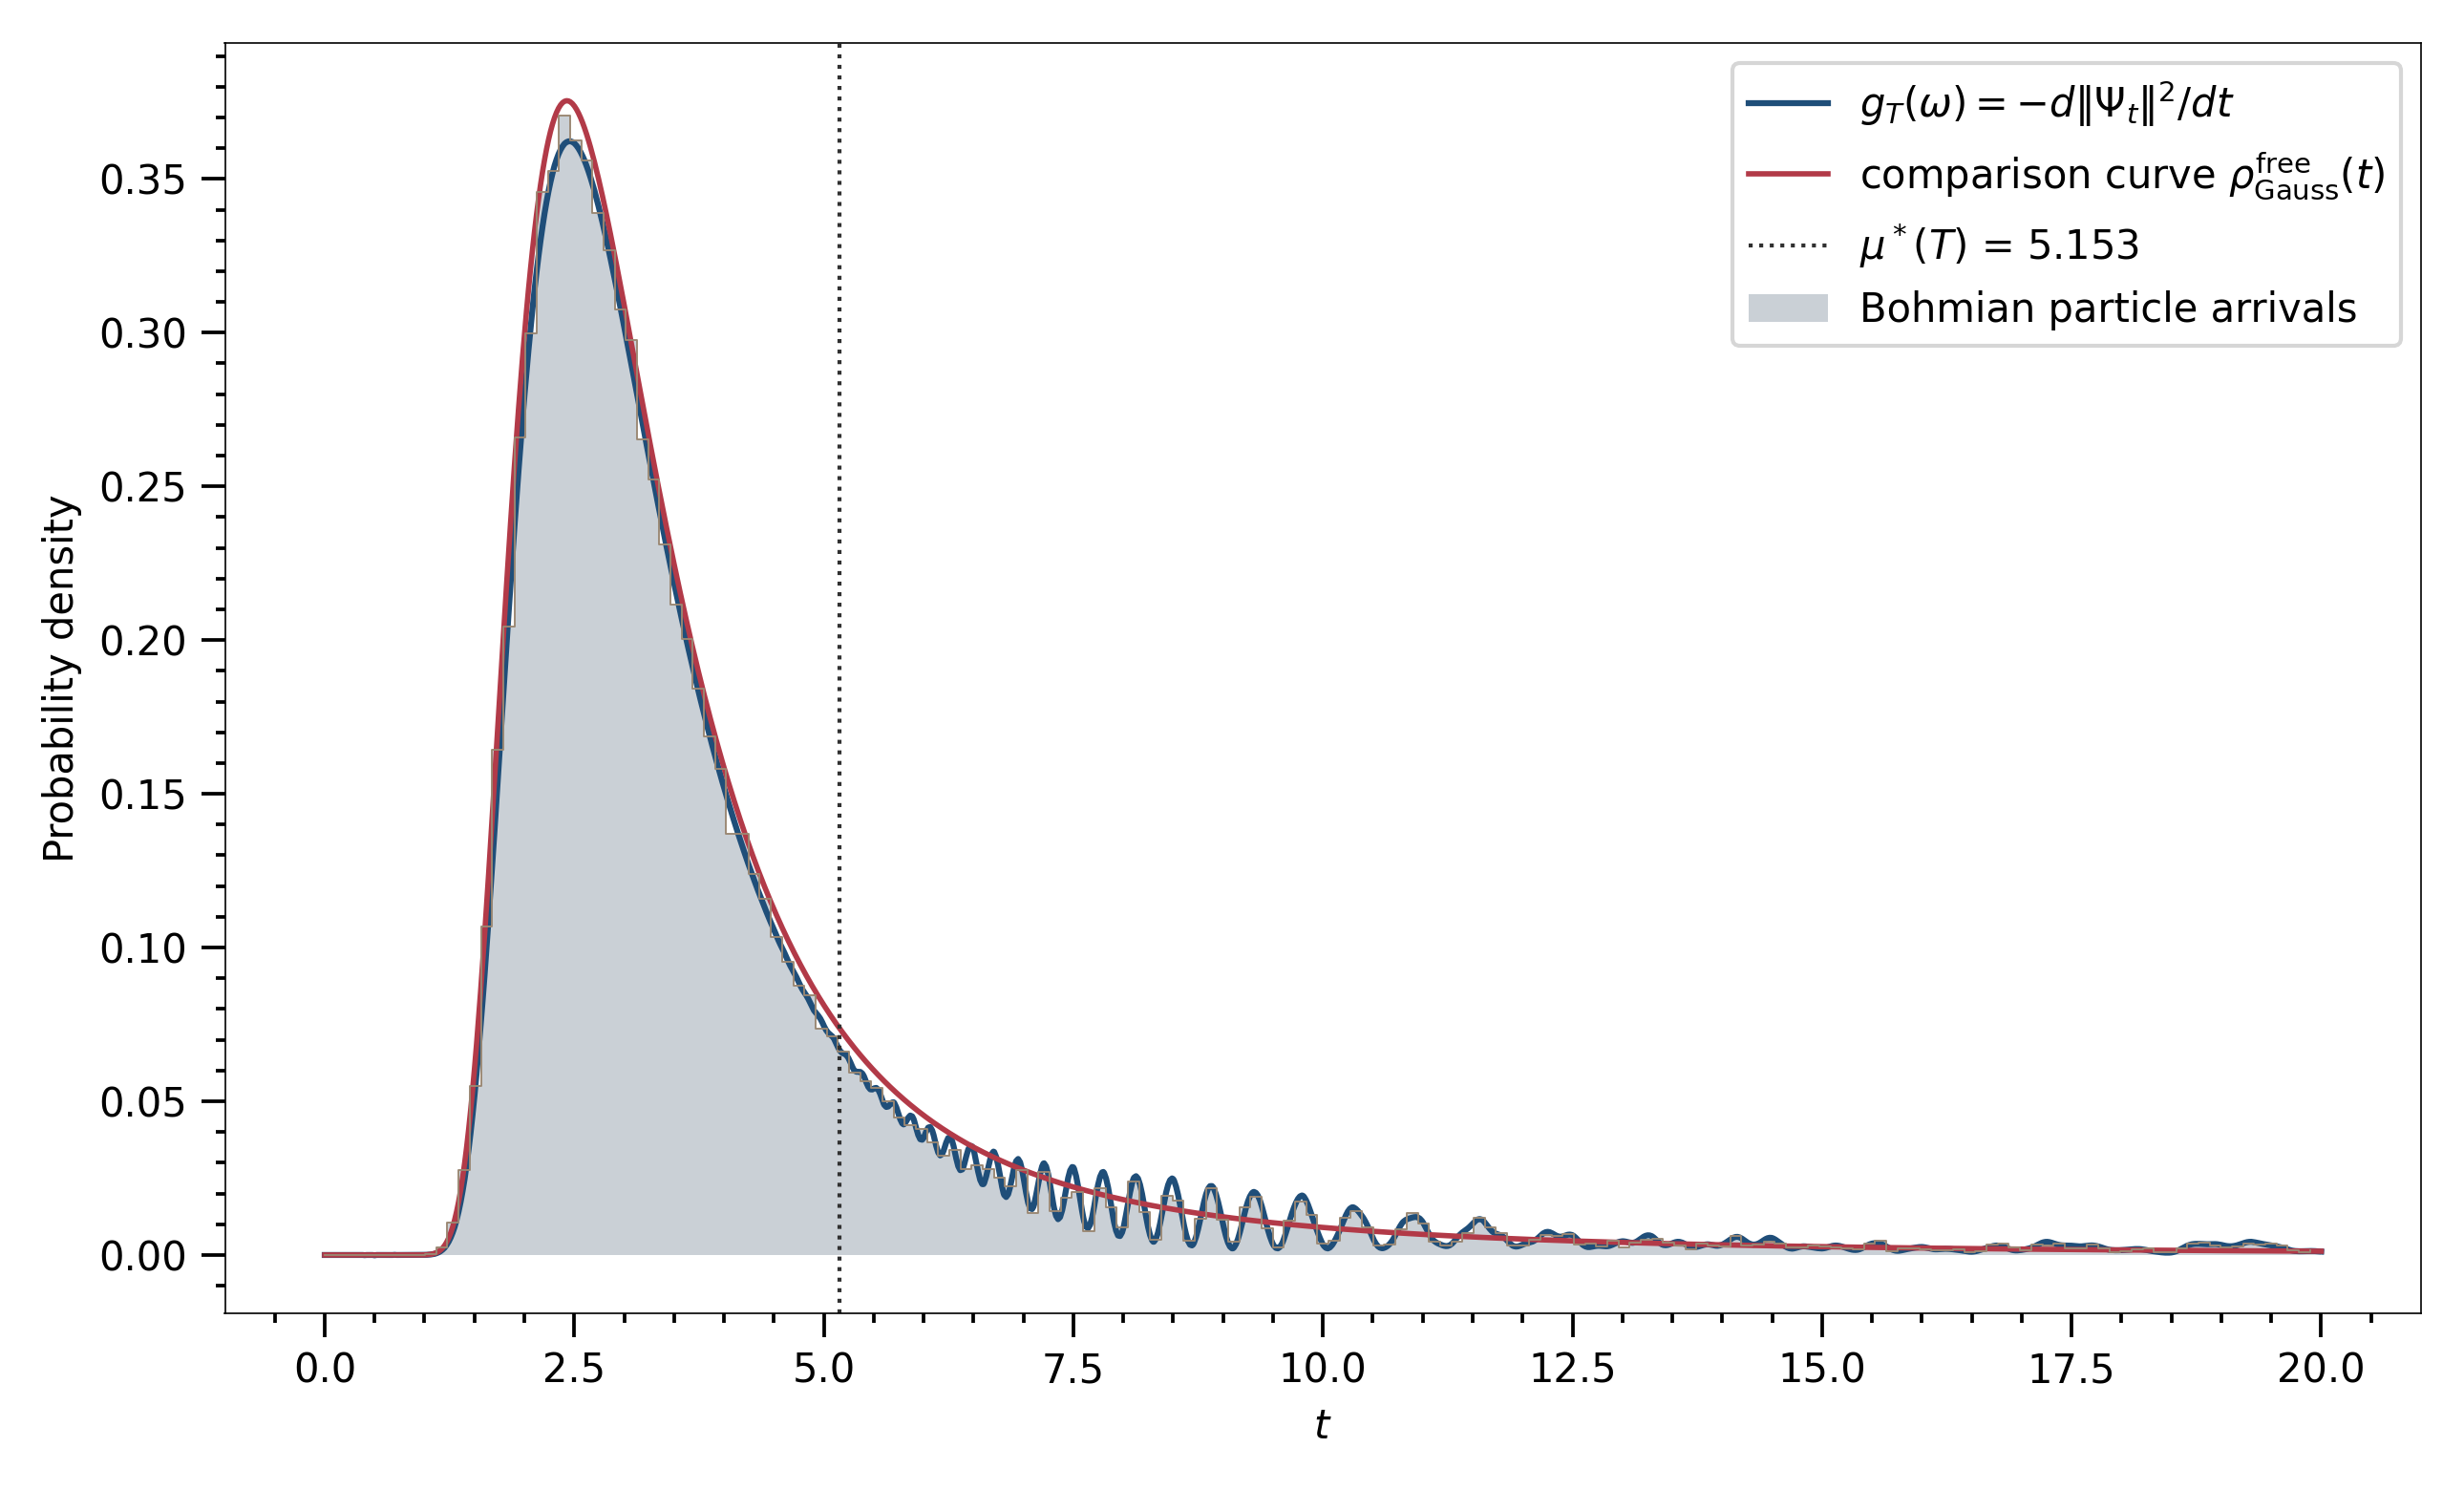}
    \par\vspace{0.3em}
    {\small (a) $\omega=1$, detection fraction = 93\%}
  \end{minipage}\hfill
  \begin{minipage}[t]{0.48\linewidth}
    \centering
    \includegraphics[width=\linewidth]{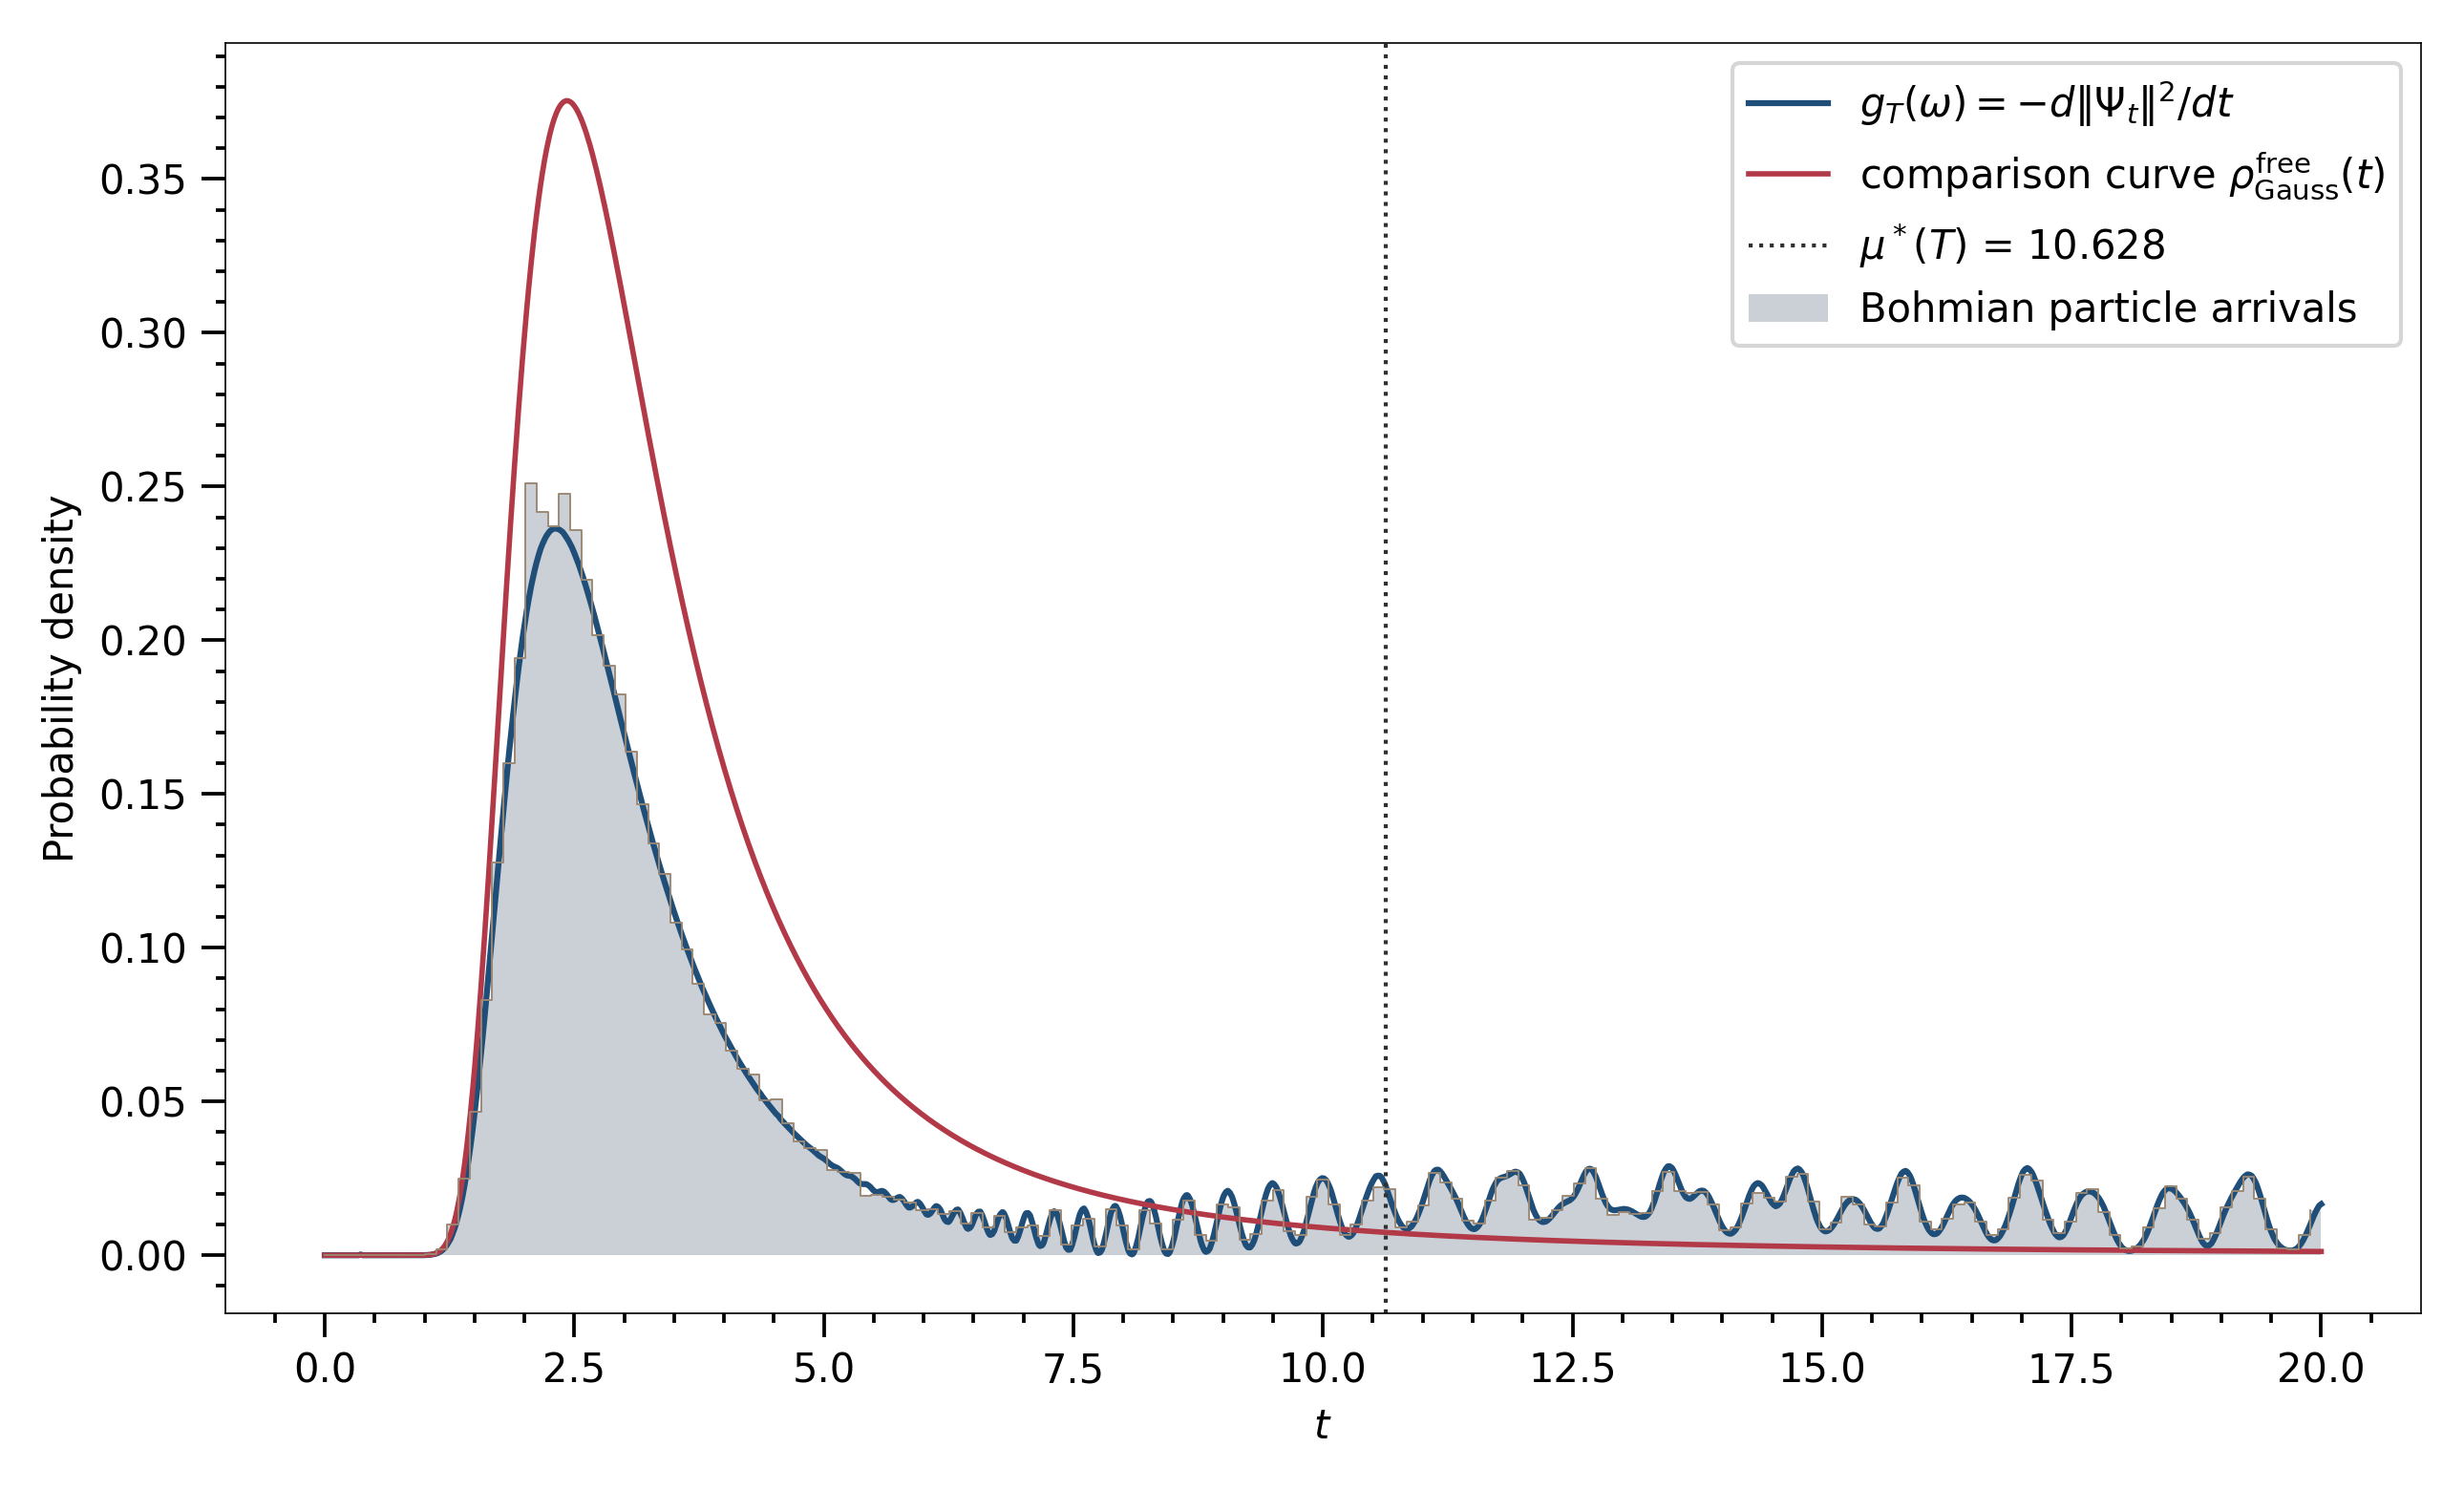}
    \par\vspace{0.3em}
    {\small (b) $\omega=100$, detection fraction = 68\%}
  \end{minipage}\hfill
  \vspace{0.8em}
  % Row 2 (single)
  \begin{minipage}[t]{0.48\linewidth}
    \centering
    \includegraphics[width=\linewidth]{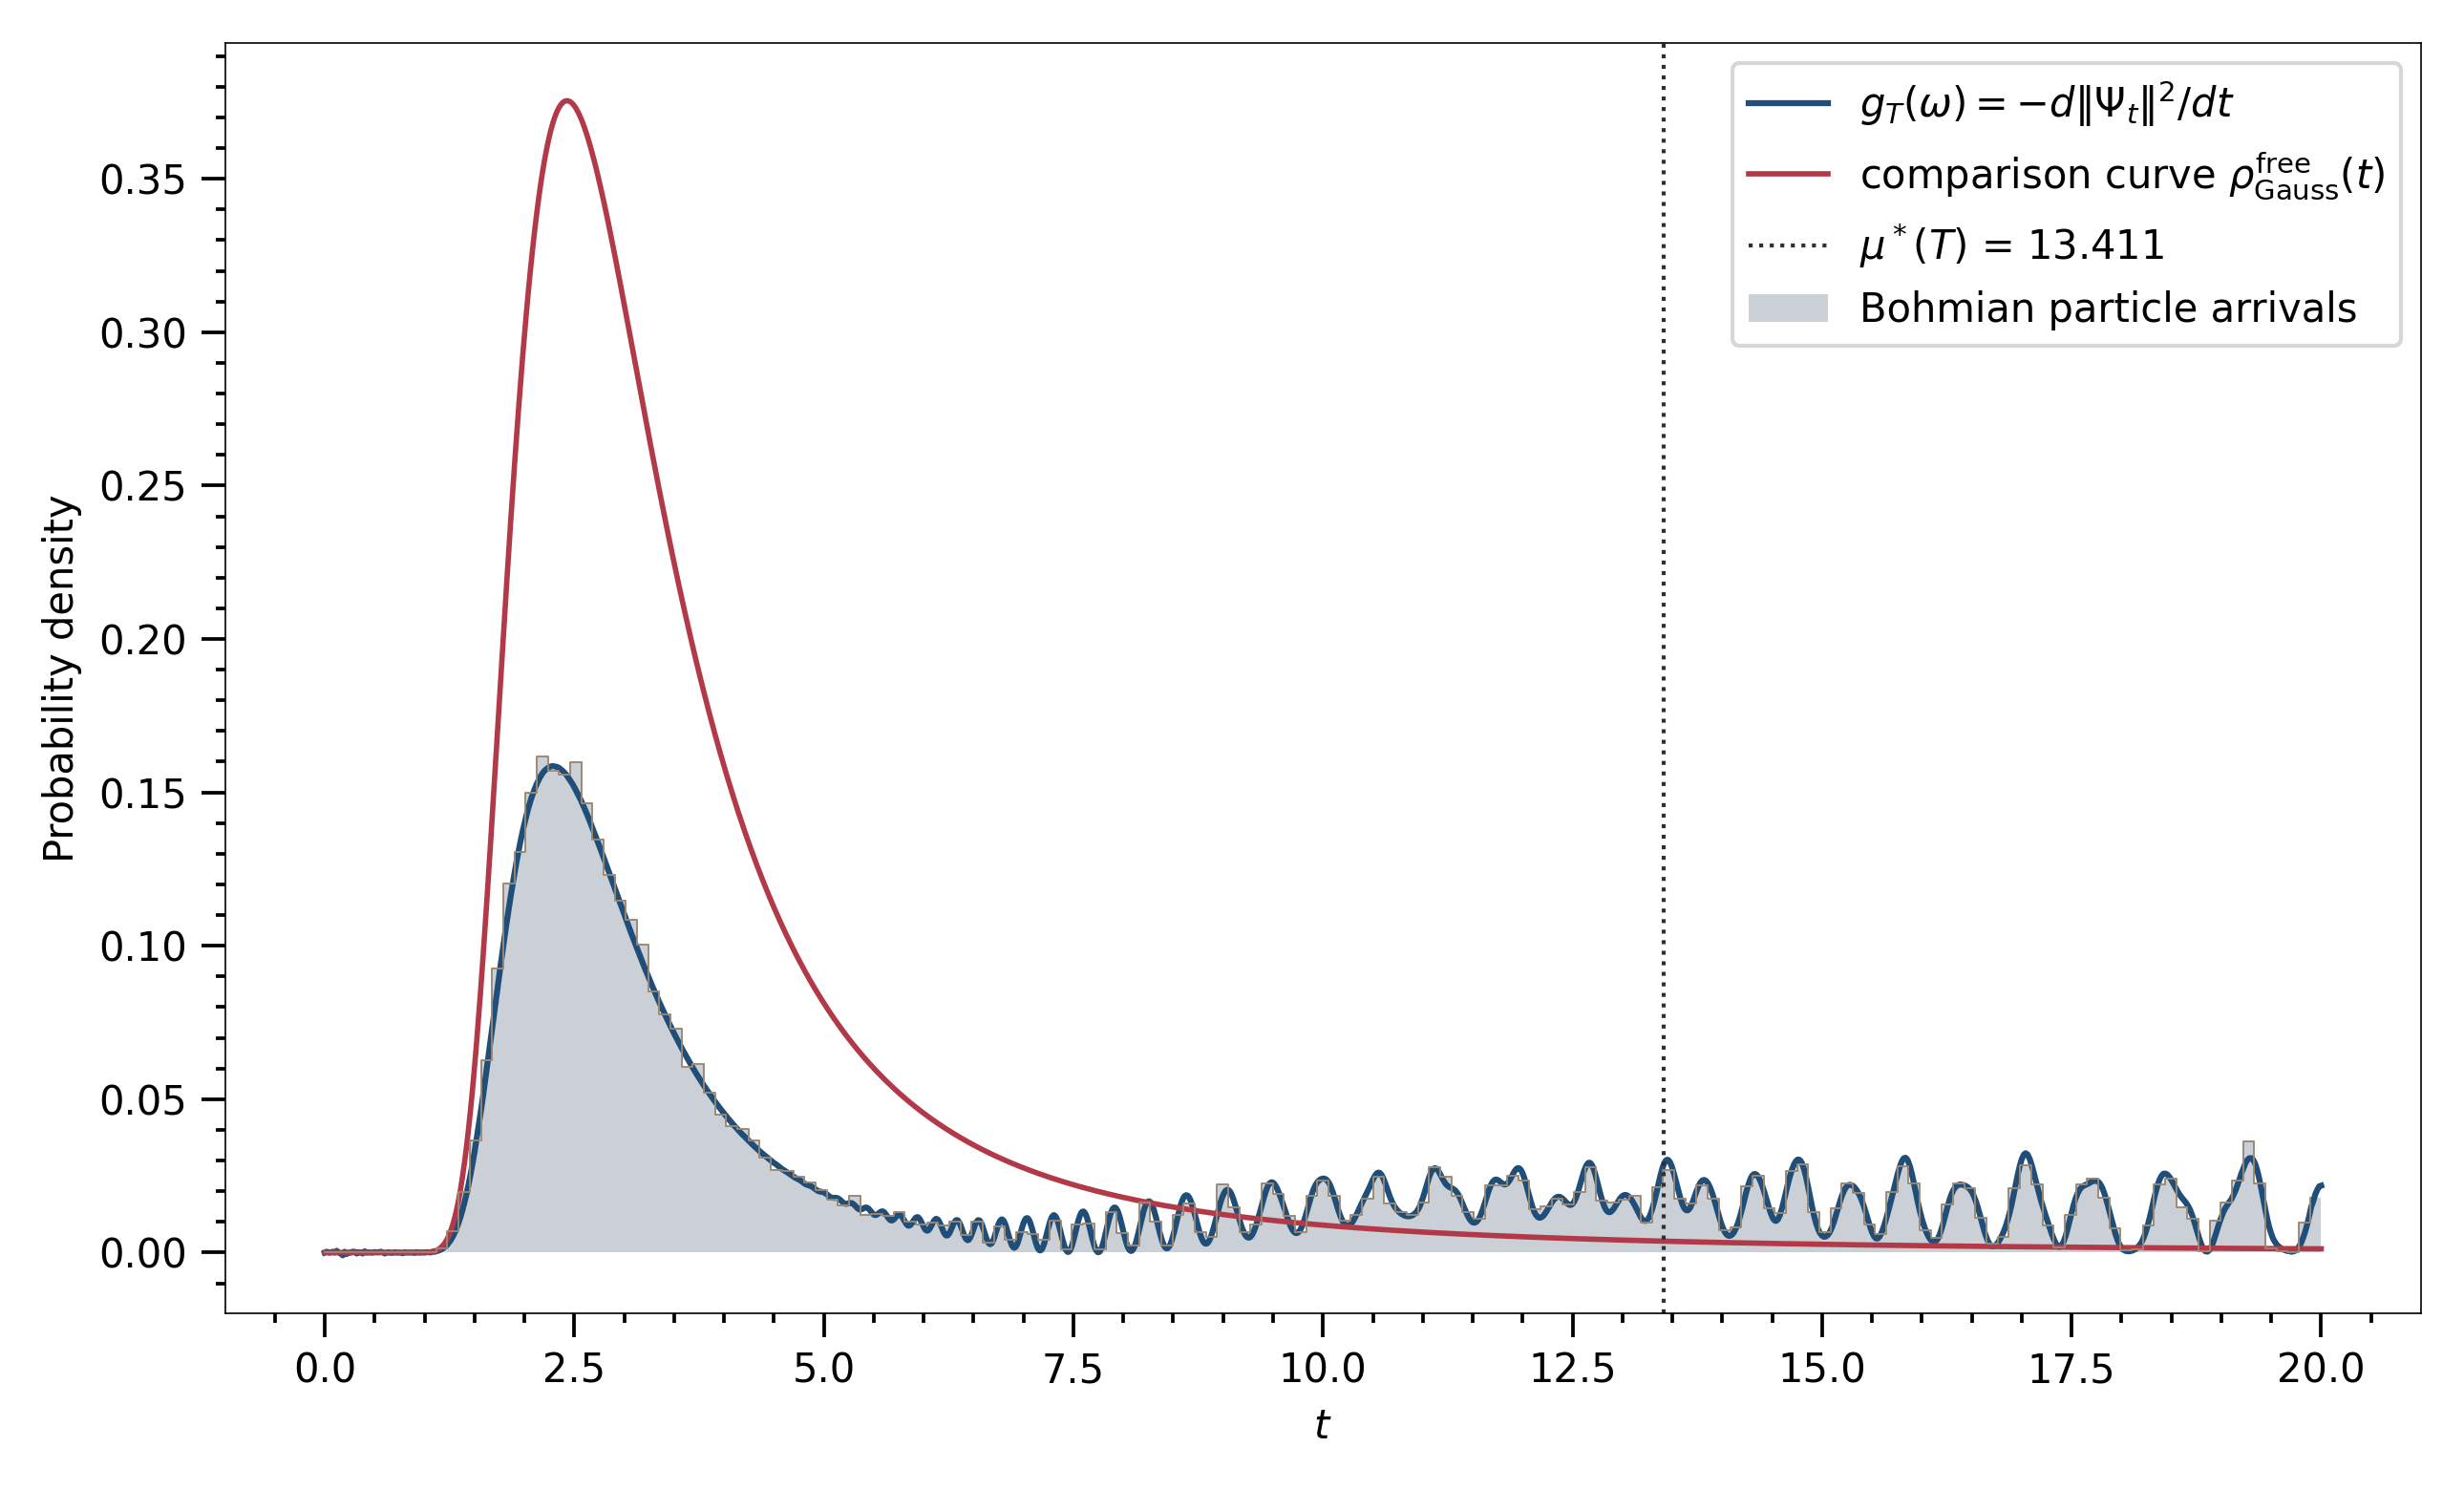}
    \par\vspace{0.3em}
    {\small (c) $\omega=200$, detection fraction = 51\%}
  \end{minipage}
  \begin{minipage}[t]{0.48\linewidth}
    \centering
    \includegraphics[width=\linewidth]{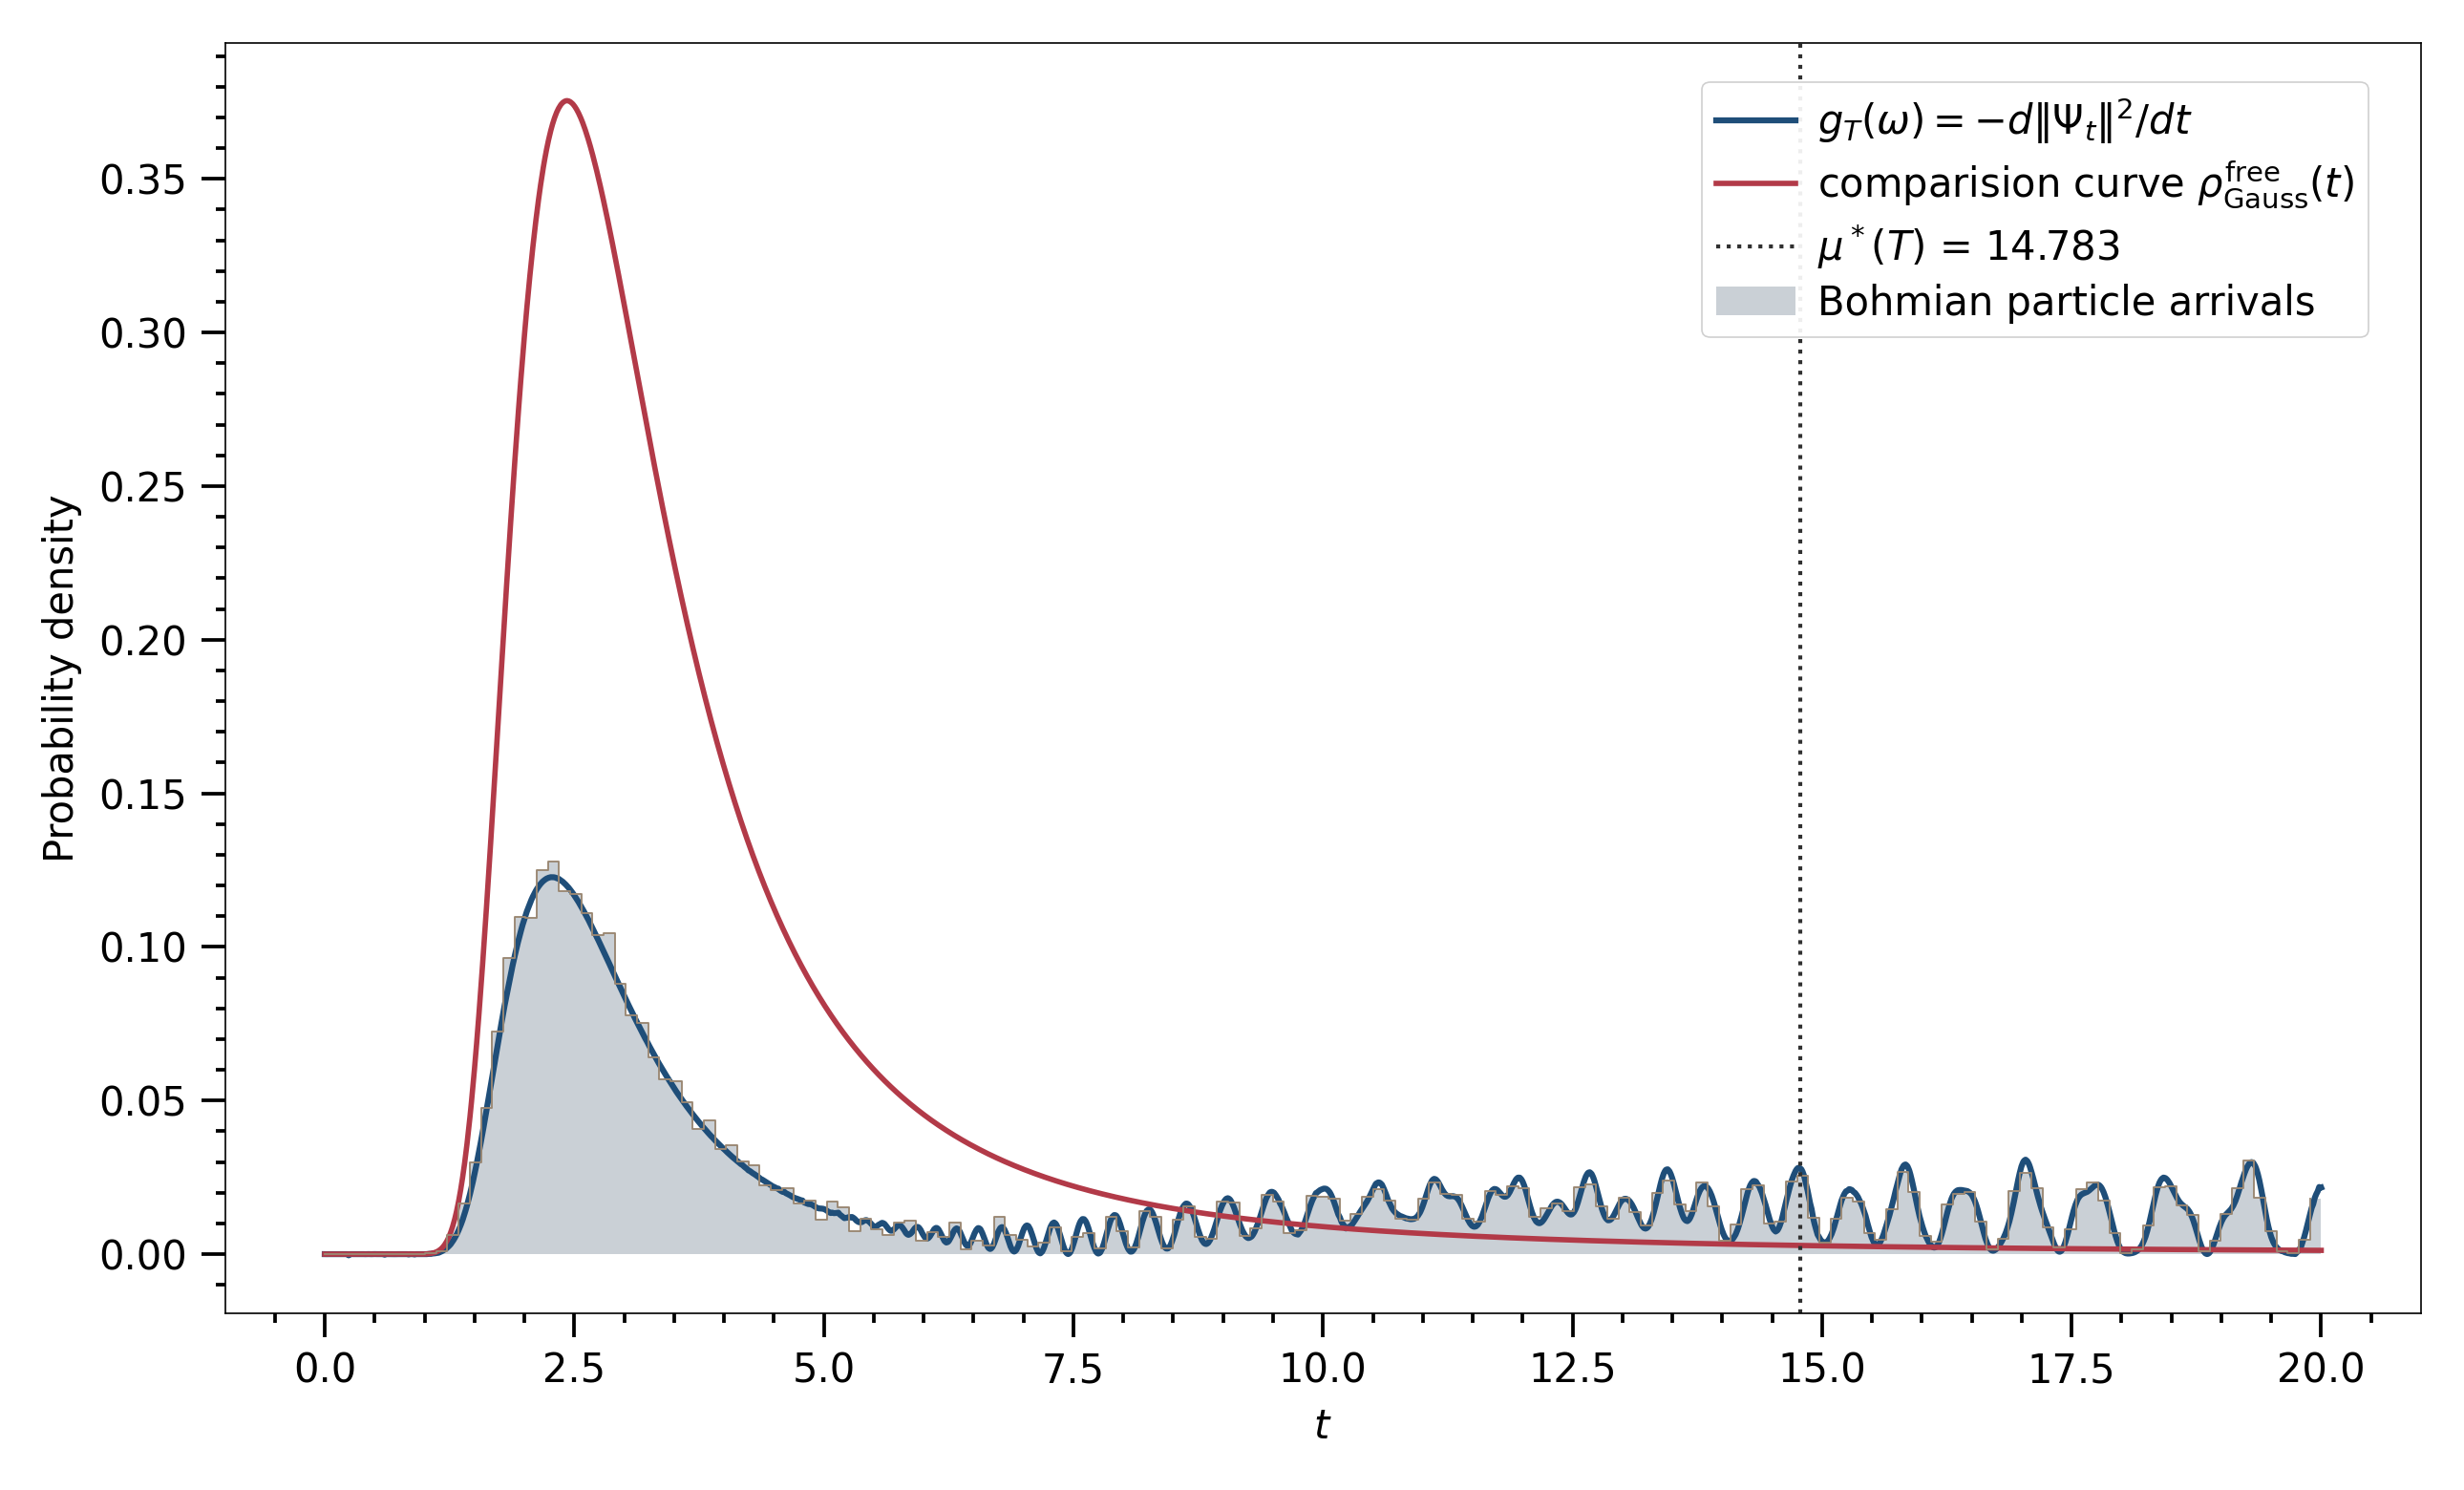}
    \par\vspace{0.3em}
    {\small (d) $\omega=300$, detection fraction = 42\%}
  \end{minipage}
\caption{
Full confinement sweep for the spinor absorbing boundary. Only \(\omega\) is
varied. Increasing \(\omega\) narrows the harmonic transverse state, suppresses
the prompt roof-flux peak, reduces the detected fraction, and shifts weight
into a delayed oscillatory sector. Blue: detector-present roof-flux density
\(g(t;\omega)\); red: detector-free Gaussian comparison current; gray:
Bohmian sampling histograms of the same detector-present flux law.}
\label{fig:SM_sweep}
\end{figure}
The finite-window mean detection time for several $\omega$ is fitted by
\begin{equation}
\mu^*(20;\omega)\simeq4.084+0.638\sqrt{\omega}.
\label{eqn:muS}
\end{equation}
This fit is empirical and finite-window dependent. The coefficients are not
universal; the robust feature is the local boundary scale
\(R=|\boldsymbol \xi|\sim\sqrt{\omega}\), derived in Sec.~\ref{sec:SM_boundary_symbol}.

\section{Finite-window bookkeeping for the statistic in Fig.~1(c)}
\label{sec:SM_finite_window}

This section gives the finite-window bookkeeping used in the main text and a
diagnostic split of the computed roof-flux signal into a prompt peak and a delayed
sector. The split is only a numerical diagnostic of the detector-present roof flux
\(g(t;\omega)\). It is not an exact microscopic decomposition of the TDSE solution
into first-pass and return amplitudes.

\subsection{Conditional finite-window density and RMDT identity}
\label{subsec:SM_RMST_identity}

Let \(T_{\rm obs}\) denote the numerical observation horizon and let \(\tau\) be the random detection time. For compactness, write \(T=T_{\rm obs}\) in this section. The detected fraction by time \(T\) is
\begin{equation}
D_T(\omega)=\mathbb{P}(\tau\leq T)
=\int_0^T g(t;\omega)\,dt .
\label{eq:SM_detected_fraction}
\end{equation}
When \(D_T(\omega)>0\), the detection-time density conditioned on detection inside
the numerical window is
\begin{equation}
        f_T(t;\omega)
        =
        \frac{g(t;\omega)}{D_T(\omega)},
        \qquad
        0\le t\le T .
        \label{eq:SM_conditional_density}
\end{equation}
Its conditional mean is
\begin{equation}
        \bar \tau_T^{\rm cond}(\omega)
        =
        \int_0^T t\, f_T(t;\omega)\,dt .
        \label{eq:SM_conditional_mean}
\end{equation}

The finite-window statistic used in the main text is the restricted mean detection time
\begin{equation}
        \mu^*(T;\omega)
        =
        \int_0^T S(t;\omega)\,dt ,
        \qquad
        S(t;\omega)=\|\Psi_t\|^2 .
        \label{eq:SM_RMST_again}
\end{equation}
Using \(g(t;\omega)=-dS(t;\omega)/dt\), integration by parts gives
\begin{equation}
\begin{aligned}
        \mu^*(T;\omega)
        &=
        T S(T;\omega)
        +
        \int_0^T t\,g(t;\omega)\,dt
        \\
        &=
        \bigl[1-D_T(\omega)\bigr]T
        +
        D_T(\omega)\,\bar \tau_T^{\rm cond}(\omega).
\end{aligned}
        \label{eq:SM_RMST_identity}
\end{equation}
Therefore \(\mu^*\) contains two finite-window effects: the conditional timing of the
detected part and the probability still undetected at the final time. Equivalently,
\begin{equation}
        \bar \tau_T^{\rm cond}(\omega)
        =
        \frac{
        \mu^*(T;\omega)-[1-D_T(\omega)]T
        }{
        D_T(\omega)
        } .
        \label{eq:SM_conditional_from_RMST}
\end{equation}
This identity is used below to keep the conditional early/late diagnostic separate
from the restricted mean detection time (RMDT) fit shown in the main text.

\subsection{Common diagnostic cutoff}
\label{subsec:SM_cutoff}
The early/late split uses one cutoff time \(t_{\rm cut}\), common to all values of
\(\omega\). The cutoff is not fitted from the roof-flux data and is not chosen
separately for each run. It is used only to define a fixed diagnostic window before
the earliest estimated contamination by a full bottom-return cycle. Let
\begin{equation}
        \Sigma_i=\{z=z_i\}
\end{equation}
be an interior monitoring plane below the detector. From the main upward-flux peak
times on two such planes, we estimate an effective axial speed \(v_{\rm est}(\omega)\).
If \(t_{\rm pk,up}^{(i)}(\omega)\) is the main upward peak time on \(\Sigma_i\), then
the estimated time of the first roof-return signal at that plane is
\begin{equation}
        t_{\rm return}^{(i)}(\omega)
        =
        t_{\rm pk,up}^{(i)}(\omega)
        +
        \frac{2d_R^{(i)}}{v_{\rm est}(\omega)},
        \qquad
        d_R^{(i)}=z_{\rm roof}-z_i .
\end{equation}
A subsequent signal from a full bottom-return cycle would require an additional
round trip from the monitoring plane to the bottom and back. We therefore define no-return time
\begin{equation}
        t_{\rm nr}^{(i)}(\omega)
        =
        t_{\rm return}^{(i)}(\omega)
        +
        \gamma
        \frac{2d_B^{(i)}}{v_{\rm est}(\omega)},
        \qquad
        d_B^{(i)}=z_i-z_{\rm bottom},
        \qquad
        \gamma=0.95 .
\end{equation}
The parameter \(\gamma\) is not a reflection coefficient and is not used to model
the dynamics. It only gives a conservative timing estimate for the diagnostic split. For the closer monitoring plane \(\Sigma_1\), the estimated no-return times are
\begin{equation}
\begin{array}{c|cccccc}
\omega & 1 & 50 & 100 & 150 & 200 & 300\\
\hline
t_{\rm nr}^{(1)}(\omega)
& 13.58 & 7.55 & 6.02 & 5.69 & 4.46 & 3.69 .
\end{array}
\end{equation}
The smallest value is about \(3.69\). We therefore use the common cutoff
\begin{equation}
        t_{\rm cut}=3.6 .
        \label{eq:SM_tcut}
\end{equation}

\subsection{Early/late identity and numerical values}
\label{subsec:SM_early_late}

Define the early and late intervals
\begin{equation}
        I_E=\{0\le t\le t_{\rm cut}\},
        \qquad
        I_L=\{t_{\rm cut}<t\le T\}.
\end{equation}
The late conditional weight is
\begin{equation}
        w_L(\omega)
        =
        \int_{t_{\rm cut}}^T f_T(t;\omega)\,dt,
        \qquad
        w_E(\omega)=1-w_L(\omega).
\end{equation}
The early and late conditional means are
\begin{equation}
        t_E(\omega)
        =
        \frac{1}{w_E(\omega)}
        \int_0^{t_{\rm cut}} t\, f_T(t;\omega)\,dt ,
\end{equation}
and
\begin{equation}
        t_L(\omega)
        =
        \frac{1}{w_L(\omega)}
        \int_{t_{\rm cut}}^T t\, f_T(t;\omega)\,dt .
\end{equation}
Then the conditional finite-window mean detection satisfies the exact identity
\begin{equation}
\begin{aligned}
        \bar \tau_T^{\rm cond}(\omega)
        &=
        w_E(\omega)t_E(\omega)+w_L(\omega)t_L(\omega)
        \\
        &=
        t_E(\omega)
        +
        w_L(\omega)\bigl[t_L(\omega)-t_E(\omega)\bigr].
\end{aligned}
        \label{eq:SM_conditional_early_late}
\end{equation}
We then define the delayed-sector contribution to the conditional mean by
\begin{equation}
        \Delta t_L^{\rm cond}(\omega)
        :=
        \bar \tau_T^{\rm cond}(\omega)-t_E(\omega)
        =
        w_L(\omega)\bigl[t_L(\omega)-t_E(\omega)\bigr].
        \label{eq:SM_delta_late}
\end{equation}

\begin{table}[H]
\caption{Early/late split of the finite-window detector statistics for
\(T=20\) and \(t_{\rm cut}=3.6\). Here \(D_T\) is the detected fraction,
\(\bar\tau_T^{\rm cond}\) is the mean conditioned on detection before \(T\),
and \(w_L,t_L,\Delta t_L^{\rm cond}\) are computed with respect to the
conditional density \(f_T\).}
\label{tab:SM_early_late}
\begingroup
\small
\setlength{\tabcolsep}{2.5pt}
\renewcommand{\arraystretch}{0.75}
\makebox[\linewidth][c]{%
\begin{minipage}{0.72\linewidth}
\begin{ruledtabular}
\begin{tabular}{@{}rccccccc@{}}
\(\omega\) &
\(D_T\) &
\(\bar\tau_T^{\rm cond}\) &
\(\mu^*(T)\) &
\(t_E\) &
\(w_L\) &
\(t_L\) &
\(\Delta t_L^{\rm cond}\) \\
\hline
1   & 0.925 & 3.95 & 5.15  & 2.59 & 0.37 & 6.18  & 1.35 \\
50  & 0.788 & 5.00 & 8.18  & 2.54 & 0.39 & 8.77  & 2.46 \\
100 & 0.670 & 6.00 & 10.62 & 2.51 & 0.45 & 10.18 & 3.48 \\
150 & 0.577 & 6.63 & 12.29 & 2.51 & 0.49 & 10.82 & 4.12 \\
200 & 0.507 & 7.01 & 13.41 & 2.50 & 0.52 & 11.17 & 4.51 \\
300 & 0.416 & 7.45 & 14.78 & 2.49 & 0.54 & 11.55 & 4.95 \\
\end{tabular}
\end{ruledtabular}
\end{minipage}%
}
\endgroup
\end{table}
Fitting the displayed diagnostic quantities as affine functions of
\(\sqrt{\omega}\) gives
\begin{align}
        t_E(\omega)
        &\approx
        2.52\pm0.04 ,
        \\
        \Delta t_L^{\rm cond}(\omega)
        &\approx
        (1.07\pm0.18)+(0.234\pm0.015)\sqrt{\omega},
        \\
        \bar\tau_T^{\rm cond}(\omega)
        &\approx
        (3.66\pm0.18)+(0.228\pm0.015)\sqrt{\omega},
        \\
        \mu^*(T;\omega)
        &\approx
        (4.38\pm0.36)+(0.618\pm0.031)\sqrt{\omega}. 
        \label{eqn:mu}
\end{align}
The fit in Eq.~\eqref{eqn:mu} uses the rounded diagnostic values displayed in Table~\ref{tab:SM_early_late}, whereas Eq.~\eqref{eqn:muS} above and Fig. 1(c) of the main text use the unrounded full confinement-sweep data.

The near constancy of \(t_E\) should not be read as the absence of a
first-encounter boundary effect. The spinor ABC already reads the
transverse scale during the first near-roof interaction, through the local
boundary scale \(R=|\boldsymbol{\xi}|\sim\sqrt{\omega}\). What is nearly
constant is only the conditional mean time of those detections that remain in
the early window.

The stronger prompt-sector signature is instead the loss of early detected
weight. Defining
\begin{equation}
D_E(\omega):=D_T(\omega)\,[1-w_L(\omega)],
\end{equation}
the data give \(D_E(1)\simeq 0.58\) and \(D_E(300)\simeq 0.19\). Thus increasing
\(\omega\) strongly suppresses the prompt roof-flux contribution, even though
the mean time \(t_E\) of the remaining prompt detections changes only weakly.
The delayed sector should therefore be understood as the finite-box continuation
and magnification, in time moments, of the same spinor-ABC boundary filtering
already imposed at the first detector encounter.

Thus, the early conditional mean changes only weakly over the scan and does not
carry the dominant square-root trend. The delayed conditional contribution
grows approximately affinely in \(\sqrt{\omega}\) over this finite window.
The RMDT trend, however, must not be identified directly with
\(\Delta t_L^{\rm cond}\). Combining Eqs.~\eqref{eq:SM_RMST_identity} and
\eqref{eq:SM_delta_late} gives
\begin{equation}
\mu^*(T;\omega)
=
D_T(\omega)
\bigl[
t_E(\omega)+\Delta t_L^{\rm cond}(\omega)
\bigr]
+
\bigl[1-D_T(\omega)\bigr]T .
\end{equation}
Therefore, the fitted coefficient of the RMDT receives contributions from the
weak residual variation of \(t_E(\omega)\), the growth of
\(\Delta t_L^{\rm cond}(\omega)\), and the decreasing detected fraction
\(D_T(\omega)\) through the survival term \(\bigl[1-D_T(\omega)\bigr]T\).
The late sector is not a separate physical mechanism. It is the finite-box
delayed continuation of the same spinor-ABC boundary-filtering mechanism
derived in Sec.~\ref{sec:SM_boundary_symbol} and represented effectively by the reduced flux-balance closure in Sec.~\ref{sec:SM_return_closure}.

\section{First-pass bulk independence of \texorpdfstring{\(\omega\)}{omega}}
\label{sec:SM_bulk}

We begin with an analytic bulk check. Before the packet has significantly touched the absorbing roof, ordinary first-pass propagation cannot generate the observed confinement dependence on $\omega$. In a separable, spin-independent bulk, changing \(\omega\) only changes the normalized transverse factor; after cross-section integration, the leading Pauli flux is purely longitudinal and independent of \(\omega\). 

We now show this explicitly. Let \(z_b=L-\delta\) be an interior counting plane below the detector, and let
\begin{equation}
        \Sigma_b=\{(x,y,z):z=z_b\}.
\end{equation}
In the region below the roof, assume the first-pass separable bulk Hamiltonian
\begin{equation}
        H_{\rm bulk}=H_{xy}(\omega)+H_z ,
\end{equation}
with
\begin{equation}
        H_{xy}(\omega)
        =
        -\frac12(\partial_x^2+\partial_y^2)+V_{xy}(x,y;\omega),
        \qquad
        H_z=-\frac12\partial_z^2 .
\end{equation}
We also assume that the absorbing roof has not yet significantly modified the state at the interior plane.  For a prepared state with spatially constant spinor \(\eta\), the auxiliary first-pass bulk field is
\begin{equation}
\Psi_{\rm fp}(x,y,z,t)
=
\chi_\omega(x,y,t)\,\phi_{\rm fp}(z,t)\,\eta,
\qquad
\rho_{\rm fp}=|\Psi_{\rm fp}|^2
=
|\chi_\omega(x,y,t)|^2|\phi_{\rm fp}(z,t)|^2 .
\label{eq:SM_separable_bulk}
\end{equation}
Here ``first-pass'' means the separable, spin-independent bulk evolution before appreciable feedback
from the absorbing roof. The longitudinal factor is initialized by $
\phi_{\rm fp}(z,0)=\phi_0(z),$ and \(\Psi_{\rm fp}\) is not the full spinor-ABC solution. It is used only to test whether ordinary bulk propagation can generate the observed \(\omega\)-dependence. The spin density of this auxiliary field is
\begin{equation}
\boldsymbol S_{\rm fp}
=
\Psi_{\rm fp}^\dagger\boldsymbol \sigma\Psi_{\rm fp}
=
\rho_{\rm fp}\boldsymbol s_\eta,
\qquad
\boldsymbol s_\eta=\eta^\dagger\boldsymbol \sigma\eta .
\end{equation}
The corresponding Pauli current is
\begin{equation}
\boldsymbol j^P_{\rm fp}
=
\boldsymbol j^{\rm conv}_{\rm fp}
+
\frac12\boldsymbol\nabla\times \boldsymbol S_{\rm fp},
\qquad
\boldsymbol j^{\rm conv}_{\rm fp}
=
\operatorname{Im}(\Psi_{\rm fp}^\dagger\boldsymbol \nabla\Psi_{\rm fp}) .
\end{equation}
Since \(\boldsymbol s_{\eta}\) is constant in the first-pass separable approximation,
\begin{equation}
        (\boldsymbol \nabla\times\boldsymbol S_{\rm fp})_z
        =
        \partial_x(\rho_{\rm fp} s_{\rm \eta, y})-\partial_y(\rho_{\rm fp} s_{\rm \eta, x}).
\end{equation}
Therefore
\begin{equation}
\int_{\Sigma_b}
\boldsymbol (\boldsymbol \nabla\times\boldsymbol S_{\rm fp})_z\,dx\,dy
=\int_{\partial\Sigma_b}
\bigl(\boldsymbol S_{{\rm fp},y}\nu_x-\boldsymbol S_{{\rm fp},x}\nu_y\bigr)\,d\ell
=0,
\end{equation}
where \(\boldsymbol\nu=(\nu_x,\nu_y)\) is the outward unit normal to \(\partial\Sigma_b\) in the transverse plane. The last equality follows from the lateral boundary conditions in the finite box,
or from transverse decay in the ideal waveguide. Hence the plane-integrated Pauli
flux equals the plane-integrated convective flux:
\begin{equation}
        \int_{\Sigma_b}j_{\rm fp,z}^P\,dx\,dy
        =
        \int_{\Sigma_b}j_{\rm fp,z}^{\rm conv}\,dx\,dy .
        \label{eq:SM_pauli_convective_plane}
\end{equation}
Define the first-pass bulk flux through \(\Sigma_b\) by
\begin{equation}
        \Phi_{\rm bulk}(t)
        =
        \int_{\Sigma_b}j_{\rm fp,z}^P(\boldsymbol  r,t)\,dA .
\end{equation}
Using Eq.~\eqref{eq:SM_separable_bulk},
\begin{equation}
\begin{aligned}
        \Phi_{\rm bulk}(t)
        &=
        \int_{\Sigma_b}
        \Im(\Psi_{\rm fp}^\dagger\partial_z\Psi_{\rm fp})\,dA
        \\
        &=
        \left(
        \int |\chi_\omega(x,y,t)|^2\,dx\,dy
        \right)
        \Im\bigl(\phi_{\rm fp}^*\partial_z\phi_{\rm fp}\bigr)(z_b,t).
\end{aligned}
\end{equation}
Since \(H_{xy}(\omega)\) is self-adjoint with the chosen transverse boundary
conditions, the transverse factor remains normalized. Therefore
\begin{equation}
        \Phi_{\rm bulk}(t)
        =
        \Im\bigl(\phi_{\rm fp}^*\partial_z\phi_{\rm fp}\bigr)(z_b,t),
        \label{eq:SM_bulk_flux_independent}
\end{equation}
which is independent of \(\omega\) and independent of the detector parameter \(\kappa\). Accordingly, the first-pass flux-averaged crossing time
\begin{equation}
        \bar\tau_{\rm bulk}
        =
        \frac{\int_0^\infty t\,\Phi_{\rm bulk}(t)\,dt}
        {\int_0^\infty \Phi_{\rm bulk}(t)\,dt}
\end{equation}
is \(\omega\)-independent under the stated assumptions. This does not claim that
the full finite-box detector signal is \(\omega\)-independent. It only shows that
the leading first-pass bulk transport does not generate the confinement trend;
the effect must enter through the spinor absorbing boundary.

\section{Boundary-symbol mechanism}
\label{sec:SM_boundary_symbol}

This section studies the detailed boundary-symbol calculation used in the main text.
The calculation is a local probe of the spinor ABC, not a second
absorber and not a physical layer below the detector. The physical detector
observable remains the roof flux at \(z=L\). At the roof the spinor ABC is
\begin{equation}
        (\boldsymbol\sigma\cdot\boldsymbol \nabla)\Psi=i\kappa\boldsymbol \sigma_z\Psi,
        \qquad
        \Psi=
        \begin{pmatrix}
        \psi_\uparrow\\
        \psi_\downarrow
        \end{pmatrix}.
        \label{eq:SM_spinor_ABC}
\end{equation}
In components,
\begin{equation}
\begin{aligned}
        \partial_z\psi_\uparrow
        &=
        i\kappa\psi_\uparrow
        -
        (\partial_x-i\partial_y)\psi_\downarrow,\\
        \partial_z\psi_\downarrow
        &=
        i\kappa\psi_\downarrow
        +
        (\partial_x+i\partial_y)\psi_\uparrow .
\end{aligned}
        \label{eq:SM_spinor_ABC_components}
\end{equation}
Equivalently, the roof condition is the first-order normal boundary relation
\begin{equation}
        \partial_z\Psi\big|_{z=L}
        =
        \mathcal C\Psi\big|_{z=L},
        \qquad
        \mathcal C=
        \begin{pmatrix}
        i\kappa & -D_-\\
        D_+ & i\kappa
        \end{pmatrix},
        \qquad
        D_\pm=\partial_x\pm i\partial_y .
        \label{eq:SM_C_operator}
\end{equation}
Therefore the detector does not impose only a scalar normal impedance. It couples the
normal boundary relation to tangential derivatives of the roof trace.

\subsection{Exact near-roof identity}
\label{subsec:SM_exact_near_roof_identity}

We now isolate the local normal response generated by the boundary relation itself.
Fix a time \(t\) and take the roof trace \(\Psi(\cdot,L,t)\) as given. We use the
homogeneous relation \(\partial_z\Psi=\mathcal C\Psi\) only to continue this trace a small
auxiliary distance inward, to \(z=L-\epsilon\) with \(\epsilon>0\). This continuation
is a local probe of the boundary symbol, not a physical detector layer; the true
TDSE solution need not satisfy \(\partial_z\Psi=\mathcal C\Psi\) away from the roof. Define the boundary-condition defect/error in a small interval \(L-\delta<z\le L\) by
\begin{equation}
        \mathcal E_{\rm bc}(z,t)
        :=
        \partial_z\Psi(\cdot,z,t)-\mathcal C\Psi(\cdot,z,t).
        \label{eq:SM_Ebc_def}
\end{equation}
The spinor ABC implies
\begin{equation}
        \mathcal E_{\rm bc}(L,t)=0 .
        \label{eq:SM_Ebc_zero}
\end{equation}
After tangential Fourier transform, each mode satisfies
\begin{equation}
        \partial_z\widehat\Psi(\boldsymbol\xi,z,t)
        =
        \mathcal C(\boldsymbol\xi)\widehat\Psi(\boldsymbol\xi,z,t)
        +
        \widehat{\mathcal E}_{\rm bc}(\boldsymbol\xi,z,t).
        \label{eq:SM_mode_normal_ode}
\end{equation}
Variation of constants, integrated backward from \(L\) to \(z\), gives the exact
near-roof identity
\begin{equation}
        \widehat\Psi(\boldsymbol\xi,z,t)
        =
        e^{(z-L)\mathcal C(\boldsymbol\xi)}
        \widehat\Psi(\boldsymbol\xi,L,t)\\
        -
        \int_z^L
        e^{(z-s)\mathcal C(\boldsymbol\xi)}
        \widehat{\mathcal E}_{\rm bc}(\boldsymbol\xi,s,t)\,ds.
        \label{eq:SM_Duhamel_identity}
\end{equation}
The first term is the homogeneous normal continuation generated by the spinor ABC.
The second term is the Duhamel remainder. We denote the roof trace by
\begin{equation}
        W_\omega(\boldsymbol\xi,t)
        :=
        \widehat\Psi_\omega(\boldsymbol\xi,L,t).
        \label{eq:SM_roof_trace}
\end{equation}
For \(z=L-\epsilon\), the Duhamel remainder is
\begin{equation}
        \widehat{\mathcal E}_{\rm Duh}
        (\boldsymbol\xi,L-\epsilon,t)
        :=
        -
        \int_0^\epsilon
        e^{-(\epsilon-u)\mathcal C(\boldsymbol\xi)}
        \widehat{\mathcal E}_{\rm bc}(\boldsymbol\xi,L-u,t)\,du .
        \label{eq:SM_Duhamel_remainder}
\end{equation}
This is the same remainder term denoted by \(\widehat{\mathcal R}_{\rm Duh}\) in the main text. Under the regularity assumption quantified in Sec.~\ref{subsec:SM_Duhamel_estimate},
this remainder is \(O(\epsilon^2)\) modewise as \(\epsilon\to0\). Hence it has no
zeroth- or first-order contribution at the roof. The leading inward normal response
is therefore determined by the homogeneous boundary symbol.

\subsection{Tangential symbol and spin--momentum branches}
\label{subsec:SM_symbol_branches}

The tangential Fourier transform is used only to expose the local symbol of the
boundary operator. In the finite-difference calculation, the analogous object is the
discrete tangential symbol used in Sec.~\ref{sec:SM_grid_symbol}. For a tangential
Fourier mode
\begin{equation}
        \boldsymbol\xi=(\xi_x,\xi_y),
        \qquad
        \xi_\pm=\xi_x\pm i\xi_y,
\end{equation}
Eq.~\eqref{eq:SM_C_operator} gives
\begin{equation}
        \mathcal C(\boldsymbol\xi)
        =
        \begin{pmatrix}
        i\kappa & -i\xi_-\\
        i\xi_+ & i\kappa
        \end{pmatrix}.
        \label{eq:SM_C_symbol}
\end{equation}
Separate the scalar impedance from the tangential spin coupling:
\begin{equation}
        \mathcal J(\boldsymbol\xi)
        :=
        \mathcal C(\boldsymbol\xi)-i\kappa I .
        \label{eq:SM_J_def}
\end{equation}
Then
\begin{equation}
        \mathcal J(\boldsymbol\xi)
        =
        (\hat{\boldsymbol z}\times\boldsymbol\xi)\cdot\boldsymbol\sigma
        =
        -\xi_y\sigma_x+\xi_x\sigma_y,
        \qquad
        \mathcal J(\boldsymbol\xi)^2=R^2I,
        \qquad
        R=|\boldsymbol\xi|.
        \label{eq:SM_J_symbol}
\end{equation}
For \(R>0\), define
\begin{equation}
        \Gamma(\boldsymbol\xi)
        =
        \frac{\mathcal J(\boldsymbol\xi)}{R}
        =
        (\hat{\boldsymbol z}\times\hat{\boldsymbol\xi})\cdot\boldsymbol\sigma,
        \qquad
        \Gamma(\boldsymbol\xi)^2=I .
        \label{eq:SM_Gamma_def}
\end{equation}

The zero mode \(R=0\) is degenerate and carries no \(R\Gamma\) contribution; it is
understood by continuity. Therefore
\begin{equation}
        \mathcal C(\boldsymbol\xi)
        =
        i\kappa I+R\Gamma(\boldsymbol\xi).
        \label{eq:SM_C_branch_form}
\end{equation}
The two boundary eigenbranches are
\begin{equation}
        \lambda_\pm(\boldsymbol\xi)=i\kappa\pm R,
        \label{eq:SM_branch_eigenvalues}
\end{equation}
with projectors
\begin{equation}
        \Pi_\pm(\boldsymbol\xi)
        =
        \frac12\bigl(I\pm\Gamma(\boldsymbol\xi)\bigr).
        \label{eq:SM_projectors}
\end{equation}
The projectors select two tangential spin--momentum branches, with in-plane spin
direction perpendicular to the tangential momentum. This is the key local difference
between the spinor ABC and a scalar absorbing boundary.

\subsection{Auxiliary normal response}
\label{subsec:SM_auxiliary_normal_response}
Since \(\Gamma^2=I\), the homogeneous exponential in
Eq.~\eqref{eq:SM_Duhamel_identity} is explicit:
\begin{equation}
\begin{aligned}
        e^{-\epsilon\mathcal C(\boldsymbol\xi)}
        &=
        e^{-i\kappa\epsilon}
        e^{-\epsilon R\Gamma(\boldsymbol\xi)}\\
        &=
        e^{-i\kappa\epsilon}
        \left[
        e^{-R\epsilon}\Pi_+(\boldsymbol\xi)
        +
        e^{R\epsilon}\Pi_-(\boldsymbol\xi)
        \right].
\end{aligned}
        \label{eq:SM_expC}
\end{equation}
Putting \(z=L-\epsilon\) in Eq.~\eqref{eq:SM_Duhamel_identity} gives
\begin{equation}
        \widehat\Psi_\omega(\boldsymbol\xi,L-\epsilon,t)
        =
        e^{-i\kappa\epsilon}
        B_{\rm br}(\epsilon,\boldsymbol\xi)W_\omega(\boldsymbol\xi,t)
        +
        \widehat{\mathcal R}_{\rm Duh}
        (\boldsymbol\xi,L-\epsilon,t),
        \label{eq:SM_near_roof_response}
\end{equation}
where the two-branch normal-response map is
\begin{equation}
        B_{\rm br}(\epsilon,\boldsymbol\xi)
        =
        e^{-R\epsilon}\Pi_+(\boldsymbol\xi)
        +
        e^{R\epsilon}\Pi_-(\boldsymbol\xi).
        \label{eq:SM_BR_def}
\end{equation}
This is the matrix-valued branch filter acting on spinor amplitudes. The factor \(e^{-R\epsilon}\Pi_+\) is the boundary-induced evanescent normal
factor, with length scale \(R^{-1}\), and the term \(e^{R\epsilon}\Pi_-\) is the
companion branch of the same auxiliary inward continuation. It is not physical
amplification, not an absorbed component, and not a second detector model. Using Eq.~\eqref{eq:SM_projectors},
\begin{equation}
B_{\rm br}(\epsilon,\boldsymbol\xi)
=
\cosh(R\epsilon)I-\sinh(R\epsilon)\Gamma(\boldsymbol\xi)
=
e^{-R\epsilon\Gamma(\boldsymbol\xi)} .
\end{equation}
Thus the branch structure is not visible as a multiplicative suppression of the
roof density itself, since \(B_{\rm br}(0,\boldsymbol \xi)=I\). It enters through the first inward
normal response:
\begin{equation}
\partial_\epsilon B_{\rm br}(\epsilon,\boldsymbol\xi)|_{\epsilon=0}
=
-R\Gamma(\boldsymbol\xi)
=
-\mathcal J(\boldsymbol\xi).
\end{equation}
This is the local sense in which the spinor ABC filters tangential spin--momentum: the same tangential radius \(R=|\boldsymbol\xi|\) that labels the roof mode sets the scale of the first normal response at the boundary.

For the harmonic transverse ground state, $\ell_\perp=\omega^{-1/2},$ so the typical tangential wave number sampled by the roof trace satisfies\footnote{Equivalently, for normalized transverse oscillator modes centered at
the trap center, $
D_\pm\chi_{00}^{(\omega)} = -\sqrt{\omega}\,\chi_\pm^{(\omega)},\quad
\chi_\pm^{(\omega)} = \frac{\chi_{10}^{(\omega)}\pm i\chi_{01}^{(\omega)}}{\sqrt2},$ up to phase conventions. This is the oscillator-basis version of the
same boundary-symbol scale \(R=|\boldsymbol \xi|\sim\sqrt{\omega}\).}
\begin{equation}
R=|\boldsymbol\xi|\sim \ell_\perp^{-1}\sim \sqrt{\omega}.
\end{equation}

A complementary local stationary viewpoint gives the same branch
structure. If one freezes a tangential branch satisfying
\(\Pi_\pm\Psi=\Psi\), the roof condition reduces to
\begin{equation}
\partial_z\psi_\pm=(i\kappa\pm R)\psi_\pm .
\end{equation}
Therefore even the local no-click matching problem is governed by the
non-scalar pair \(i\kappa\pm R\), not by a single scalar Robin
impedance. In a frozen half-space plane-wave check this corresponds to
a matrix no-click reflection amplitude of the form
\begin{equation}
 \operatorname{Ref}_{\rm loc}(k_n,\boldsymbol\xi)
=
r_+(k_n,R)\Pi_+(\boldsymbol \xi)
+
r_-(k_n,R)\Pi_-(\boldsymbol \xi),
\end{equation}
where \(k_n>0\) is the normal wave number. In that frozen local model
the two branch intensities are equal, but the branch phases and
projectors remain different. We do not use this stationary viewpoint
as a fit model or as a scattering theory of the finite guide. The full
phase-resolved scattering problem, including oscillator-channel
evanescent components, is separate from the finite-window roof-flux
mechanism studied here. \footnote{The author thanks Roderich Tumulka for discussions on
stationary scattering viewpoints and evanescent boundary responses.}

\subsection{Covariance form of the local boundary source}
\label{subsec:SM_covariance_source}

The previous subsection identifies the local boundary scale. We now express its
first-order effect on a normalized auxiliary time moment in covariance form. This
auxiliary moment is only a diagnostic of the local boundary response; the physical
detector statistic remains the roof flux at \(z=L\).

Since the scalar phase \(e^{-i\kappa\epsilon}\) drops out of densities, the relevant
first-order density response is obtained after removing this phase. By
Eq.~\eqref{eq:SM_near_roof_response} and the Duhamel estimate of
Sec.~\ref{subsec:SM_Duhamel_estimate},
\begin{equation}
e^{i\kappa\epsilon}\widehat\Psi_\omega(\boldsymbol\xi,L-\epsilon,t)
=
B_{\rm br}(\epsilon,\boldsymbol\xi)W_\omega(\boldsymbol\xi,t)
+
O_{\rm Duh}(\epsilon^2).
\end{equation}
Thus the exact phase-removed trace and the homogeneous branch probe have the same
zeroth and first inward variations at the roof. We therefore define
\begin{equation}
\widetilde W_{\omega,\epsilon}(\boldsymbol\xi,t)
:=
B_{\rm br}(\epsilon,\boldsymbol\xi)W_\omega(\boldsymbol\xi,t),
\end{equation}
and compute the first normal variation from this homogeneous branch probe. We keep
the branch exponential exact, rather than replacing it by a finite-depth Taylor
approximation. Since \(B_{\rm br}(\epsilon,\boldsymbol\xi)=e^{-\epsilon R\Gamma(\boldsymbol\xi)}\)
and \(\Gamma(\boldsymbol\xi)\) is Hermitian with \(\Gamma^2=I\), we have
\begin{equation}
B_{\rm br}(\epsilon,\boldsymbol\xi)^\dagger
B_{\rm br}(\epsilon,\boldsymbol\xi)
=
e^{-2\epsilon R\Gamma(\boldsymbol\xi)}
=
\cosh(2R\epsilon)I-\sinh(2R\epsilon)\Gamma(\boldsymbol\xi).
\end{equation}
Therefore the auxiliary homogeneous boundary-layer spectral density is exactly
\begin{equation}
\rho^{\rm bl}_{\omega,\epsilon}(\boldsymbol\xi,t)
:=
\left|\widetilde W_{\omega,\epsilon}(\boldsymbol\xi,t)\right|^2
=
W_\omega^\dagger e^{-2\epsilon R\Gamma(\boldsymbol\xi)}W_\omega .
\end{equation}
On the null set where \(W_\omega^\dagger W_\omega=0\), \(a_\omega\) may be defined arbitrarily, e.g. \(a_\omega=0\). Writing
\begin{equation}
\rho^{\rm bl}_{\omega,0}(\boldsymbol\xi,t)=W_\omega^\dagger W_\omega, \quad\text{and}  \qquad  a_\omega(\boldsymbol\xi,t)
:=
-2\frac{W_\omega^\dagger\Gamma(\boldsymbol\xi)W_\omega}
        {W_\omega^\dagger W_\omega},
\end{equation}
we obtain the exact reweighting form
\begin{equation}
\rho^{\rm bl}_{\omega,\epsilon}(\boldsymbol\xi,t)
=
\rho^{\rm bl}_{\omega,0}(\boldsymbol\xi,t)\,
b_{\omega,\epsilon}(\boldsymbol\xi,t),
\end{equation}
where
\begin{equation}
b_{\omega,\epsilon}(\boldsymbol\xi,t)
=
\cosh(2R\epsilon)
+
\frac{a_\omega(\boldsymbol\xi,t)}{2}\sinh(2R\epsilon).
\label{eq:SM_Filter2}
\end{equation}
The quantity \(a_\omega\) is real because \(\Gamma\) is Hermitian. Since the eigenvalues of \(\Gamma\) are \(\pm1\),
\begin{equation}
|a_\omega(\boldsymbol\xi,t)|\le 2.
\end{equation}
In particular,
\begin{equation}
b_{\omega,0}=1,
\qquad
\left.\partial_\epsilon b_{\omega,\epsilon}\right|_{\epsilon=0}
=
R a_\omega(\boldsymbol\xi,t).
\label{eq:SM_filterAt0}
\end{equation}
No finite-depth smallness assumption \(R\epsilon\ll1\) is used here: the branch map has been kept exact, and only its derivative at the physical roof is taken. We now pass from this pointwise density reweighting to a normalized auxiliary time moment. Let
\begin{equation}
d\mu^{(0)}_\omega(\boldsymbol\xi,t)
:=
\rho^{\rm bl}_{\omega,0}(\boldsymbol\xi,t)\,d^2\boldsymbol\xi\,dt,
\qquad
Z^{(0)}_\omega
:=
\int d\mu^{(0)}_\omega ,
\end{equation}
where the time integral is over the chosen finite observation window. Define the
normalized roof-trace measure
\begin{equation}
d\nu^{(0)}_\omega
:=
\frac{d\mu^{(0)}_\omega}{Z^{(0)}_\omega}.
\end{equation}
The branch-reweighted auxiliary measure at depth \(\epsilon\) is
\begin{equation}
d\mu^{\rm bl}_{\omega,\epsilon}
=
\rho^{\rm bl}_{\omega,\epsilon}(\boldsymbol\xi,t)\,d^2\xi\,dt
=
b_{\omega,\epsilon}(\boldsymbol\xi,t)\,d\mu^{(0)}_\omega .
\end{equation}
After normalization,
\begin{equation}
d\nu^{\rm bl}_{\omega,\epsilon}
=
\frac{d\mu^{\rm bl}_{\omega,\epsilon}}
     {\int d\mu^{\rm bl}_{\omega,\epsilon}}
=
\frac{b_{\omega,\epsilon}(\boldsymbol\xi,t)}
     {\mathbb E_{\nu^{(0)}_\omega}[b_{\omega,\epsilon}]}
\,d\nu^{(0)}_\omega .
\end{equation}
This identity is exact for the homogeneous branch probe. Now for any finite-window observable \(F(\boldsymbol\xi,t)\), its expectation with respect to this
auxiliary measure is therefore
\begin{equation}
\mathbb E_{\nu^{\rm bl}_{\omega,\epsilon}}[F]
=
\frac{\mathbb E_{\nu^{(0)}_\omega}[F\,b_{\omega,\epsilon}]}
     {\mathbb E_{\nu^{(0)}_\omega}[b_{\omega,\epsilon}]}.
\label{eq:SM_TimeMoment}     
\end{equation}
Differentiating Eq.~\eqref{eq:SM_TimeMoment} at \(\epsilon=0\), and using Eq.~\eqref{eq:SM_filterAt0}
gives
\begin{equation}
\left.
\partial_\epsilon
\mathbb E_{\nu^{\rm bl}_{\omega,\epsilon}}[F]
\right|_{\epsilon=0}
=
\mathbb E_{\nu^{(0)}_\omega}[F\,R a_\omega]
-
\mathbb E_{\nu^{(0)}_\omega}[F]\,
\mathbb E_{\nu^{(0)}_\omega}[R a_\omega].
\end{equation}
Thus
\begin{equation}
\left.
\partial_\epsilon
\mathbb E_{\nu^{\rm bl}_{\omega,\epsilon}}[F]
\right|_{\epsilon=0}
=
\operatorname{Cov}_{\nu^{(0)}_\omega}
\!\left(F,R a_\omega\right).
\end{equation}
Taking \(F=t\) to calculate the normalized first time moment, the local first-order boundary-response coefficient is
\begin{equation}
\Lambda_\omega
:=
\left.
\partial_\epsilon
\bar t_{\rm bl}(\omega,\epsilon)
\right|_{\epsilon=0},
\qquad
\bar t_{\rm bl}(\omega,\epsilon)
:=
\mathbb E_{\nu^{\rm bl}_{\omega,\epsilon}}[t],
\end{equation}
and therefore
\begin{equation}
\Lambda_\omega
=
\operatorname{Cov}_{\nu^{(0)}_\omega}
\!\left(t,R a_\omega\right).
\end{equation}
This is the desired covariance form of the local boundary response. The derivation used
the exact branch exponential through \(b_{\omega,\epsilon}\), and the only derivative taken
was the derivative at the physical roof, \(\epsilon=0\).  For the harmonic transverse family we write
\begin{equation}
R=\sqrt{\omega}\,s,
\end{equation}
where \(s\) is the dimensionless tangential radius in oscillator units. Hence
\begin{equation}
\Lambda_\omega
=
\sqrt{\omega}\,
\operatorname{Cov}_{\nu^{(0)}_\omega}
\!\left(t,s a_\omega\right)
=
\sqrt{\omega}\,\beta^{\rm bl}_\omega,
\label{eq:SM_source2}
\end{equation}
with
\begin{equation}
\beta^{\rm bl}_\omega
:=
\operatorname{Cov}_{\nu^{(0)}_\omega}
\!\left(t,s a_\omega\right).
\end{equation}
Since \(|a_\omega|\le 2\) and \(0\le t\le T\) on the finite observation window, Cauchy--Schwarz gives, for example,
\begin{equation}
|\beta_\omega^{\rm bl}|
\le
2T\,
\sqrt{\mathbb E_{\nu_\omega^{(0)}}[s^2]} .
\end{equation}
Thus \(\beta_\omega^{\rm bl}\) remains bounded whenever the scaled tangential moment \(\mathbb E_{\nu_\omega^{(0)}}[s^2]\) remains order one, as checked numerically in Sec.~\ref{sec:SM_grid_symbol}.

We emphasize that \(\bar t_{\rm bl}(\omega,\epsilon)\) is not an observable
detection time at \(z=L-\epsilon\); all physical detection statistics are defined by
the roof flux at \(z=L\). The auxiliary boundary-response calculation only extracts
the local source in Eq.~\ref{eq:SM_source2}. In the full finite guide, this local filtering affects the
roof statistics through the first near-roof interaction and through undetected,
branch-reweighted components that leave the near-roof region and later return, as
represented by the reduced flux closure in Sec.~\ref{sec:SM_return_closure}.

\section{Finite-grid boundary-symbol diagnostic and Duhamel estimate}
\label{sec:SM_grid_symbol}

This section gives the discrete diagnostic corresponding to
Sec.~\ref{sec:SM_boundary_symbol}. The physical detector statistic is always the
roof flux at \(z=L\). The auxiliary depth
\begin{equation}
        \epsilon_g=h_z =\dfrac{L}{N_z}
\end{equation}

is used only as a one-grid normal probe of the spinor-ABC boundary response. It is not a physical detector thickness. At each diagnostic time we use the stored roof trace
\begin{equation}
        W_\omega(\boldsymbol\xi,t)
        =
        \widehat\Psi(\boldsymbol\xi,L,t).
\end{equation}
To match the central finite-difference tangential derivatives used in the solver, the continuum tangential variable is replaced by the discrete symbol
\begin{equation}
        \boldsymbol\xi_h(k)
        =
        \left(
        \frac{\sin(k_xh_x)}{h_x},
        \frac{\sin(k_yh_y)}{h_y}
        \right),
        \qquad
        R_h=|\boldsymbol\xi_h|,
        \qquad
        s=\frac{R_h}{\sqrt{\omega}} .
        \label{eq:SM_discrete_symbol}
\end{equation}
Because the transverse walls are Dirichlet, this symbol is used as a local stencil diagnostic for the central-difference tangential derivative, not as an exact diagonalization of the full finite transverse operator.  The discrete spinor generator \(\mathcal J_h\) is obtained from
Eq.~\eqref{eq:SM_J_symbol} by replacing \(\boldsymbol\xi\) with
\(\boldsymbol\xi_h\), so that \(\mathcal J_h^2=R_h^2I\). For \(R_h>0\), define
\begin{equation}
        \widehat{\mathcal J}_h=\frac{\mathcal J_h}{R_h}.
\end{equation}
The local spinor factor is
\begin{equation}
        a_\omega(\boldsymbol\xi,t)
        =
        -2\,
        \frac{
        W_\omega^\dagger
        \widehat{\mathcal J}_h
        W_\omega
        }{
        W_\omega^\dagger W_\omega
        },
        \qquad
        |a_\omega|\le2 .
        \label{eq:SM_discrete_a}
\end{equation}
All averages are taken with respect to the normalized roof-trace measure
\begin{equation}
        \mathbb E_{\nu_\omega^{(0)}}[F]
        =
        \frac{
        \int_0^T
        \sum_{\boldsymbol\xi}
        \|W_\omega(\boldsymbol\xi,t)\|^2
        F(\boldsymbol\xi,t)\,dt
        }{
        \int_0^T
        \sum_{\boldsymbol\xi}
        \|W_\omega(\boldsymbol\xi,t)\|^2\,dt
        } .
        \label{eq:SM_discrete_average}
\end{equation}
We compute
\begin{equation}
        \beta_\omega^{\rm bl}
        =
        \operatorname{Cov}_{\nu_\omega^{(0)}}(t,sa_\omega),
        \qquad
        \Lambda_\omega
        =
        \operatorname{Cov}_{\nu_\omega^{(0)}}(t,R_h a_\omega)
        =
        \sqrt{\omega}\,\beta_\omega^{\rm bl}.
        \label{eq:SM_discrete_Lambda}
\end{equation}
We also monitor the one-grid finite-depth probe scale
\begin{equation}
        q_\omega
        =
        \mathbb E_{\nu_\omega^{(0)}}[(\epsilon_gR_h)^2]
        =
        (\epsilon_g\sqrt{\omega})^2
        \mathbb E_{\nu_\omega^{(0)}}[s^2].
        \label{eq:SM_qomega}
\end{equation}
The quantity \(q_\omega\) is not used in the derivation of
the covariance formula in Sec.~\ref{subsec:SM_covariance_source}. It is only a dimensionless finite-depth diagnostic for the one-grid probe \(\epsilon_g=h_z\):
small \(q_\omega\) means that the sampled modes have \(\epsilon_g R_h\) small on average. It is not an error estimate. The actual one-grid continuation defect is monitored separately by \(\mathcal E_{2{\rm br}}\).  As a global consistency check, we record the detector-budget mismatch
\begin{equation}
        \Delta_{\rm bud}^{\rm rel}
        =
        \left|
        \frac{
        \int_0^T J_L(t)\,dt
        -
        \bigl(\|\Psi_0\|^2-\|\Psi_T\|^2\bigr)
        }{
        \|\Psi_0\|^2-\|\Psi_T\|^2
        }
        \right|.
        \label{eq:SM_budget_mismatch}
\end{equation}
Finally, we compare the true trace one grid spacing below the roof with the
homogeneous two-branch continuation from the roof trace:
\begin{equation}
        W_{\rm hom}(\boldsymbol\xi,t;h_z)
        =
        e^{-i\kappa h_z}
        e^{-h_z\mathcal J_h(\boldsymbol\xi)}
        W_\omega(\boldsymbol\xi,t),
        \qquad
        W_{\rm in}(\boldsymbol\xi,t)
        =
        \widehat\Psi(\boldsymbol\xi,L-h_z,t).
\end{equation}
The one-grid continuation defect is
\begin{equation}
\begin{aligned}
\mathcal E_{2\mathrm{br}}(h_z)
=
\left\langle
\frac{
\left\|W_{\mathrm{in}}(\cdot,t)
      -W_{\mathrm{hom}}(\cdot,t;h_z)\right\|_{\ell^2_{\boldsymbol{\xi}}}
}{
\left\|W_{\mathrm{in}}(\cdot,t)\right\|_{\ell^2_{\boldsymbol{\xi}}}
}
\right\rangle_{\mathrm{act}} .
\end{aligned}
\label{eq:SM_two_branch_defect}
\end{equation}
Here \(\langle\cdot\rangle_{\rm act}\) denotes an active-flux-weighted average
over times for which the roof signal is appreciable.

\begin{table}[H]
\caption{Representative one-grid diagnostics for the spinor-ABC boundary
response. Here \(\epsilon_g=h_z\), \(R_h=|\boldsymbol\xi_h|\),
\(s=R_h/\sqrt{\omega}\), and \(q_\omega=\mathbb E[(\epsilon_gR_h)^2]\) is a one-grid finite-depth probe scale,
not an error estimate and not an assumption in the covariance derivation.}
\label{tab:SM_grid_diagnostics}
\begingroup
\small
\setlength{\tabcolsep}{2.0pt}
\renewcommand{\arraystretch}{0.75}
\makebox[\linewidth][c]{%
\begin{minipage}{0.88\linewidth}
\begin{ruledtabular}
\begin{tabular}{@{}rccccccc@{}}
\(\omega\) &
\(\epsilon_g\sqrt{\omega}\) &
\(q_\omega\) &
\(\Delta_{\rm bud}^{\rm rel}\) &
\(\mathbb E[s^2]\) &
\(\beta_\omega^{\rm bl}\) &
\(\Lambda_\omega\) &
\(\mathcal E_{2{\rm br}}\) \\
\hline
1   & 0.013 & \(1.7\times10^{-4}\) & \(1.8\times10^{-5}\) & 0.978 & \(-8.0\times10^{-2}\) & \(-8.0\times10^{-2}\) & \(1.8\times10^{-3}\) \\
50  & 0.094 & \(2.4\times10^{-2}\) & \(4.0\times10^{-4}\) & 2.744 & \(-2.5\times10^{-2}\) & \(-1.8\times10^{-1}\) & \(1.5\times10^{-2}\) \\
100 & 0.133 & \(5.6\times10^{-2}\) & \(7.2\times10^{-4}\) & 3.140 & \(3.2\times10^{-2}\) & \(3.2\times10^{-1}\) & \(3.0\times10^{-2}\) \\
200 & 0.189 & \(1.0\times10^{-1}\) & \(6.8\times10^{-4}\) & 2.919 & \(2.1\times10^{-2}\) & \(3.0\times10^{-1}\) & \(5.4\times10^{-2}\) \\
300 & 0.231 & \(1.4\times10^{-1}\) & \(2.4\times10^{-4}\) & 2.650 & \(1.0\times10^{-2}\) & \(1.8\times10^{-1}\) & \(7.6\times10^{-2}\) \\
\end{tabular}
\end{ruledtabular}
\end{minipage}%
}
\endgroup
\end{table}
The detector-budget mismatch stays below \(10^{-3}\). The scaled tangential moment
\(\mathbb E[s^2]\) remains order-one, confirming that the relevant discrete
tangential scale is \(R_h=\sqrt{\omega}\,s\). The covariance coefficient
\(\beta_\omega^{\rm bl}\) remains bounded, so the local source has the form
\(\Lambda_\omega=\sqrt{\omega}\beta_\omega^{\rm bl}\). The sign of
\(\beta_\omega^{\rm bl}\) is not itself the mechanism; the diagnostic supports the
scale \(R_h\sim\sqrt{\omega}\). The two-branch continuation defect remains below
about \(8\%\), showing that the homogeneous spinor-ABC continuation captures the
near-roof trace at one grid depth with controlled finite-grid defect.

\subsection{Duhamel estimate}
\label{subsec:SM_Duhamel_estimate}

This subsection proves the estimate used in Sec.~\ref{subsec:SM_exact_near_roof_identity}.
Starting from Eq.~\eqref{eq:SM_Duhamel_remainder}, assume that
\(\widehat{\mathcal E}_{\rm bc}\) is \(C^1\) in the normal variable on
\(L-\epsilon\le z\le L\). Define
\begin{equation}
        G_\omega(\boldsymbol\xi,t;\epsilon)
        =
        \sup_{0\le u\le\epsilon}
        \left\|
        \partial_z\widehat{\mathcal E}_{\rm bc}
        (\boldsymbol\xi,L-u,t)
        \right\| .
        \label{eq:SM_Gomega_def}
\end{equation}
Since \(\widehat{\mathcal E}_{\rm bc}(\boldsymbol\xi,L,t)=0\),
\begin{equation}
        \left\|
        \widehat{\mathcal E}_{\rm bc}(\boldsymbol\xi,L-u,t)
        \right\|
        \le
        u\,G_\omega(\boldsymbol\xi,t;\epsilon).
        \label{eq:SM_Ebc_bound}
\end{equation}
Moreover, from
\(\mathcal C(\boldsymbol\xi)=i\kappa I+R\Gamma(\boldsymbol\xi)\),
\(\Gamma^2=I\), and \(R=|\boldsymbol\xi|\),
\begin{equation}
        \left\|
        e^{-(\epsilon-u)\mathcal C(\boldsymbol\xi)}
        \right\|
        \le
        e^{(\epsilon-u)R}
        \le
        e^{\epsilon R}.
        \label{eq:SM_exp_bound}
\end{equation}
Inserting Eqs.~\eqref{eq:SM_Ebc_bound} and \eqref{eq:SM_exp_bound} into
Eq.~\eqref{eq:SM_Duhamel_remainder} gives
\begin{equation}
\begin{aligned}
        \left\|
        \widehat{\mathcal E}_{\rm Duh}(\boldsymbol\xi,L-\epsilon,t)
        \right\|
        &\le
        e^{\epsilon R}
        G_\omega(\boldsymbol\xi,t;\epsilon)
        \int_0^\epsilon u\,du\\
        &=
        \frac{\epsilon^2}{2}
        e^{\epsilon R}
        G_\omega(\boldsymbol\xi,t;\epsilon).
\end{aligned}
        \label{eq:SM_Duhamel_bound}
\end{equation}
Thus, for each fixed tangential mode,
\begin{equation}
        \widehat{\mathcal E}_{\rm Duh}(\boldsymbol\xi,L-\epsilon,t)
        =
        O(\epsilon^2)
        \qquad
        (\epsilon\to0).
        \label{eq:SM_Duhamel_Oeps2}
\end{equation}
In particular,
\begin{equation}
        \widehat{\mathcal E}_{\rm Duh}(\boldsymbol\xi,L,t)=0,
        \qquad
        \left.
        \partial_\epsilon
        \widehat{\mathcal E}_{\rm Duh}(\boldsymbol\xi,L-\epsilon,t)
        \right|_{\epsilon=0}
        =0 .
        \label{eq:SM_Duhamel_no_first_order}
\end{equation}
Therefore the Duhamel remainder does not change the first inward normal variation
of the roof trace. The finite-grid counterpart of this statement is the continuation defect reported in Table~\ref{tab:SM_grid_diagnostics}.

The estimate~\ref{eq:SM_Duhamel_Oeps2}--\ref{eq:SM_Duhamel_no_first_order} is modewise; no uniform continuum
bound in \(\boldsymbol \xi\) or \(\omega\) is claimed here. In the finite-grid
implementation the sampled tangential spectrum is finite, and the
size of the one-grid probe is diagnosed by \(q_\omega\),
while the actual continuation mismatch is measured by
\(\mathcal E_{2{\rm br}}\) in Table~\ref{tab:SM_grid_diagnostics}.

\section{REDUCED RETURN CLOSURE}
\label{sec:SM_return_closure}
The boundary-symbol calculation identifies the local spinor-ABC scale
\begin{equation}
\Lambda_\omega=\sqrt{\omega}\,\beta^{\rm bl}_\omega .
\label{eq:SM_local_scale_return_intro}
\end{equation}
This is not yet a detection-time statistic. The physical observable is
the detector-present roof flux
\begin{equation}
g(t;\omega)=J_L(t).
\end{equation}
The purpose of this section is to give a reduced flux-balance and finite-guide memory closure explaining
how undetected spinor-ABC-filtered components can return to the roof and make the local scale
 \(R=|\boldsymbol\xi|\sim\sqrt{\omega}\) visible in finite-window moments.

 Introduce a near-roof matching plane and an auxiliary control layer
\begin{equation}
\Sigma_*=\{z=z_*\},\qquad z_*=L-\ell,\qquad
\Omega_{\rm bl}^{(\ell)}=\{(x,y,z):z_*<z<L\}.
\end{equation}
Let
\begin{equation}
P_{\rm bl}^{(\ell)}(t)=\int_{\Omega_{\rm bl}^{(\ell)}}\rho(x,y,z,t)\,dV,
\end{equation}
and define the signed matching-plane flux and the detected roof flux by
\begin{equation}
J_*(t)=\int_{\Sigma_*} j_z(x,y,z_*,t)\,dxdy,\qquad
J_L(t)=\int_{\Sigma_L} j_z(x,y,L,t)\,dxdy.
\end{equation}
Here \(j_z\) denotes the \(z\)-component of the Pauli current. The sign convention is that \(J_*(t)>0\) means flux entering the
near-roof layer from below. Since the spinor ABC gives
\begin{equation}
J_L(t)=\kappa\int_{\Sigma_L}\rho(x,y,L,t)\,dxdy\ge 0,
\end{equation}
the continuity equation in the auxiliary layer gives
\begin{equation}
\frac{d}{dt}P_{\rm bl}^{(\ell)}(t)=J_*(t)-J_L(t).
\label{eq:SM_layer_balance}
\end{equation}
Thus probability entering the near-roof layer may be detected at the
roof, remain temporarily stored in the layer, or leave the layer again
through \(\Sigma_*\) as an undetected filtered component.

Let \(F_{\rm out}^{\rm nc}(t;\omega,\ell)\) denote the effective
outgoing no-click flux of undetected, spinor-ABC-filtered amplitude
through \(\Sigma_*\). This object is not measured directly and is not
equal to the detected roof flux. A causal return kernel
\(k_{\omega,\ell}^{\rm ret}(u)\) then represents the later contribution
to the roof flux from such undetected components after propagation
through the finite guide. Here and below \(u\ge0\) denotes a time lag:
\(F_{\rm out}^{\rm nc}(t-u;\omega,\ell)\) is the no-click flux that
left the near-roof layer at the earlier time \(t-u\), and
\(k_{\omega,\ell}^{\rm ret}(u)\) is the effective weight for that
component to contribute to the roof flux after delay \(u\). Therefore
\begin{equation}
g_{\rm box}(t;\omega)
=
g_{\rm first}(t;\omega)
+
\int_0^t
k_{\omega,\ell}^{\rm ret}(u)
F_{\rm out}^{\rm nc}(t-u;\omega,\ell)\,du,
\label{eq:SM_return_closure}
\end{equation}
where \(g_{\rm first}\) denotes the roof flux associated with the first near-roof encounter before a full return from the guide. Equation~\eqref{eq:SM_return_closure} is a reduced flux-level closure, not an exact
mode-resolved TDSE decomposition. It summarizes the delayed influence
of an unresolved no-click channel after phase, branch, and mode
information have been compressed into an effective scalar kernel.

For a one-channel moment estimate, one may eliminate the unresolved
no-click flux \(F_{\rm out}^{\rm nc}\) into an effective causal memory
kernel \(k_{\omega,\ell}^{\rm eff}\). This second kernel should not be
identified with \(k_{\omega,\ell}^{\rm ret}\): it also contains the
unresolved relation between the hidden no-click flux and the previous
roof/near-roof history. This gives the scalar Volterra closure
\begin{equation}
g_{\rm box}
=
g_{\rm first}
+
K^{\rm eff}_{\omega,\ell}g_{\rm box},
\qquad
(K^{\rm eff}_{\omega,\ell}f)(t)
=
\int_0^t k^{\rm eff}_{\omega,\ell}(u)f(t-u)\,du .
\end{equation}
The occurrence of \(g_{\rm box}\) on the right-hand side should not be
read as already detected probability returning to the detector. It is
the result of eliminating the unresolved undetected channel into an
effective memory kernel. The effective kernel describes the delayed influence of
surviving, branch-reweighted amplitude.

If \(K^{\rm eff}_{\omega,\ell}\) is contractive, for example
\(\|k^{\rm eff}_{\omega,\ell}\|_1<1\), then formally
\begin{equation}
g_{\rm box}
=
(I-K^{\rm eff}_{\omega,\ell})^{-1}g_{\rm first}
=
\sum_{n=0}^{\infty}
(K^{\rm eff}_{\omega,\ell})^n g_{\rm first}.
\end{equation}
For an untruncated causal flux \(f\), define
\begin{equation}
M_0[f]=\int_0^\infty f(t)\,dt,\qquad
M_1[f]=\int_0^\infty t f(t)\,dt.
\end{equation}
Let
\begin{equation}
m_{\rm ret}^{(0)}
=
\int_0^\infty k^{\rm eff}_{\omega,\ell}(u)\,du,\qquad
m_{\rm ret}^{(1)}
=
\int_0^\infty u\,k^{\rm eff}_{\omega,\ell}(u)\,du,
\end{equation}
when \(m^{(0)}_{\rm ret}\neq 0\), define the normalized first moment of the effective
returned channel by
\begin{equation}
\bar U_{\rm ret}(\omega;\ell)
:=
\frac{m^{(1)}_{\rm ret}}{m^{(0)}_{\rm ret}} .
\end{equation}
If \(k^{\rm eff}_{\omega,\ell}\) is nonnegative, \(m^{(0)}_{\rm ret}\) may be interpreted as an
effective return probability and \(\bar U_{\rm ret}\) as the mean return delay. In general,
they are only the zeroth moment and normalized first moment of the reduced memory
kernel. The corresponding convolution identities therefore yield
\begin{equation}
M_0[K^{\rm eff}_{\omega,\ell}f]
=
m_{\rm ret}^{(0)}M_0[f],
\end{equation}
and
\begin{equation}
M_1[K^{\rm eff}_{\omega,\ell}f]
=
m_{\rm ret}^{(0)}M_1[f]
+
m_{\rm ret}^{(1)}M_0[f].
\end{equation}
Consequently, for the corresponding untruncated mean time,
\begin{equation}
\bar\tau_{\rm box}
=
\bar\tau_{\rm first}
+
\frac{m_{\rm ret}^{(1)}}{1-m_{\rm ret}^{(0)}} .
\label{eq:SM_return_mean}
\end{equation}
This equation is not used as a fit model for the numerical data. It only shows how a delayed effective memory kernel shifts a flux first moment. 

The local spinor-ABC filtering enters the returned component through the same tangential scale inherited from the roof response. For the harmonic transverse family,
\begin{equation}
R=|\boldsymbol\xi|=\sqrt{\omega}\,s,
\end{equation}
with \(s\) dimensionless and order one. The returned component has been filtered by the boundary, propagated through the finite guide, and re-entered the near-roof region. Therefore its effective coefficient need not equal \(\beta^{\rm bl}_\omega\).  We write this returned-channel coefficient as \(\beta^{\rm ret}_\omega\), and use the reduced moment
ansatz
\begin{equation}
\bar U_{\rm ret}(\omega;\ell)
:=
\frac{m_{\rm ret}^{(1)}}{m_{\rm ret}^{(0)}}
\simeq
U_{\rm bulk,ret}(\ell)+c_0(\ell)
+c_1(\ell)\sqrt{\omega}\,\beta^{\rm ret}_\omega .
\label{eq:SM_return_delay_ansatz}
\end{equation}
Since \(m_{\rm ret}^{(1)}=m_{\rm ret}^{(0)}\bar U_{\rm ret}\),
Eq.~\eqref{eq:SM_return_mean} can be written as
\begin{equation}
\bar\tau_{\rm box}
=
\bar\tau_{\rm first}
+
\alpha_{\rm ret}(\omega;\ell)\,
\bar U_{\rm ret}(\omega;\ell),
\qquad
\alpha_{\rm ret}(\omega;\ell)
:=
\frac{m_{\rm ret}^{(0)}(\omega;\ell)}
{1-m_{\rm ret}^{(0)}(\omega;\ell)} .
\end{equation}
Thus \(m_{\rm ret}^{(0)}\) controls the effective amount of returned
weight, while \(\bar U_{\rm ret}\) controls its effective delay. Combining Eqs.~\eqref{eq:SM_return_mean} and~\eqref{eq:SM_return_delay_ansatz} gives, over a finite fitted range,
\begin{equation}
\bar\tau_{\rm box}(\omega)
\simeq
A_0(\ell,T)+B_0(\ell,T)\sqrt{\omega}
+\mathcal R_{\rm eff}(\omega;\ell,T),
\end{equation}
where \(\mathcal R_{\rm eff}\) collects finite-window truncation, the variation of the effective return probability, and the residual \(\omega\)-dependence of the returned-channel coefficient.
When this remainder varies slowly over the sampled range, the finite-window moment is well approximated by an affine function of \(\sqrt{\omega}\).

Finally, the detection statistic plotted in the main text is the finite-window
restricted mean detection-time statistics, not the untruncated conditional mean. As shown in Sec.~\ref{sec:SM_finite_window},
\begin{equation}
\mu^*(T;\omega)
=
D_T(\omega)\,\bar\tau_T^{\rm cond}(\omega)
+
[1-D_T(\omega)]T .
\end{equation}
Therefore the observed finite-window coefficient receives contributions both from delayed conditional timing and from the decreasing detected fraction. 

Importantly, the closure is not a mode-resolved solution of the TDSE and is not used to fit the data. Its only purpose is to show how an undetected no-click channel, once compressed into an effective causal memory kernel, can transfer the local boundary scale $R\sim\sqrt{\omega}$ into finite-window roof-flux moments. Therefore the observed affine-in-$\sqrt{\omega}$ behavior should be read as a finite-range detector-response signature, not as a universal asymptotic law.

\section{Control Checks}
\label{sec:SM_controls}

This section records exploratory control checks addressing two questions:
whether the spinor-ABC delayed sector is removed by representative bulk spin
perturbations when the spinor ABC is retained, and whether the same
confinement trend can be reproduced without the spinor ABC by using generic
spin-dependent absorbing Hamiltonian layers. These controls are not used to
establish the fitted scaling or to prove uniqueness of the spinor ABC. Within
the tested parameter ranges, bulk spin perturbations did not substantially
remove the delayed sector, and generic absorbing Hamiltonian layers did not
robustly reproduce the spinor-ABC confinement trend.

\subsection{Bulk spin and transverse-state controls}
\label{subsec:SM_bulk_spin_controls}

We first kept the spinor absorbing boundary fixed and modified only the bulk
Hamiltonian,
\begin{equation}
        H=H_{\rm waveguide}(\omega)+H_{\rm spin}.
\end{equation}
Representative choices of \(H_{\rm spin}\) included localized Rabi--Zeeman terms,
transverse Zeeman gradients, Rashba and Rashba--Dresselhaus spin--orbit
couplings, and a Pauli magnetic minimal-coupling Hamiltonian. In the magnetic
case, the roof condition was replaced by the corresponding gauge-covariant
spinor ABC,
\begin{equation}
        (\boldsymbol\sigma\cdot \boldsymbol D)\Psi=i\kappa\sigma_z\Psi,
        \qquad
        \boldsymbol D=\boldsymbol\nabla-iq\boldsymbol A .
\end{equation}
We also tested whether the effect depends essentially on preparing the transverse
harmonic ground state by replacing \(\chi_{00}^{(\omega)}\) with first excited
transverse modes and with the chiral combination
\begin{equation}
        \chi_{\rm chiral}^{(\omega)}
        =
        \frac{\chi_{10}^{(\omega)}+i\chi_{01}^{(\omega)}}{\sqrt2}.
\end{equation}
Within the tested parameter range, these modifications did not substantially
remove the delayed sector relative to the spinor-ABC reference run. Thus the
confinement dependence is not primarily caused by generic bulk spin dynamics or
by the special choice of the transverse ground state. The dominant source remains
the boundary response.

\subsection{Hamiltonian-layer mimics}
\label{subsec:SM_layer_mimics}

We next asked whether the spinor-ABC delay can be reproduced without imposing
the spinor ABC at the detector surface. We replaced the boundary condition by a
finite absorbing Hamiltonian layer,
\begin{equation}
        L_{\rm det}<z<L_{\rm det}+\ell_{\rm det},
\end{equation}
with a smooth turn-on function \(\chi(z)\) and a Dirichlet wall at the far end of
the layer:
\begin{equation}
        H=H_{\rm waveguide}(\omega)+H_{\rm layer}.
\end{equation}
We considered ordinary spin-dependent absorbing layers, including Rashba-type loss and helicity-based tangential-momentum loss. These models did not robustly
reproduce the spinor-ABC confinement dependence. For comparison, we also considered an inverse-engineered impedance layer. Let
\begin{equation}
        K=\sigma_xp_y-\sigma_yp_x,
        \qquad
        R=(p_x^2+p_y^2)^{1/2},
        \qquad
        p_j=-i\partial_j .
\end{equation}
In tangential Fourier variables, \(K\) has eigenvalues \(\pm R\), and \(K/R\)
separates the two tangential spin--momentum branches. The inverse-engineered
layer was chosen so that, in a stationary Dirichlet-backed calibration, its two
branch impedances approximate
\begin{equation}
        i\kappa-R,
        \qquad
        i\kappa+R .
\end{equation}
This model is not a generic absorbing layer. It explicitly builds the
spinor-ABC branch impedances into the layer. Therefore these controls support
a more specific conclusion: generic absorbing layers or scalar absorber
reflection do not reproduce the spinor-ABC confinement trend. Separately, the
bulk perturbation checks in Sec.~\ref{subsec:SM_bulk_spin_controls} show that representative bulk spin
dynamics do not explain away the delayed sector when the spinor ABC is
retained. Reproducing the response requires an effective entrance impedance
with the same tangential branch structure \(i\kappa\pm|\boldsymbol{\xi}|\) by construction.

\section{Parameter scans and robustness checks}
\label{sec:SM_parameter_scans}

This section records how the spinor-ABC roof-flux statistics change when source or detector parameters are varied. These scans are not used to derive a new scaling law. Their purpose is to show that fitted coefficients, detected fractions, and late-time tails depend on the finite-window source/detector geometry, while the local transverse scale remains
\begin{equation}
 R=|\boldsymbol\xi|\sim\sqrt{\omega}.
\end{equation}
Thus, when an affine-in-\(\sqrt\omega\) fit is used, its coefficients should be read as source-, detector-, geometry-, and window-dependent.

\subsection{\texorpdfstring{\(\kappa\)-scan}{kappa-scan}}
\label{subsec:SM_kappa_scan}

Figure~\ref{fig:SM_kappa_scan} and Table~\ref{tab:SM_kappa_scan} show the
dependence on the boundary parameter \(\kappa\), with \(k_z=\pi\),
\(\sigma_\parallel=0.5\), and \(\omega=1\) fixed. The finite-window statistic is smallest
near the longitudinally matched value \(\kappa\simeq k_z=\pi\). Moving
\(\kappa\) below or above this value increases \(\mu^*(T;\kappa)\) and changes the
late-time tail.

This is consistent with the scalar one-dimensional reference picture, in which a
Robin absorber is best matched near \(\kappa=k_z\). For the spinor ABC this is
only a longitudinal matching guide: the transverse confinement mechanism remains
controlled by
\begin{equation}
        R=|\boldsymbol\xi|\sim\sqrt{\omega}.
\end{equation}

\begin{figure}[H]
  \centering
  \begin{minipage}[t]{0.44\linewidth}
    \centering
    \includegraphics[width=\linewidth]{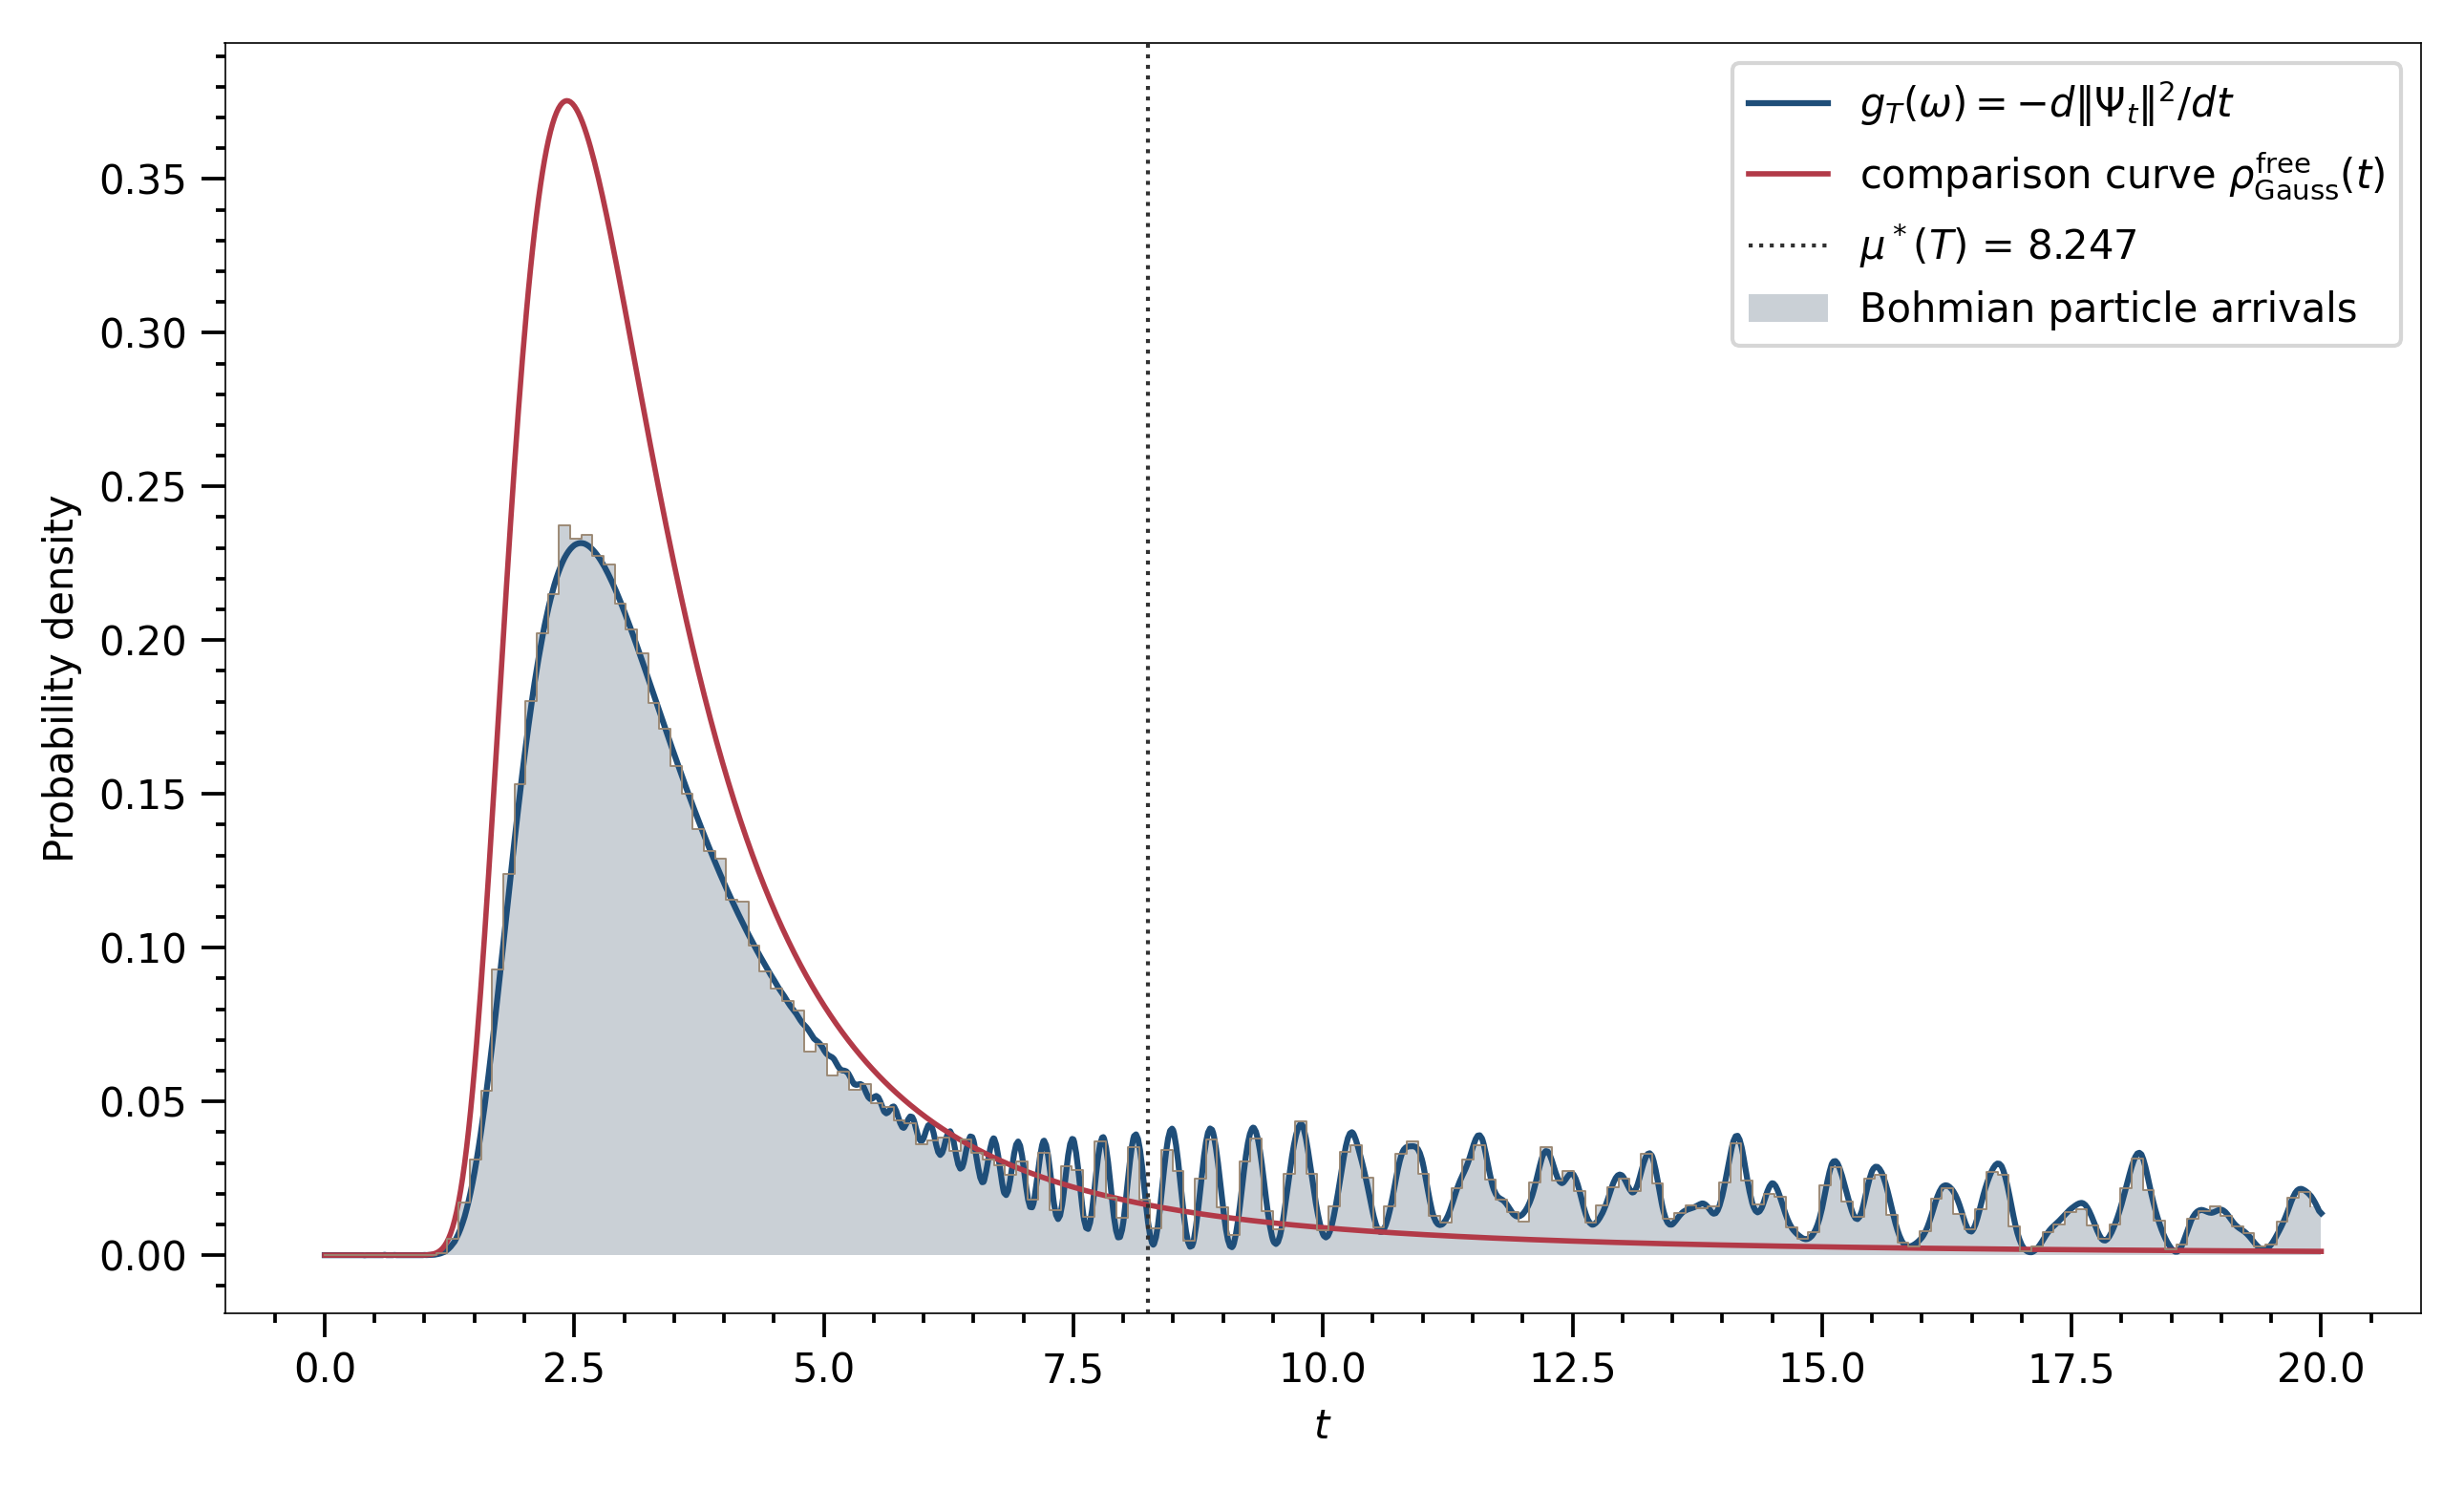}
    \par\vspace{0.2em}
    {\small (a) $\kappa=1$}
  \end{minipage}%
  \hspace{0.035\linewidth}%
  \begin{minipage}[t]{0.44\linewidth}
    \centering
    \includegraphics[width=\linewidth]{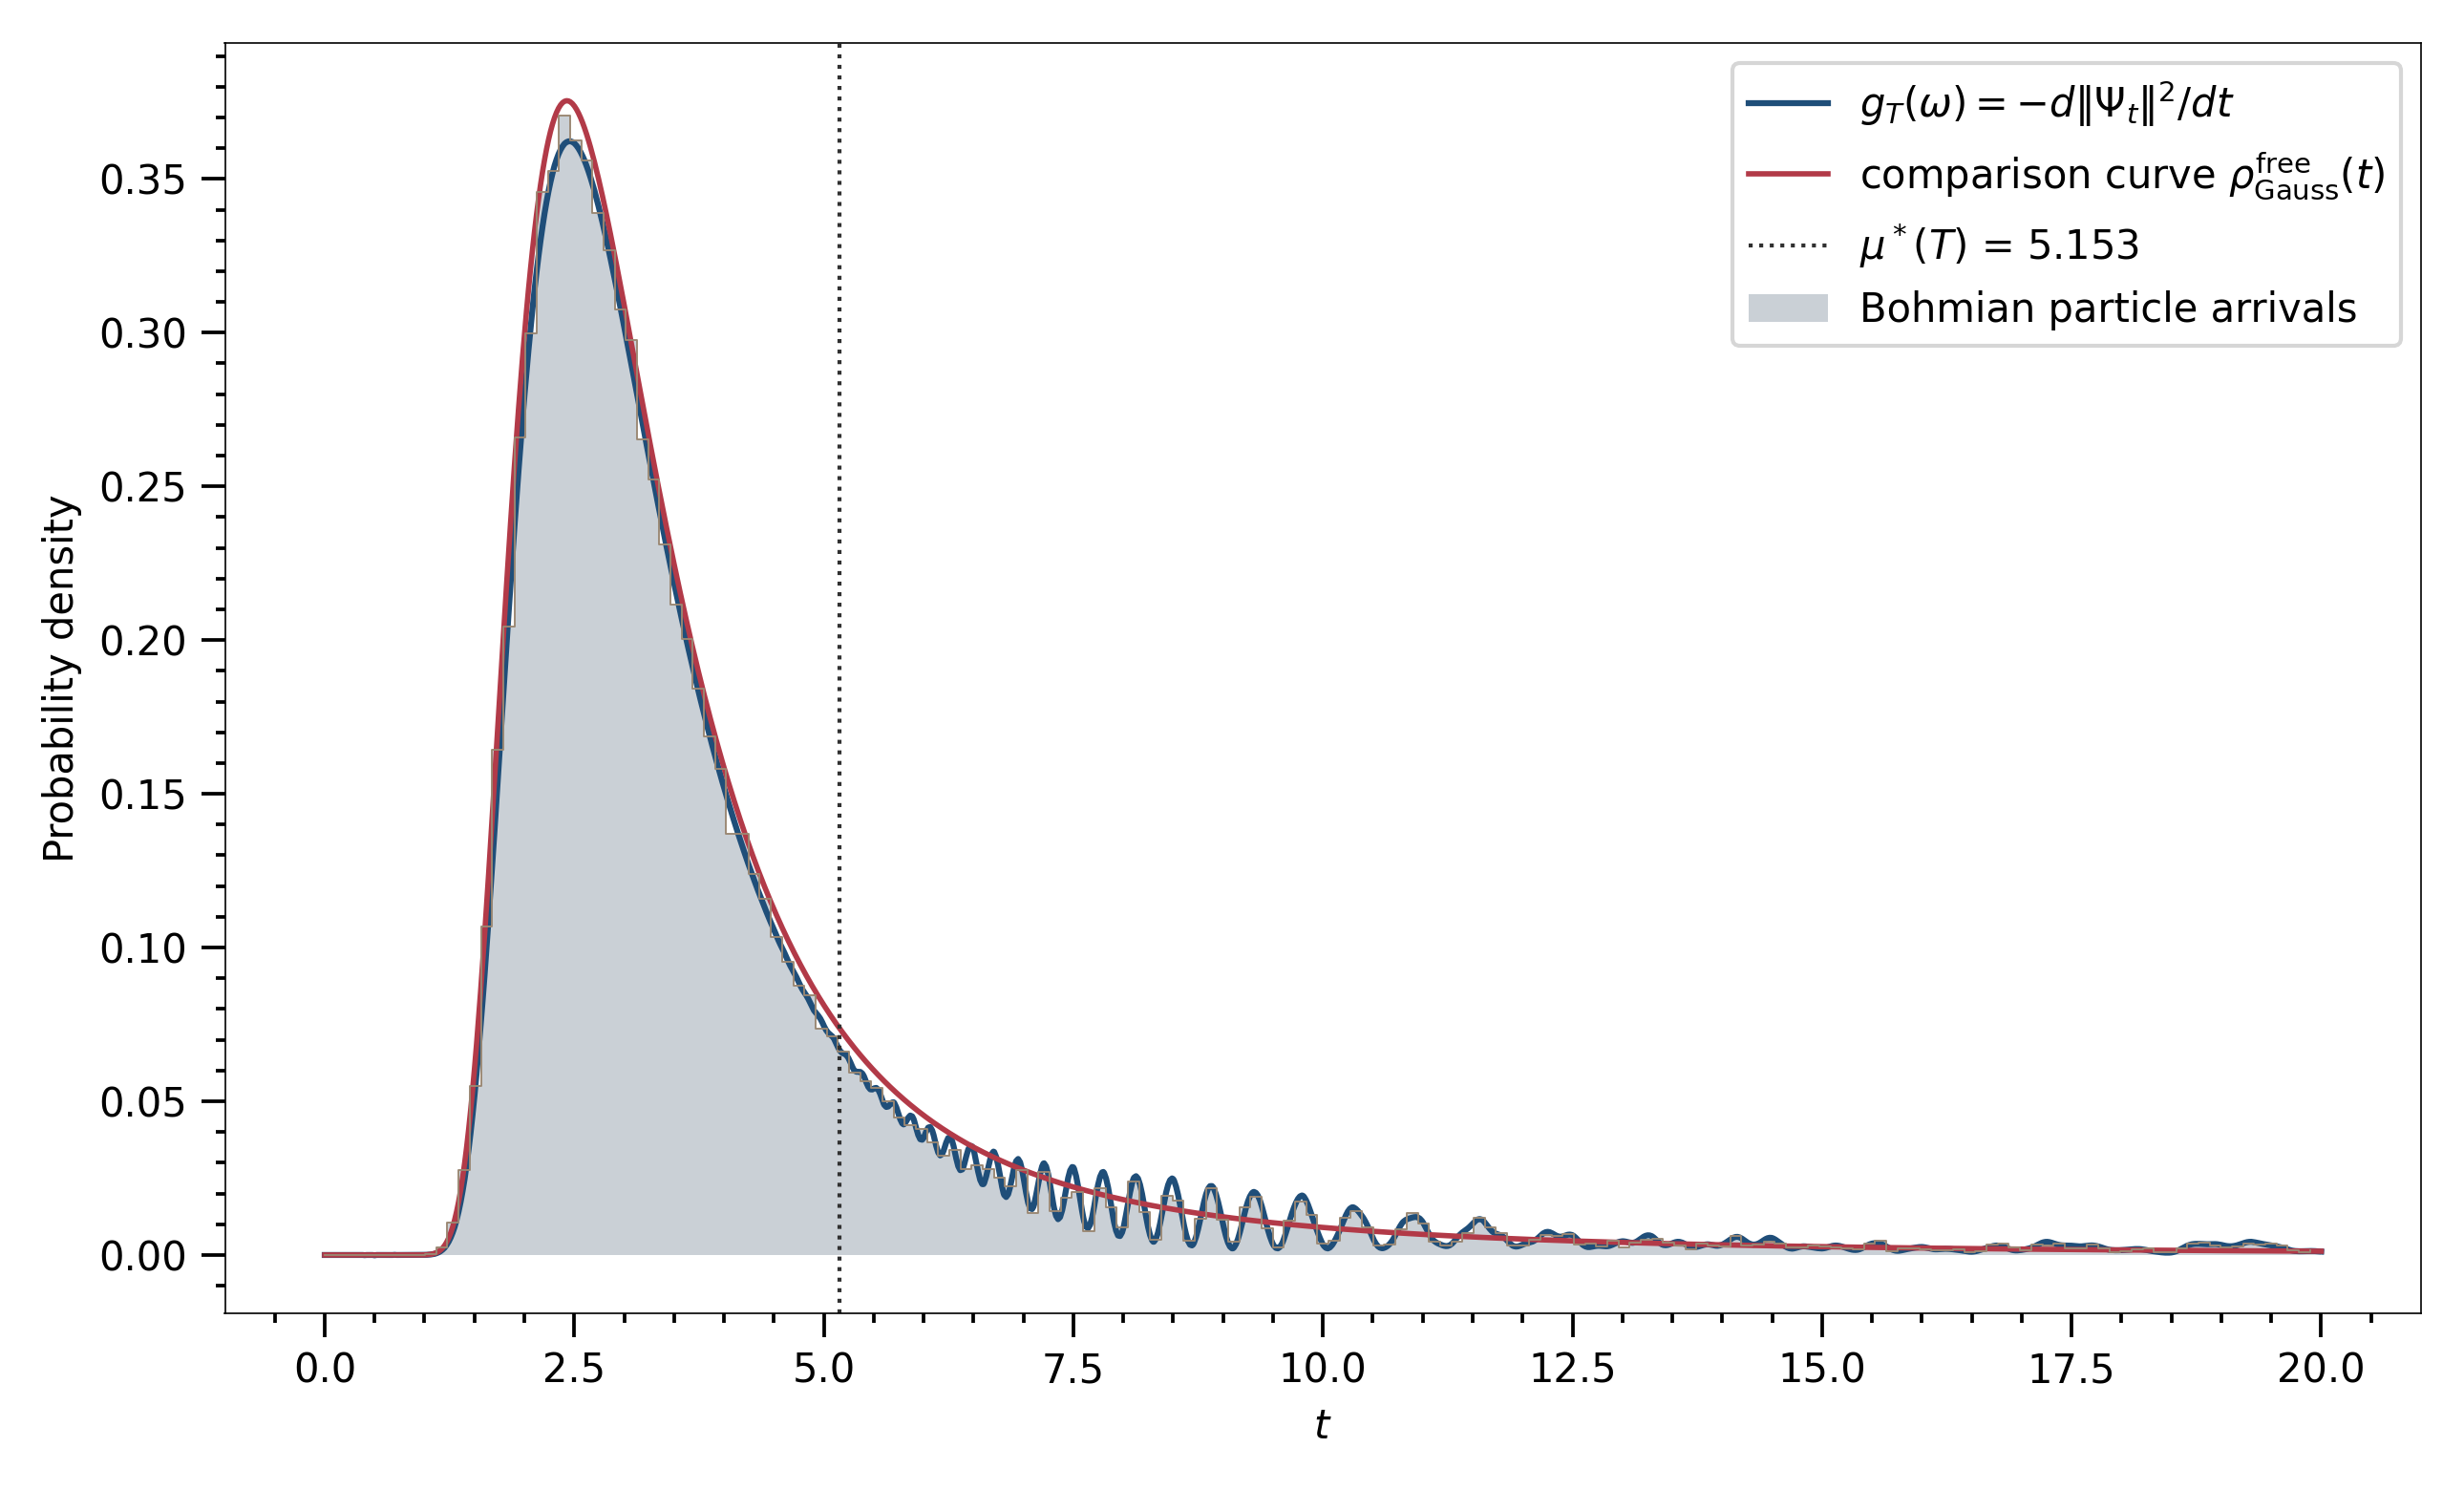}
    \par\vspace{0.2em}
    {\small (b) $\kappa=\pi$}
  \end{minipage}

  \vspace{0.8em}

  \begin{minipage}[t]{0.44\linewidth}
    \centering
    \includegraphics[width=\linewidth]{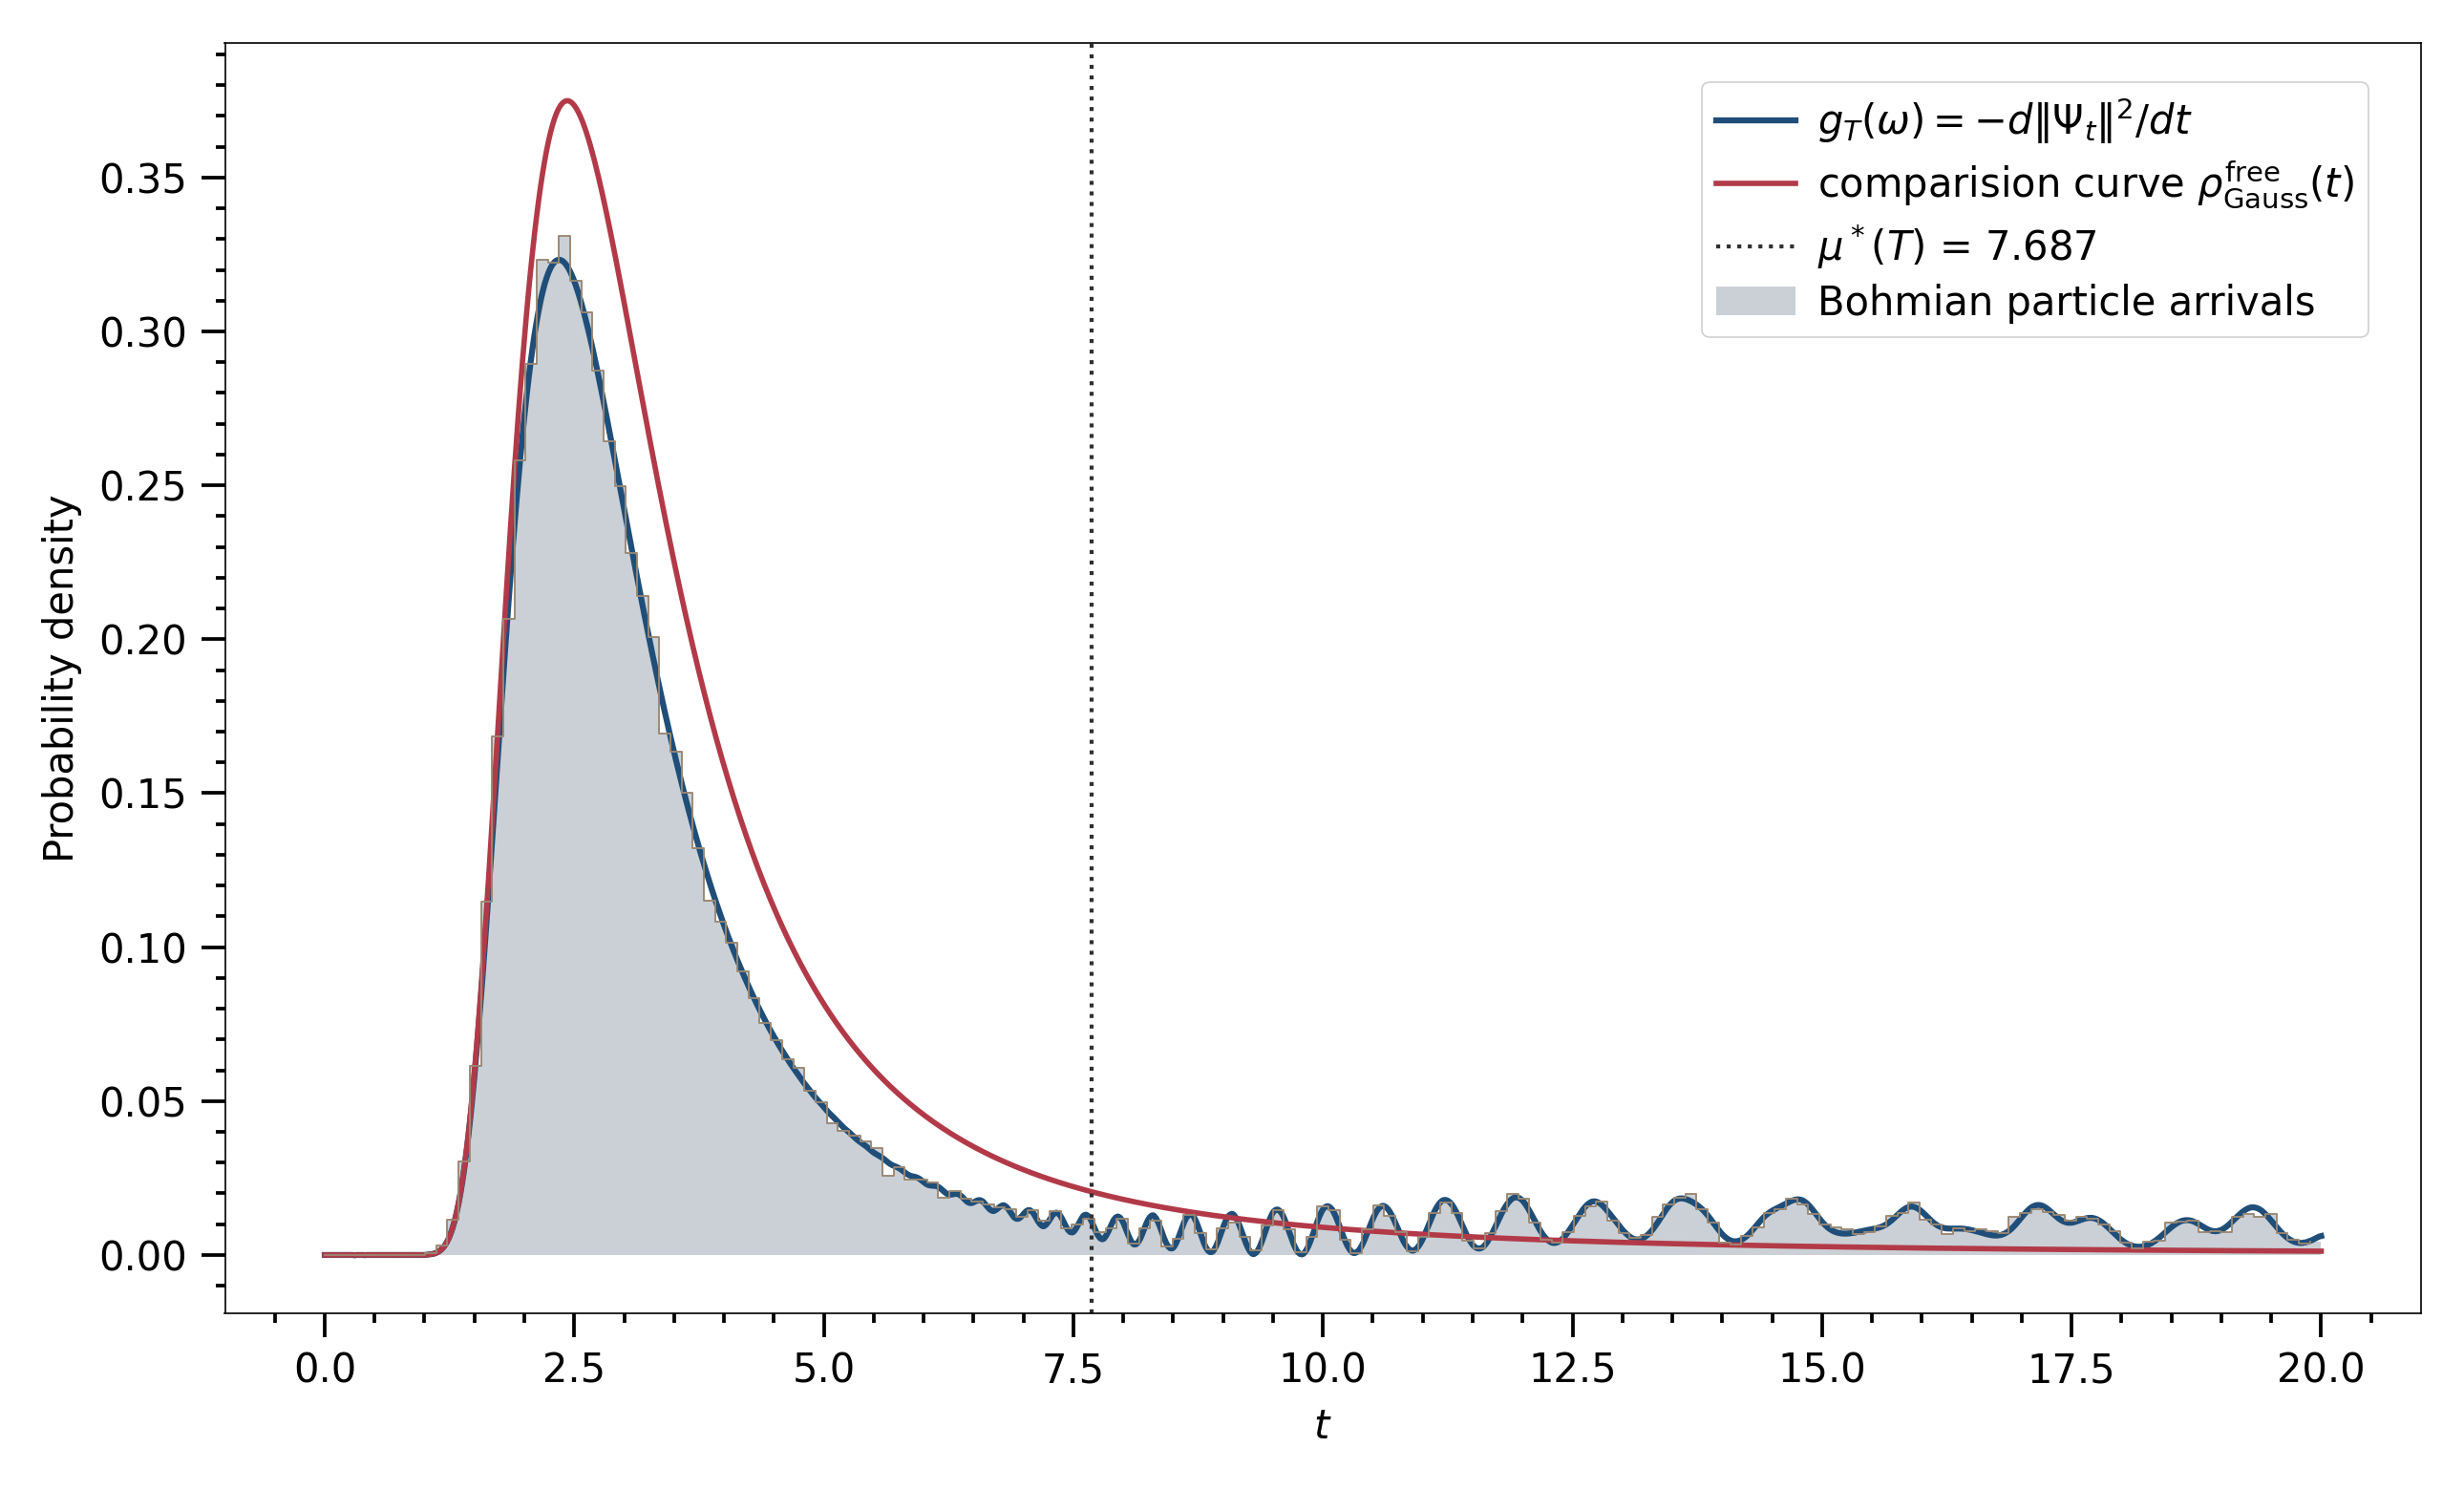}
    \par\vspace{0.2em}
    {\small (c) $\kappa=9$}
  \end{minipage}%
  \hspace{0.035\linewidth}%
  \begin{minipage}[t]{0.44\linewidth}
    \centering
    \includegraphics[width=\linewidth]{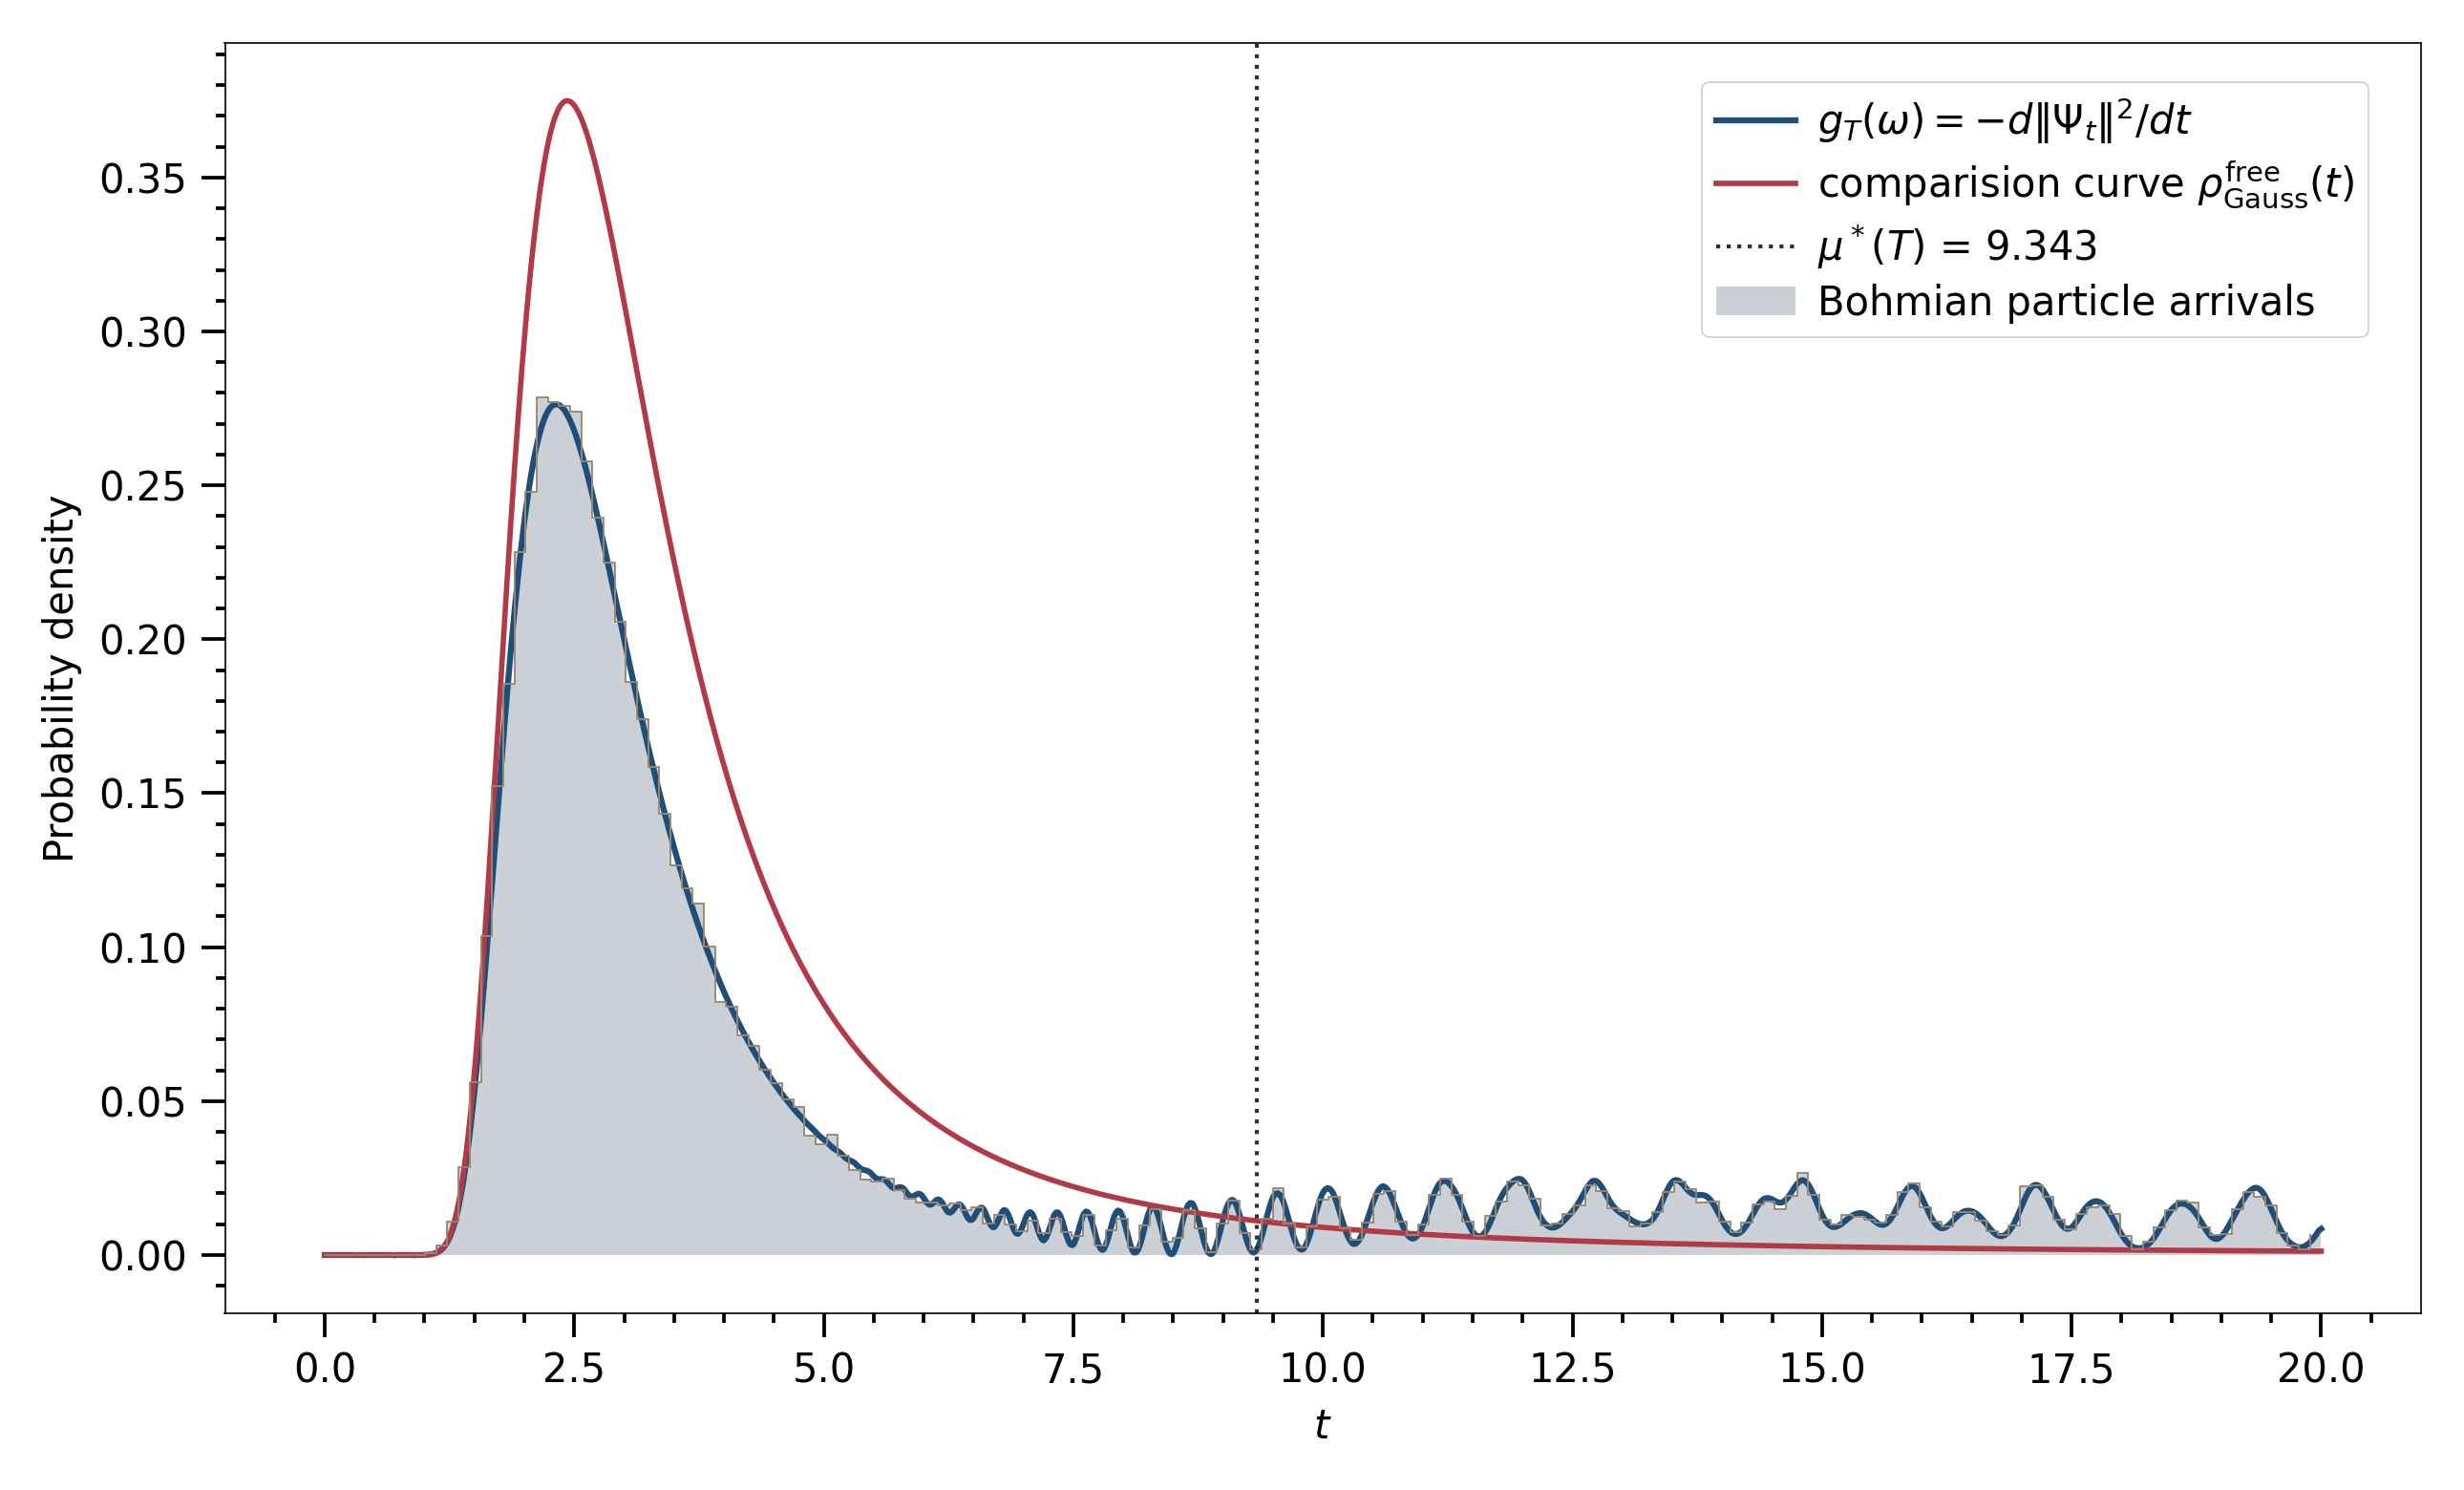}
    \par\vspace{0.2em}
    {\small (d) $\kappa=13$}
  \end{minipage}
  \caption{\(\kappa\)-scan for the spinor ABC. The parameters \(k_z=\pi\),
  \(\sigma_\parallel=0.5\), and \(\omega=1\) are fixed.}
  \label{fig:SM_kappa_scan}
\end{figure}

\begin{table}[H]
\caption{Finite-window statistic \(\mu^*(T;\kappa)\) for the \(\kappa\)-scan at
fixed \(\omega=1\), \(k_z=\pi\), and \(\sigma_\parallel=0.5\).}
\label{tab:SM_kappa_scan}
\begingroup
\small
\setlength{\tabcolsep}{2.5pt}
\renewcommand{\arraystretch}{0.95}
\makebox[\linewidth][c]{%
\begin{minipage}{0.72\linewidth}
\begin{ruledtabular}
\begin{tabular}{@{}c|ccccccccc@{}}
\(\kappa\) & 0.1 & 0.5 & 1 & 2 & \(\pi\) & 5 & 7 & 9 & 13 \\
\hline
\(\mu^*(T;\kappa)\) & 17.016 & 11.709 & 8.247 & 5.653 & 5.153 & 5.729 & 6.717 & 7.687 & 9.343
\end{tabular}
\end{ruledtabular}
\end{minipage}%
}
\endgroup
\end{table}

\subsection{\texorpdfstring{\(\sigma_\parallel\)-scan}{sigma-z scan}}
\label{subsec:SM_sigmaz_scan}

Changing \(\sigma_\parallel\) changes the longitudinal spatial width and momentum spread
of the incoming packet. Narrower packets have broader momentum support and
produce broader, more oscillatory detector-time profiles. Therefore \(\sigma_\parallel\)
affects the finite-window coefficients and detailed tails, but not the local
origin of the confinement scale.

\begin{figure}[H]
  \centering
  \begin{minipage}[t]{0.48\linewidth}
    \centering
    \includegraphics[width=\linewidth]{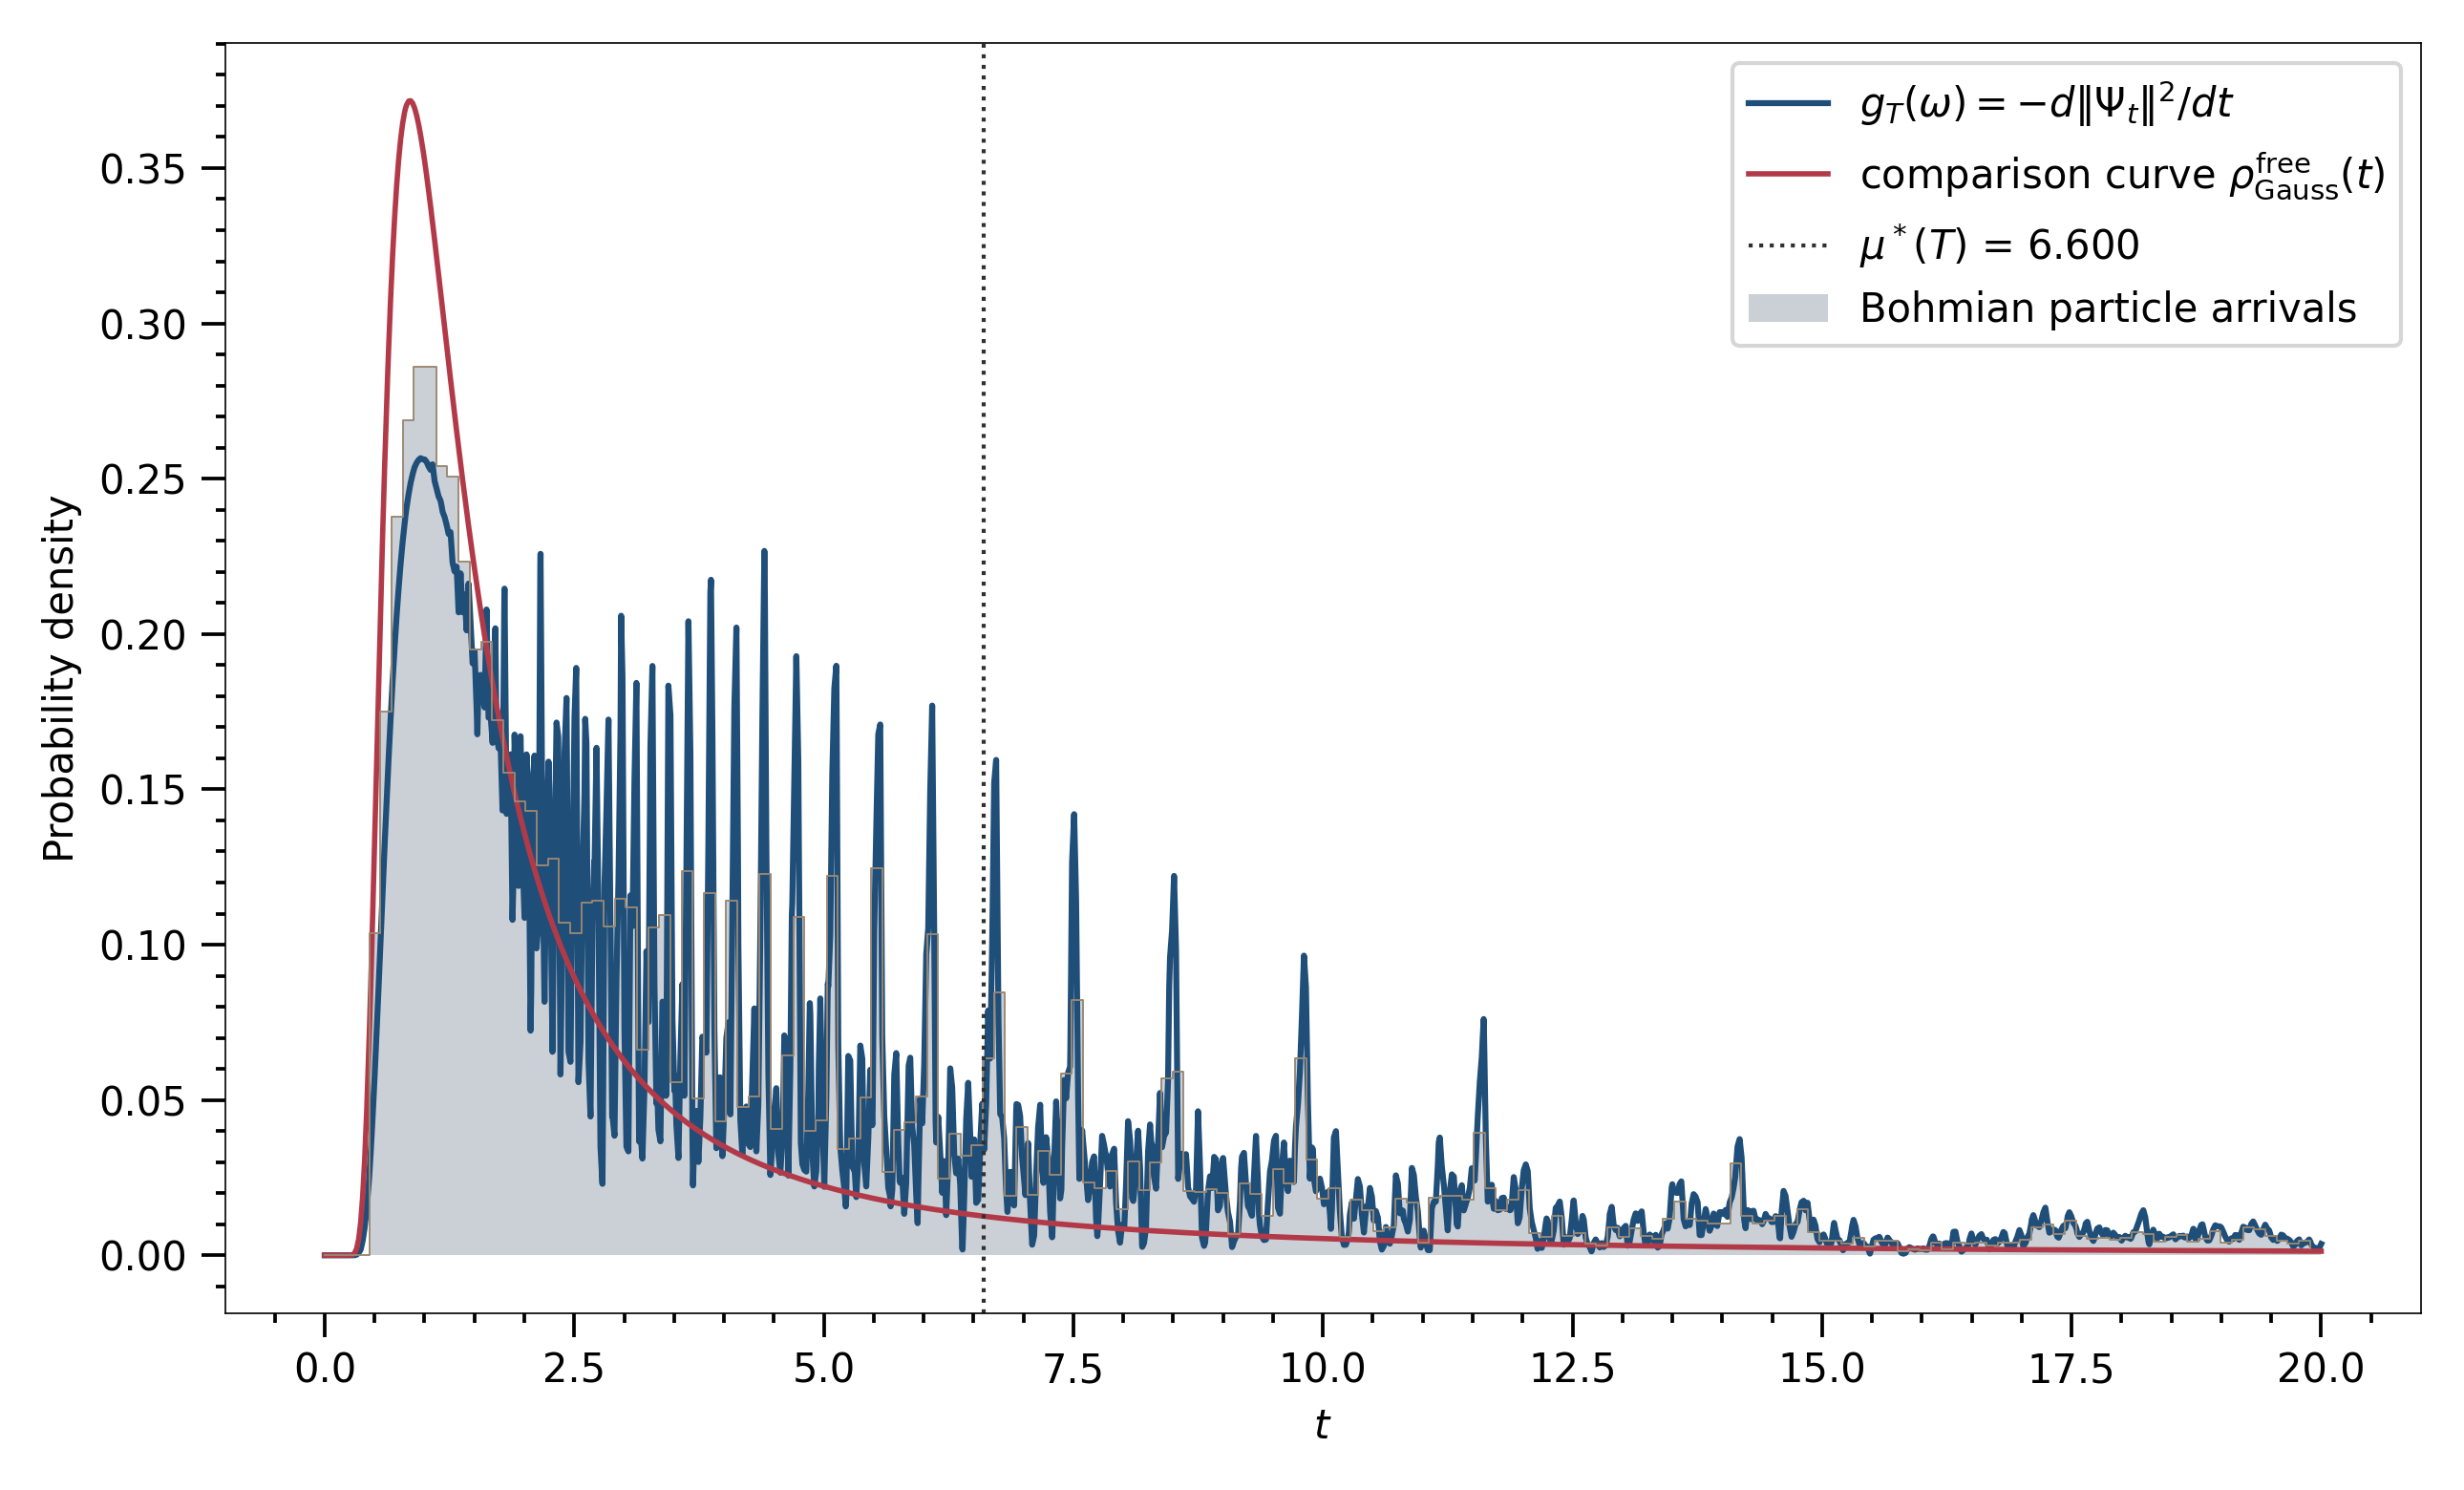}
    \par\vspace{0.3em}
    {\small (a) $\sigma_\parallel=0.1$}
  \end{minipage}\hfill
  \begin{minipage}[t]{0.48\linewidth}
    \centering
    \includegraphics[width=\linewidth]{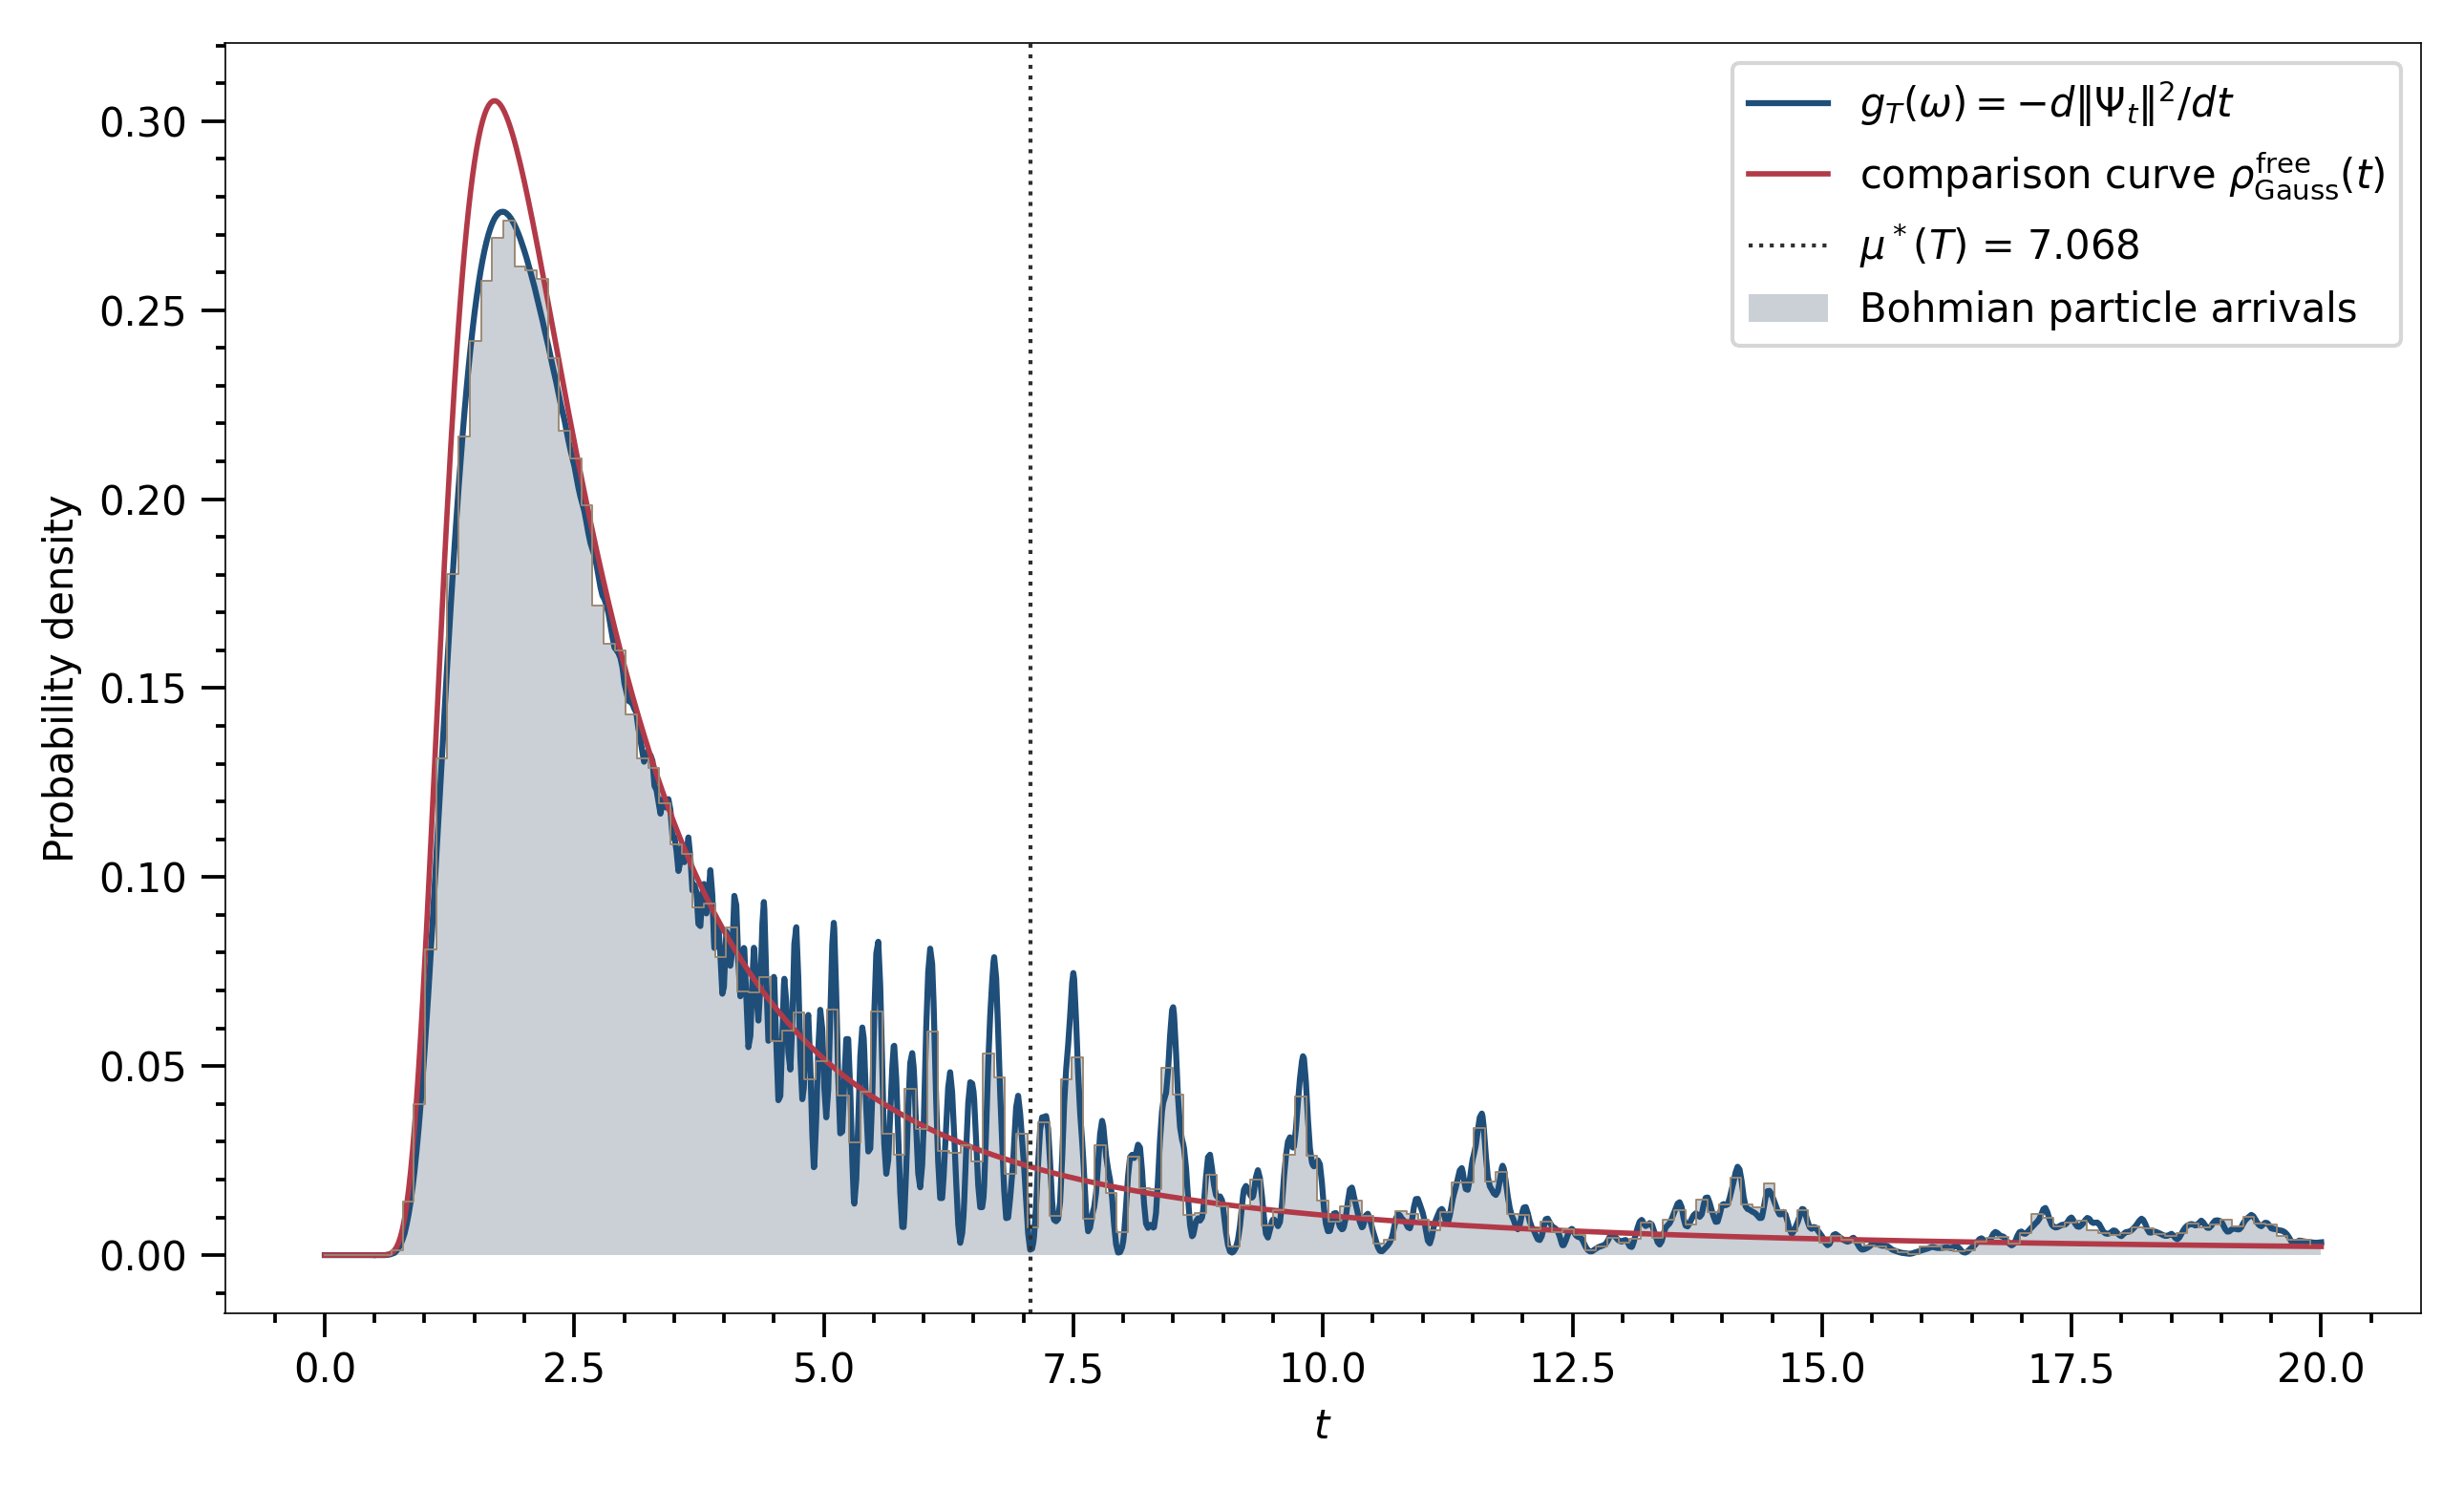}
    \par\vspace{0.3em}
    {\small (b) $\sigma_\parallel=0.25$}
  \end{minipage}

  \vspace{0.8em}

  \begin{minipage}[t]{0.48\linewidth}
    \centering
    \includegraphics[width=\linewidth]{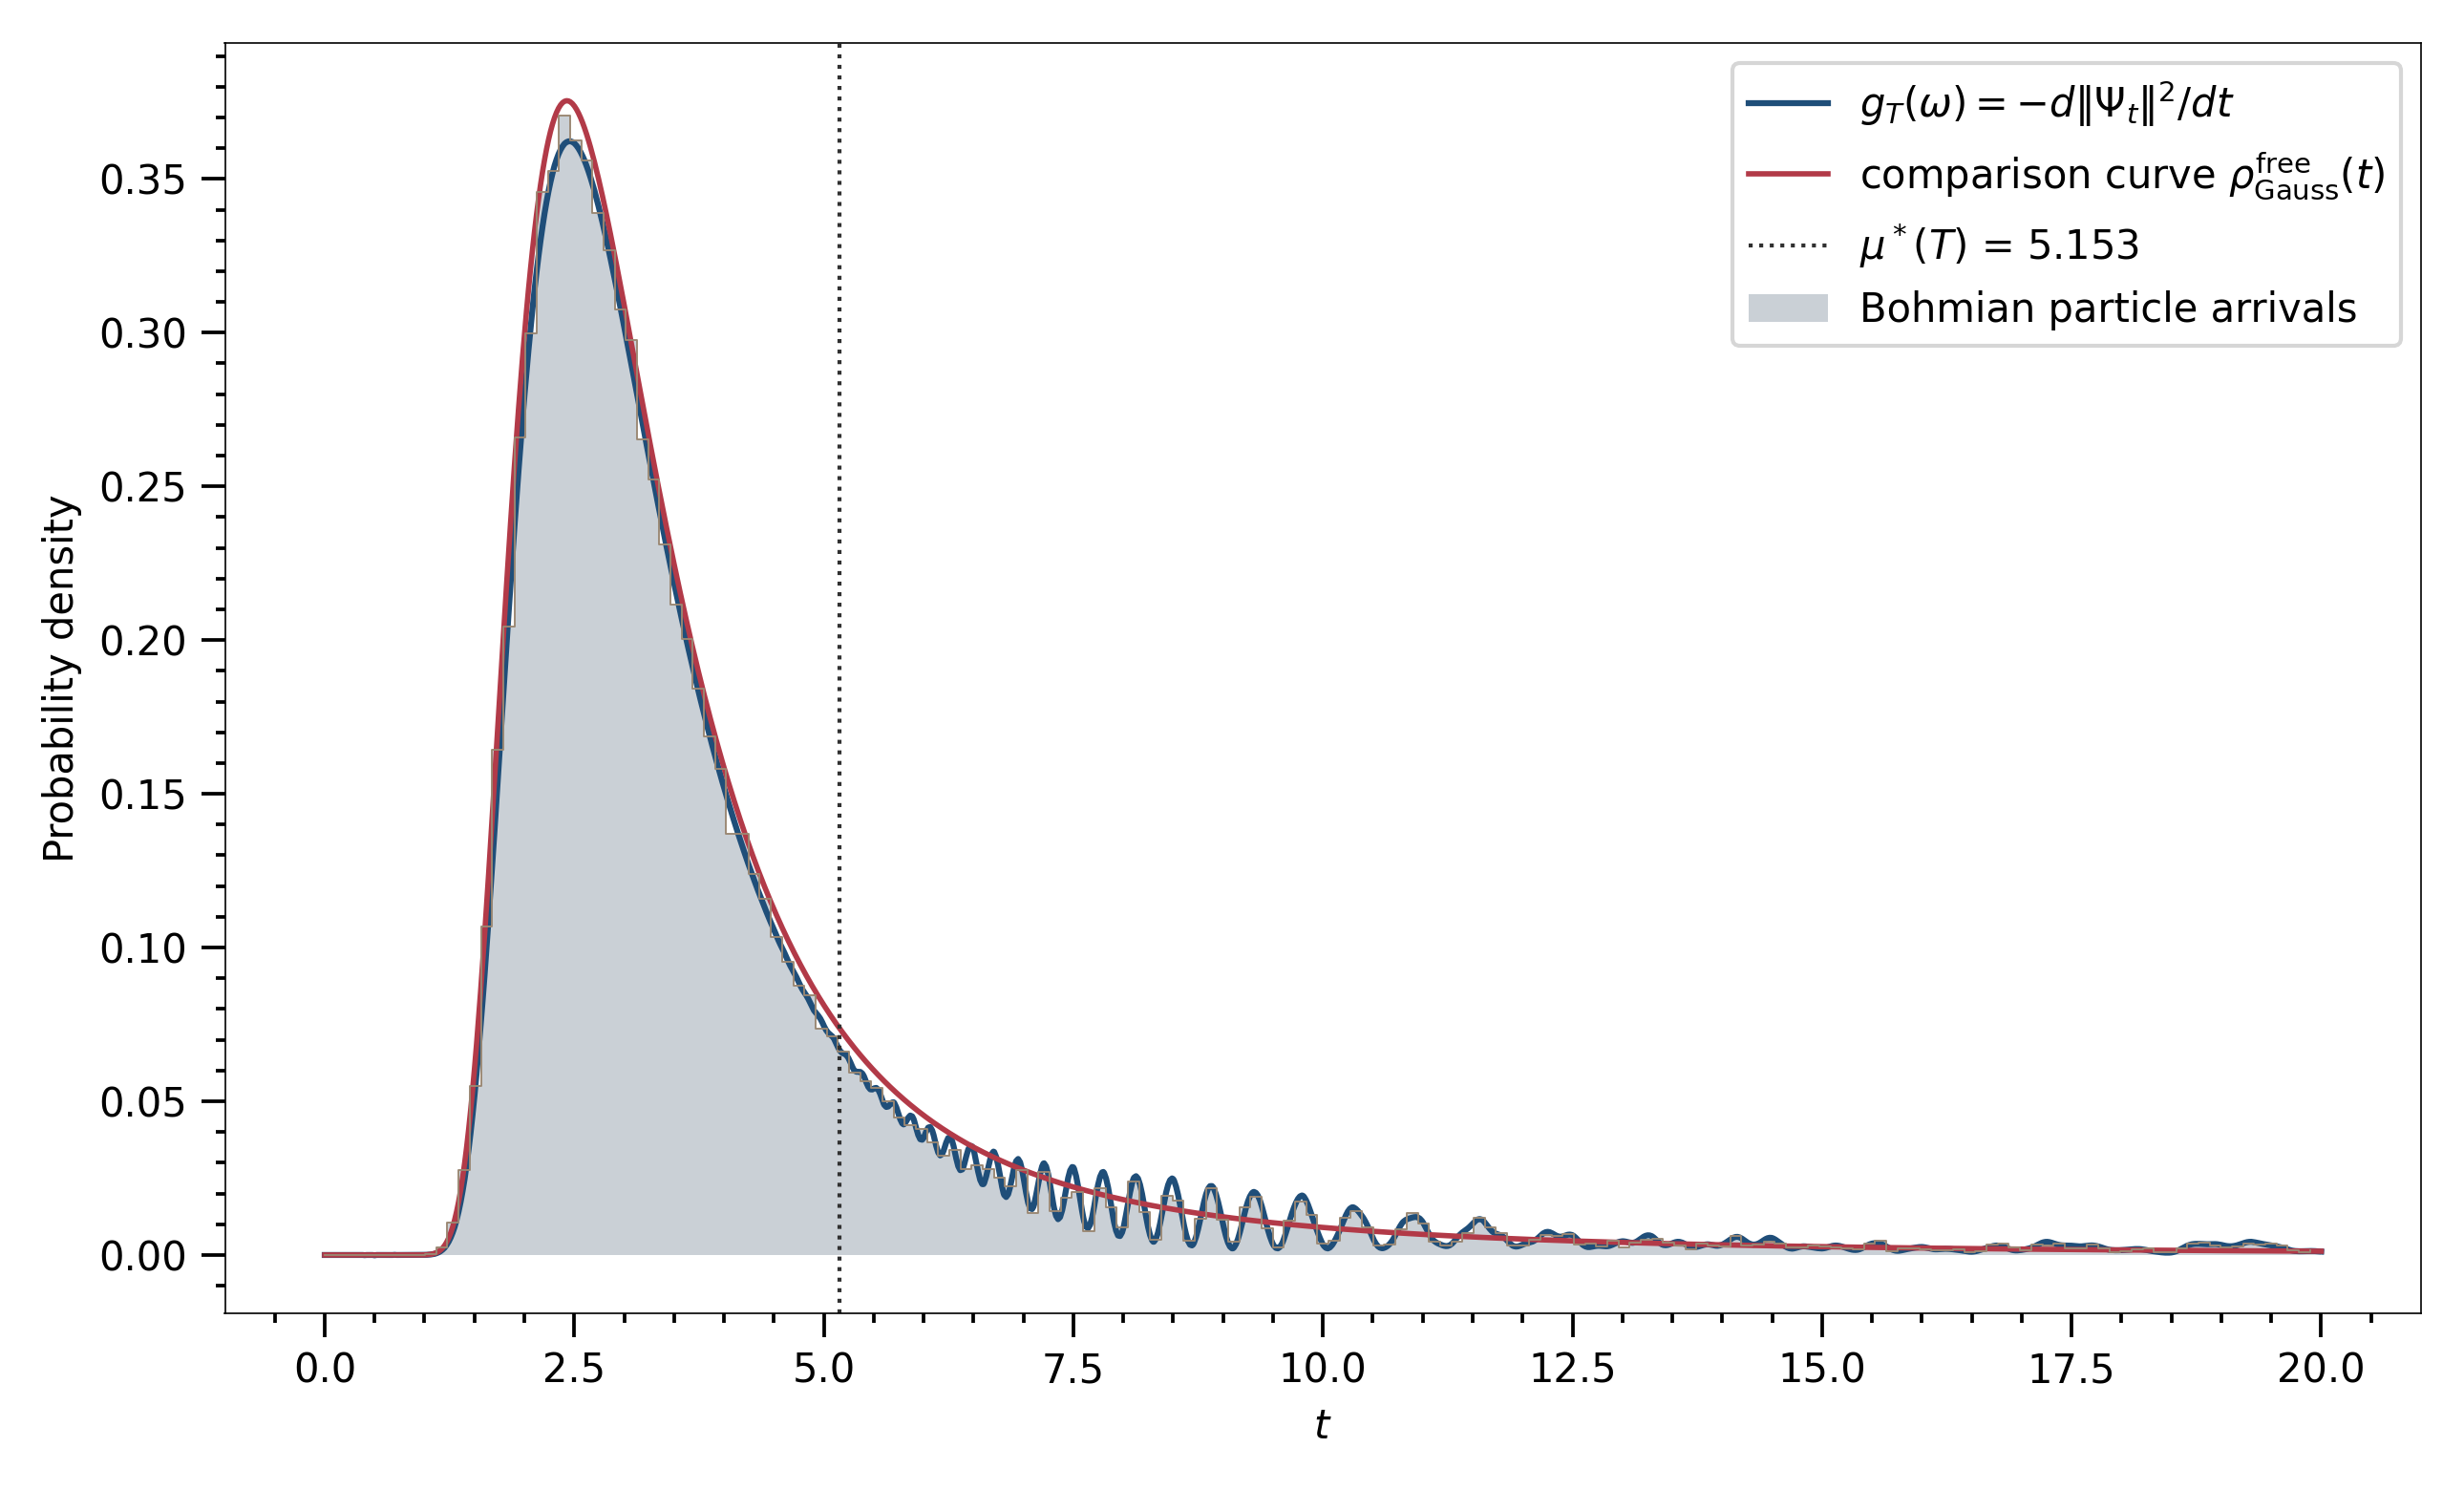}
    \par\vspace{0.3em}
    {\small (c) $\sigma_\parallel=0.5$}
  \end{minipage}\hfill
  \begin{minipage}[t]{0.48\linewidth}
    \centering
    \includegraphics[width=\linewidth]{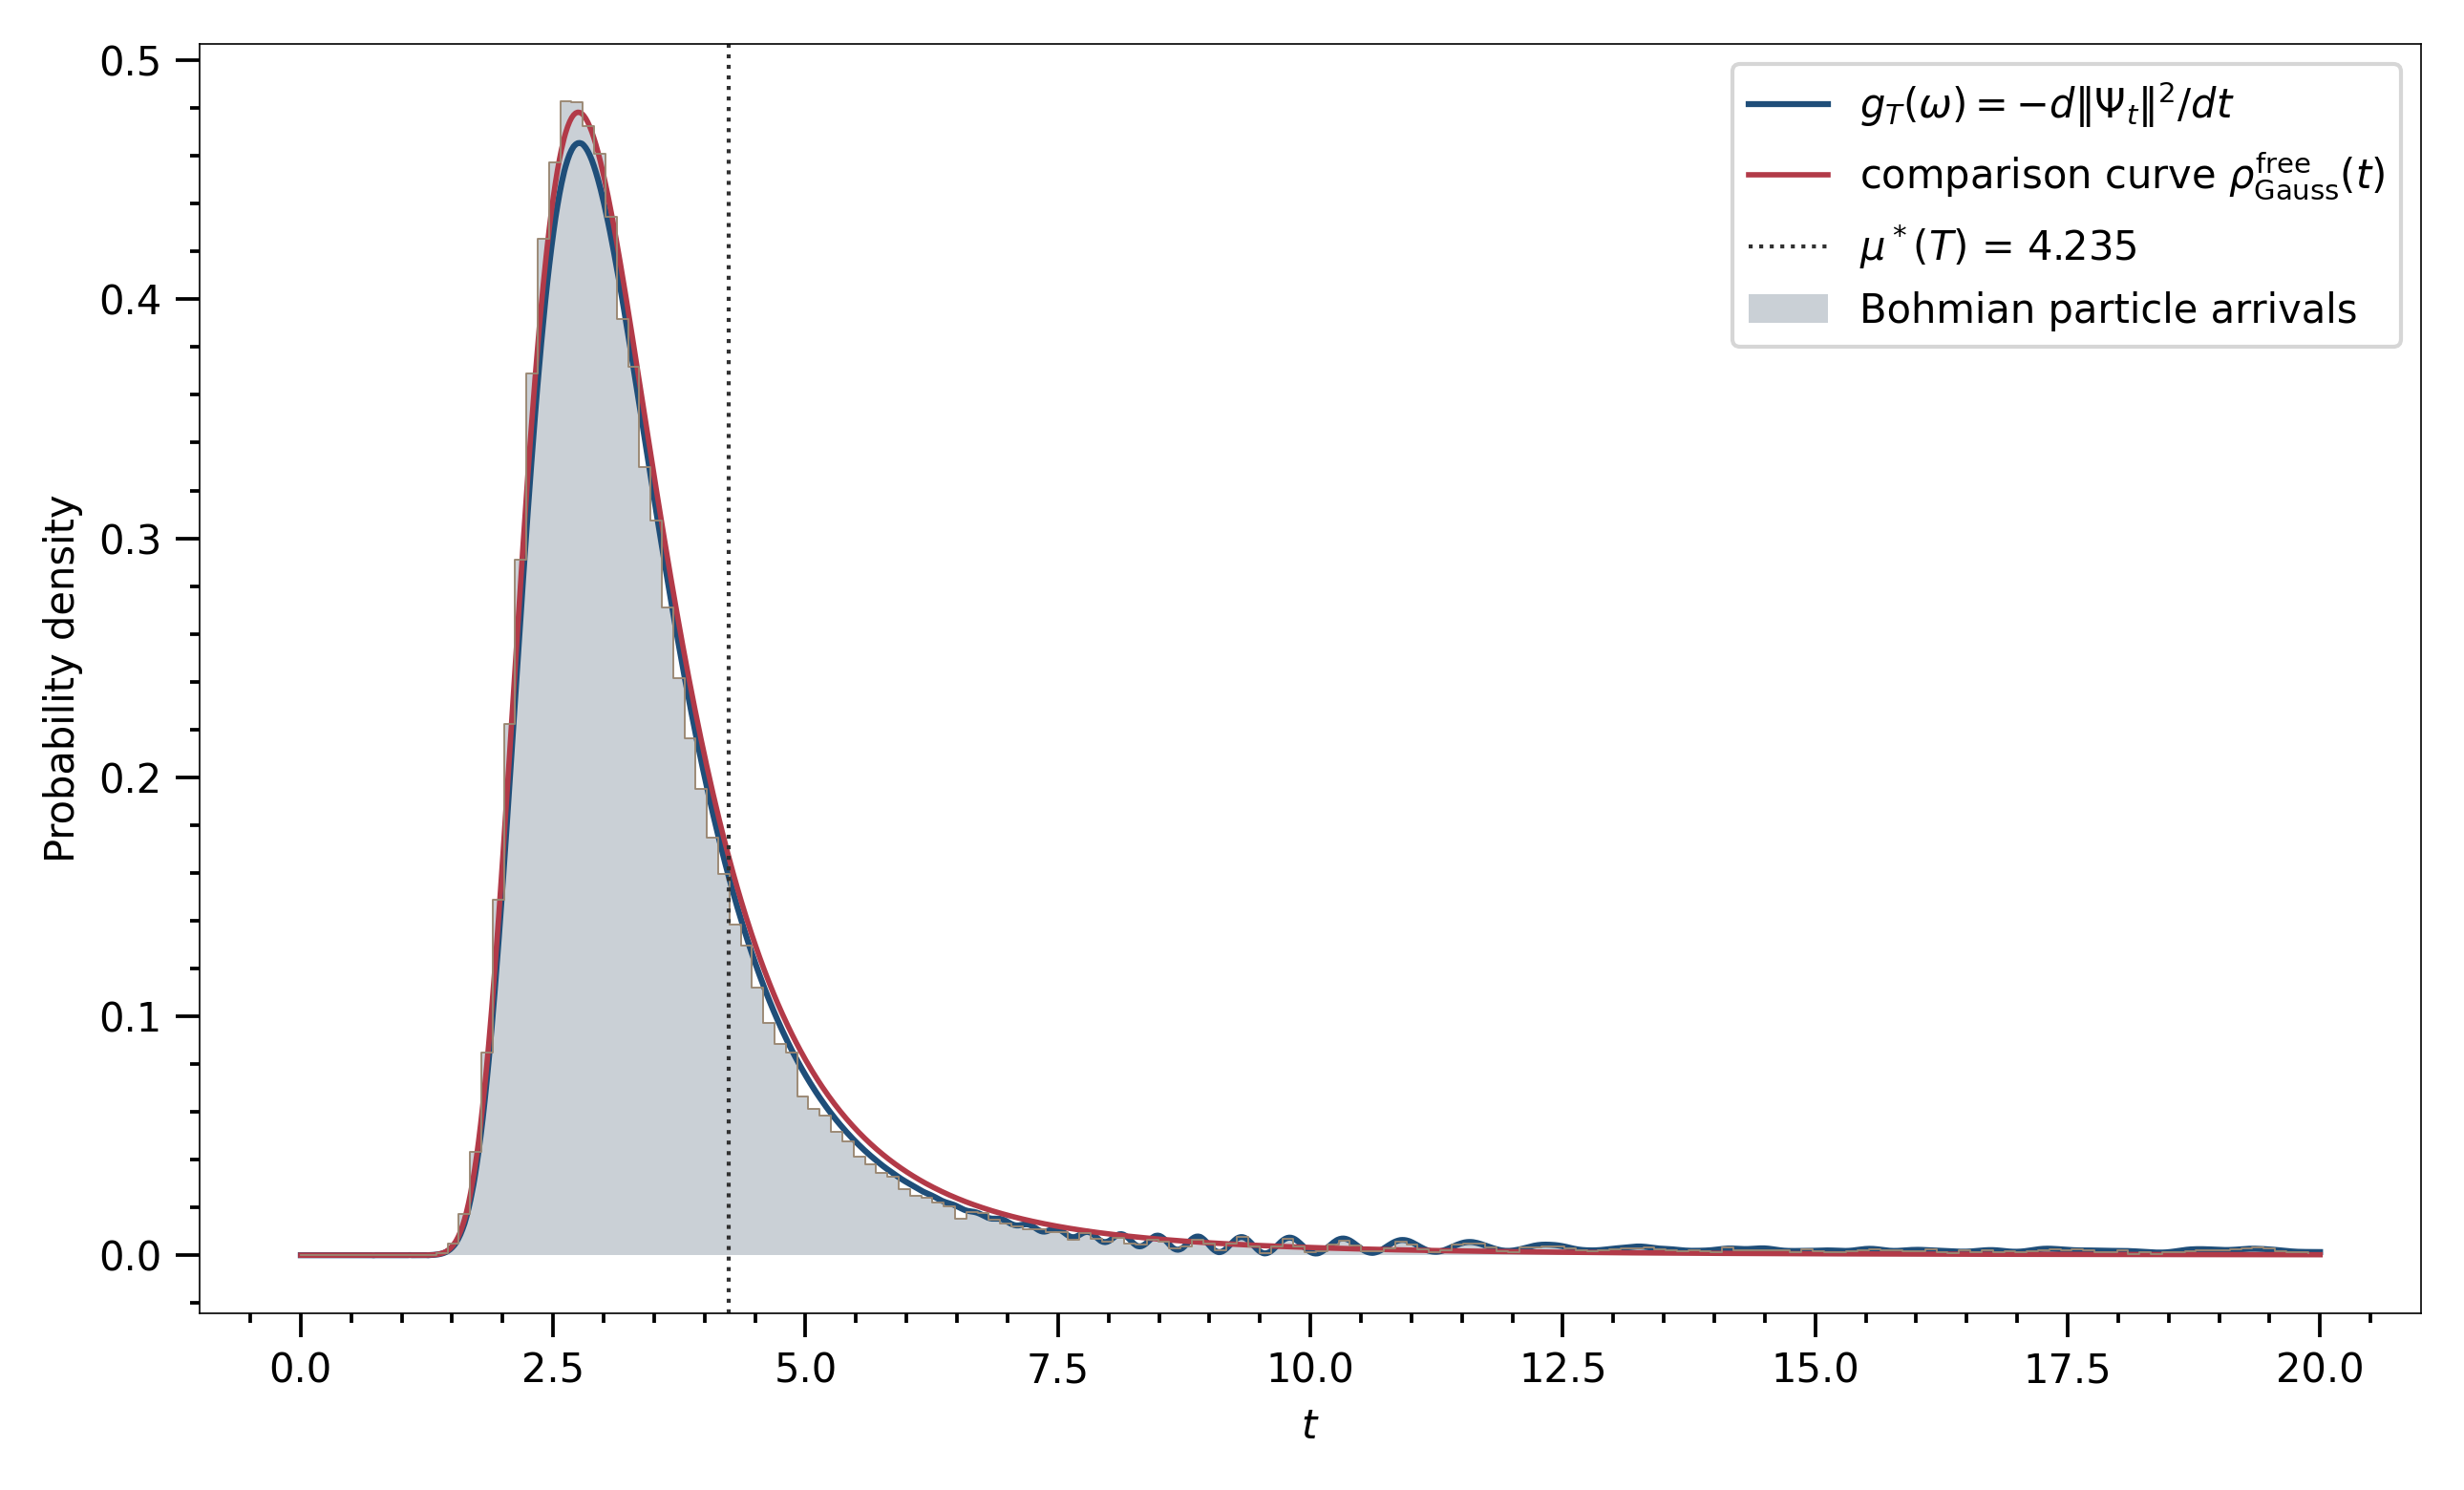}
    \par\vspace{0.3em}
    {\small (d) $\sigma_\parallel=0.75$}
  \end{minipage}
\caption{\(\sigma_\parallel\)-scan for the spinor ABC. The parameters
\(k_z=\kappa=\pi\) and \(\omega=1\) are fixed.}
  \label{fig:SM_sigma_scan}
\end{figure}
For two representative longitudinal widths, the finite-window fits are
\begin{equation}
\mu^*(T;\omega)\simeq A_\sigma+B_\sigma\sqrt{\omega}.
\end{equation}
\begin{table}[H]
\caption{Representative fit coefficients for
\(\mu^*(T;\omega)\simeq A_\sigma+B_\sigma\sqrt{\omega}\), with
\(k_z=\kappa=\pi\) fixed.}
\label{tab:SM_sigmaz_fit}
\begingroup
\small
\setlength{\tabcolsep}{4.0pt}
\renewcommand{\arraystretch}{0.75}
\makebox[\linewidth][c]{%
\begin{minipage}{0.30\linewidth}
\begin{ruledtabular}
\begin{tabular}{@{}c|cc@{}}
\(\sigma_\parallel\) & 0.25 & 0.5 \\
\hline
\(A_\sigma\) & 6.253 & 4.084 \\
\(B_\sigma\) & 0.435 & 0.638
\end{tabular}
\end{ruledtabular}
\end{minipage}%
}
\endgroup
\end{table}

The coefficients change with the source packet, but the approximate
\(\sqrt{\omega}\) trend persists over the finite fitted range.

\subsection{\texorpdfstring{\(k_z\)-scan}{k-z scan}}
\label{subsec:SM_kz_scan}

Changing \(k_z\) mainly changes the bulk flight-time scale and the longitudinal
matching to the detector. For small \(k_z\), the incoming packet is slow and the
fixed boundary parameter \(\kappa=\pi\) is strongly mismatched; the roof-flux
density is broad and the late oscillatory sector is prominent. For larger
\(k_z\), the first roof encounter occurs earlier and the finite-window statistic
decreases. Thus \(k_z\) changes effective prefactors and tail structure, while
the transverse-confinement mechanism remains the boundary scale
\(R=|\boldsymbol\xi|\sim\sqrt{\omega}\).

\begin{figure}[H]
  \centering
  \begin{minipage}[t]{0.48\linewidth}
    \centering
    \includegraphics[width=\linewidth]{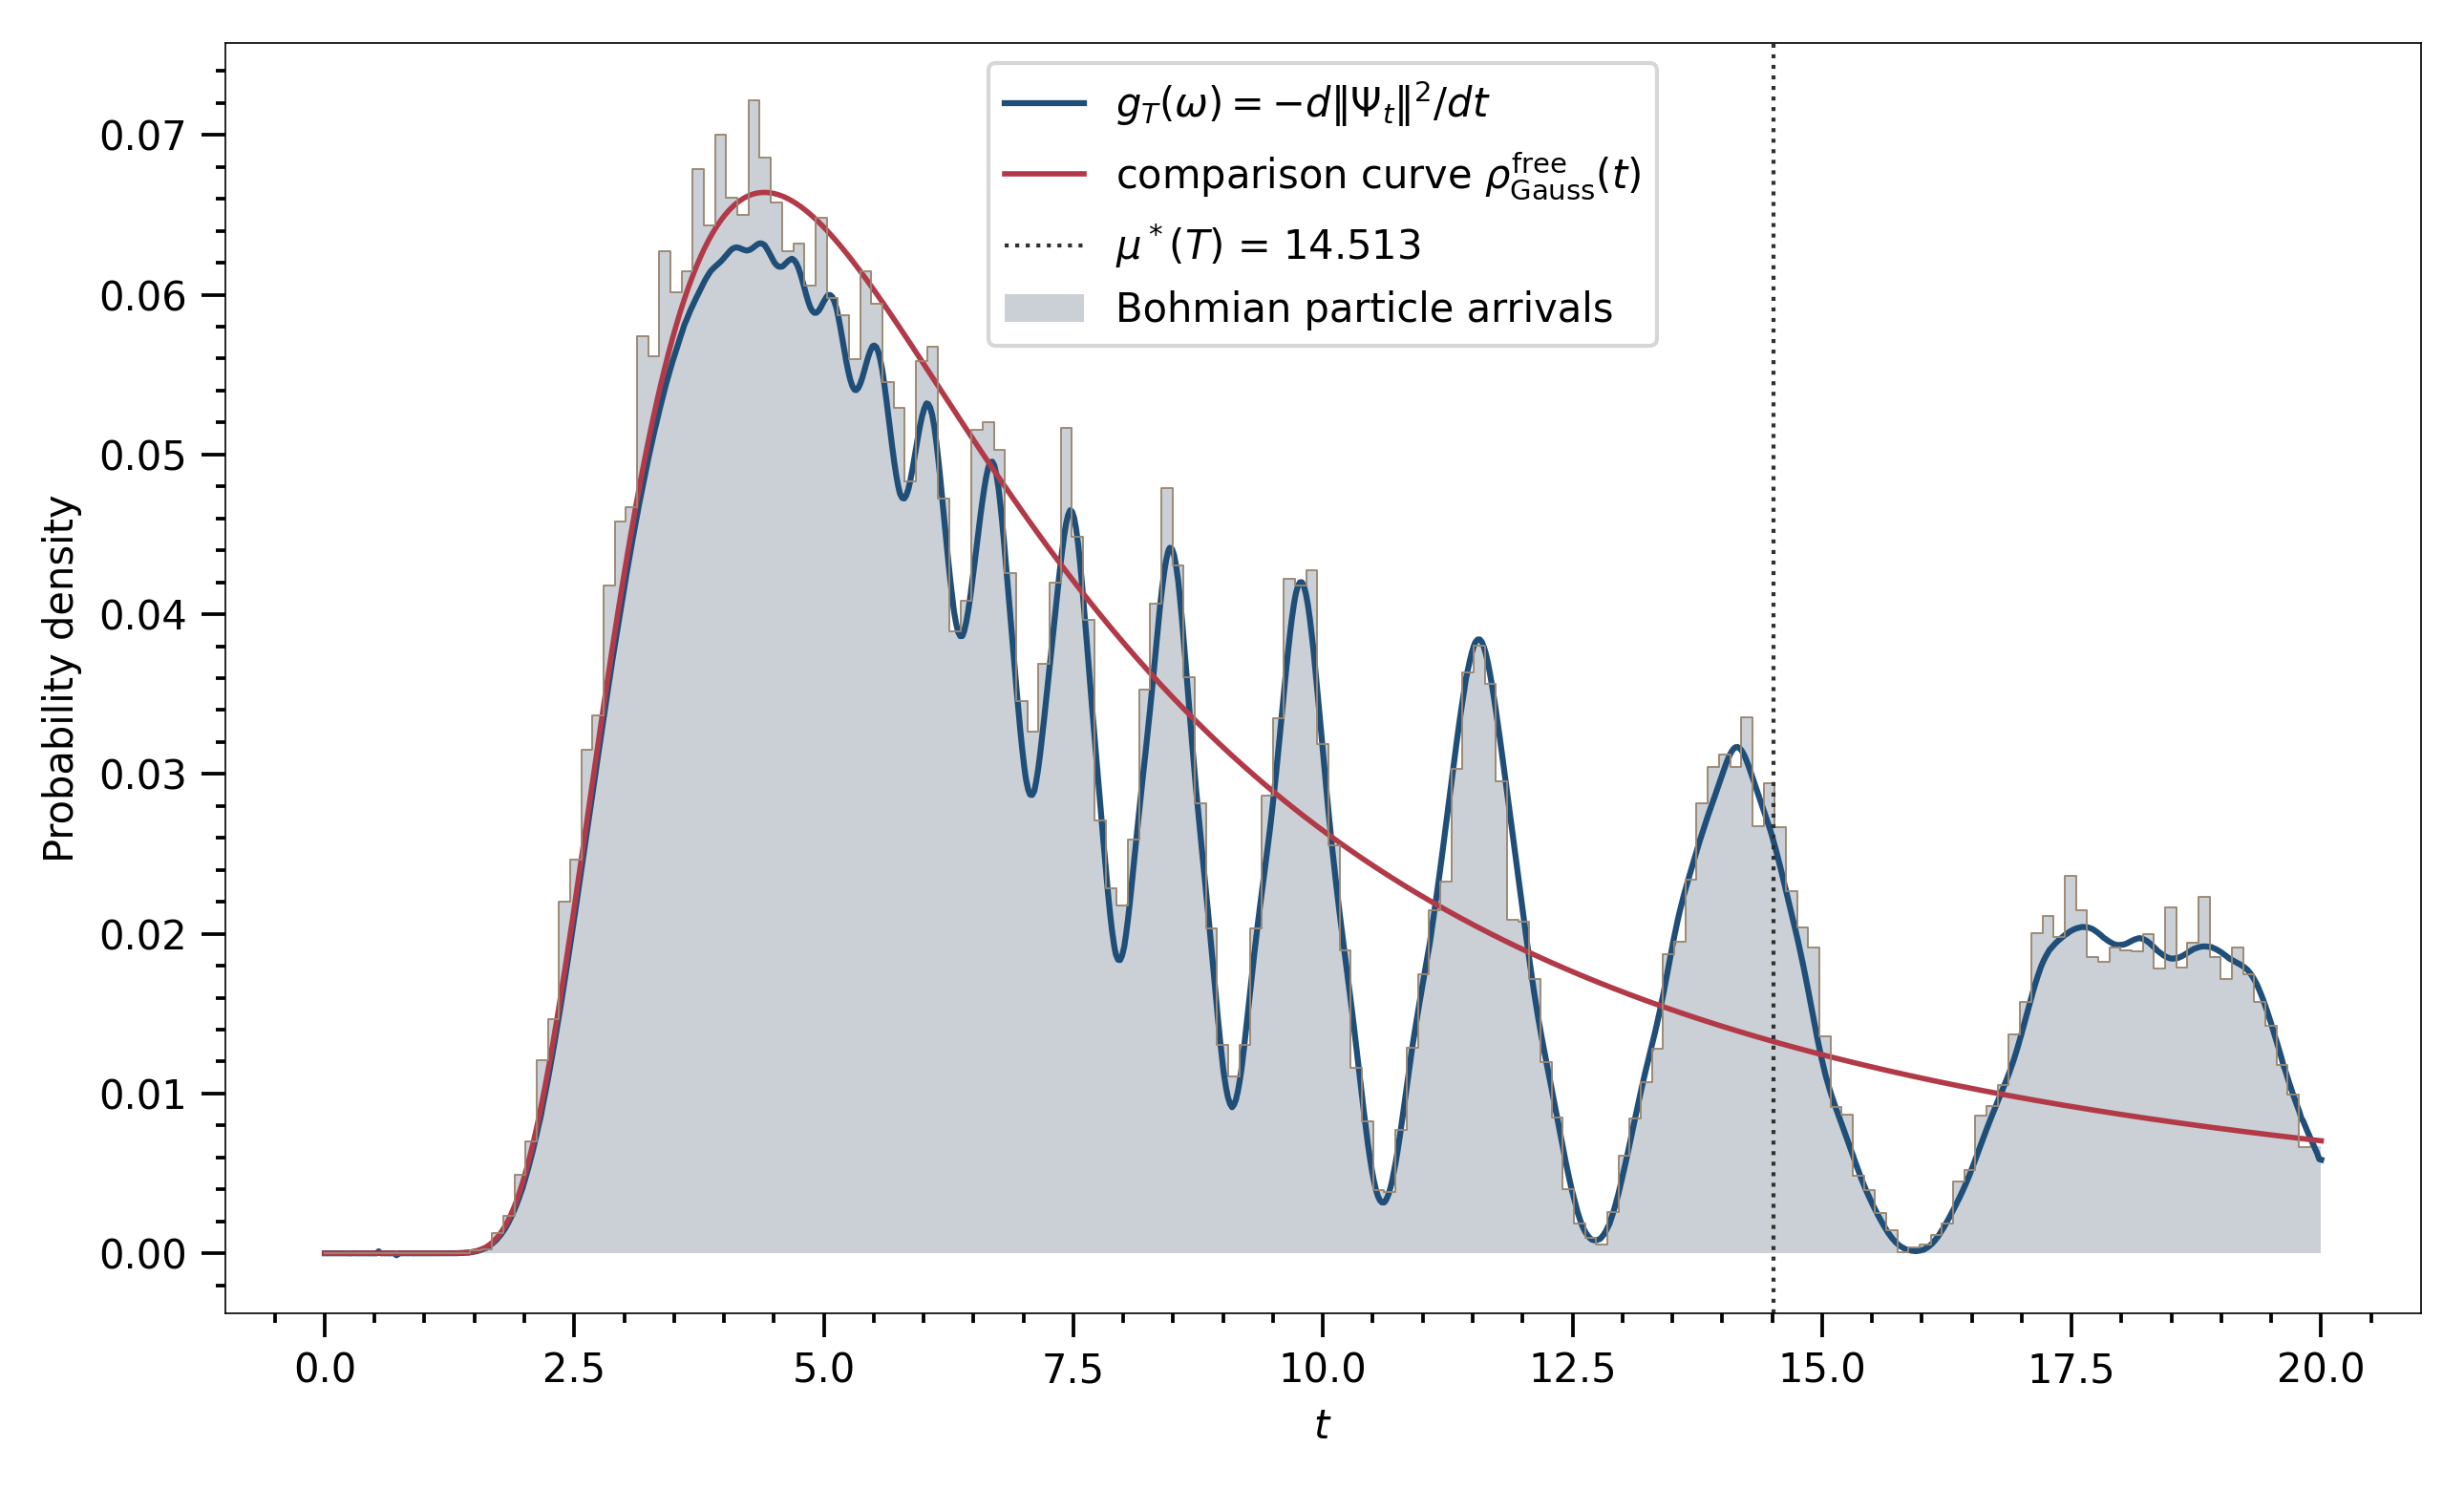}
    \par\vspace{0.3em}
    {\small (a) $k_z=0.5$}
  \end{minipage}\hfill
  \begin{minipage}[t]{0.48\linewidth}
    \centering
    \includegraphics[width=\linewidth]{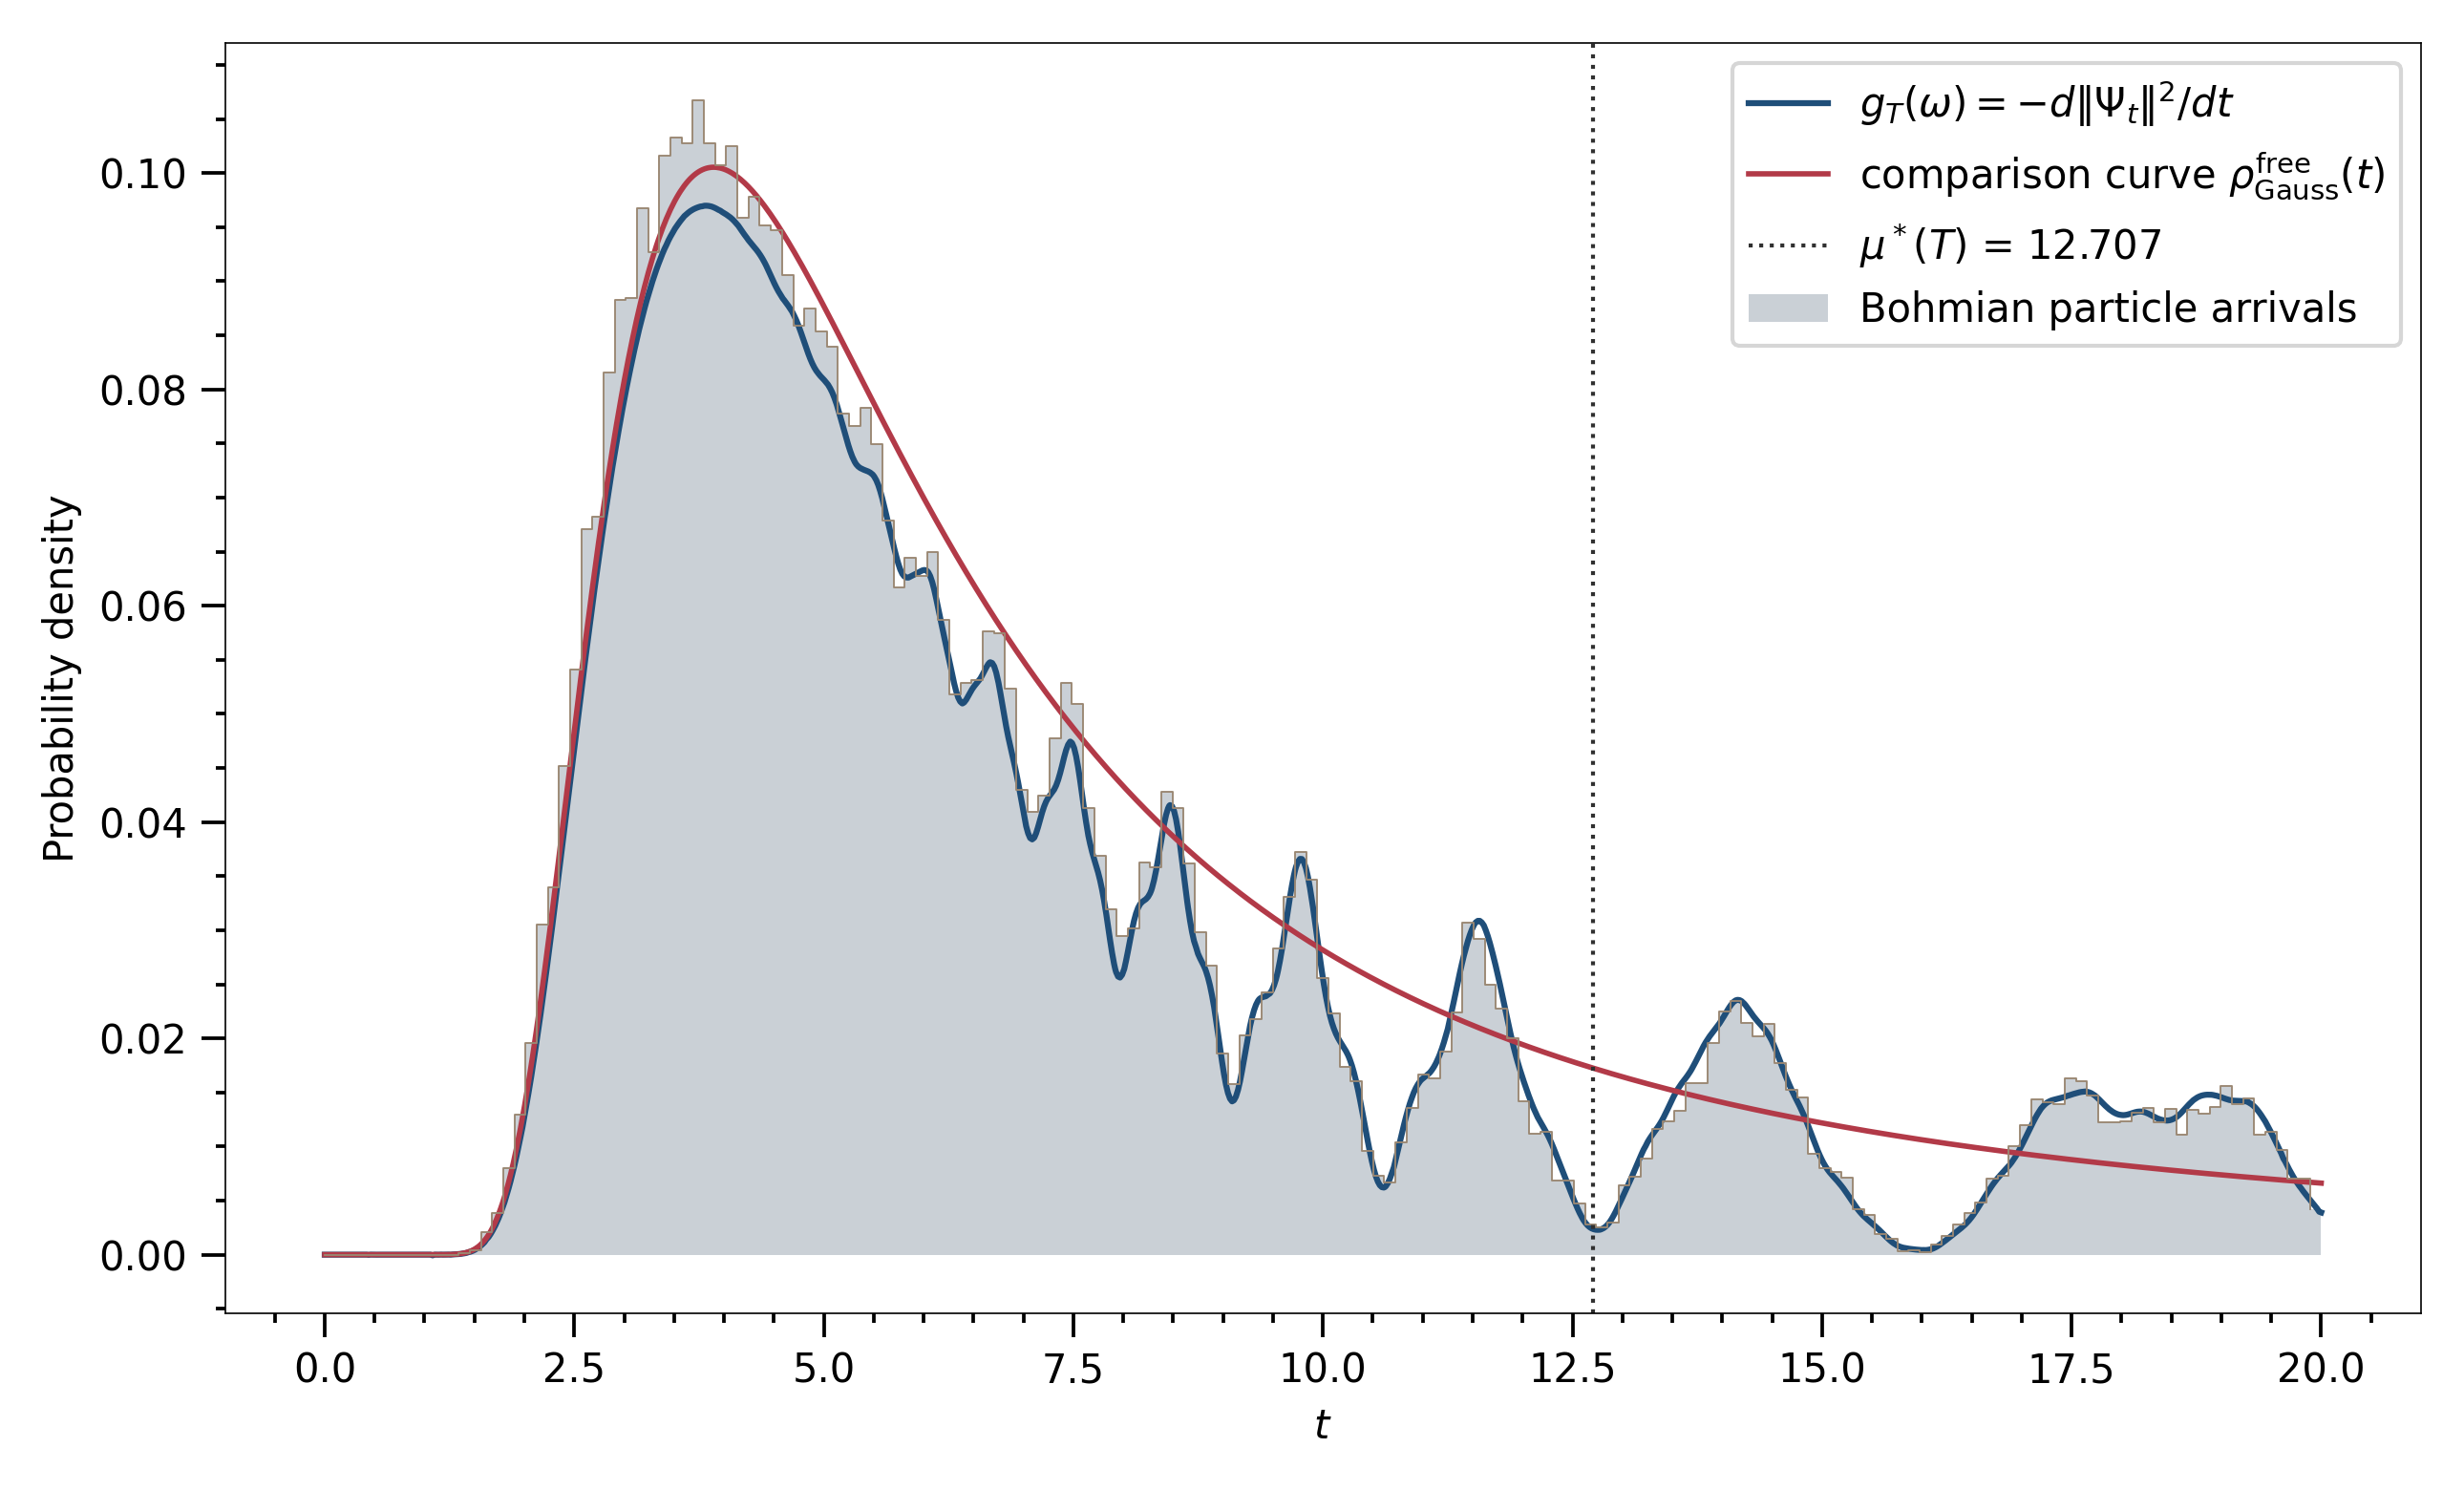}
    \par\vspace{0.3em}
    {\small (b) $k_z=1$}
  \end{minipage}

  \vspace{0.8em}

  \begin{minipage}[t]{0.48\linewidth}
    \centering
    \includegraphics[width=\linewidth]{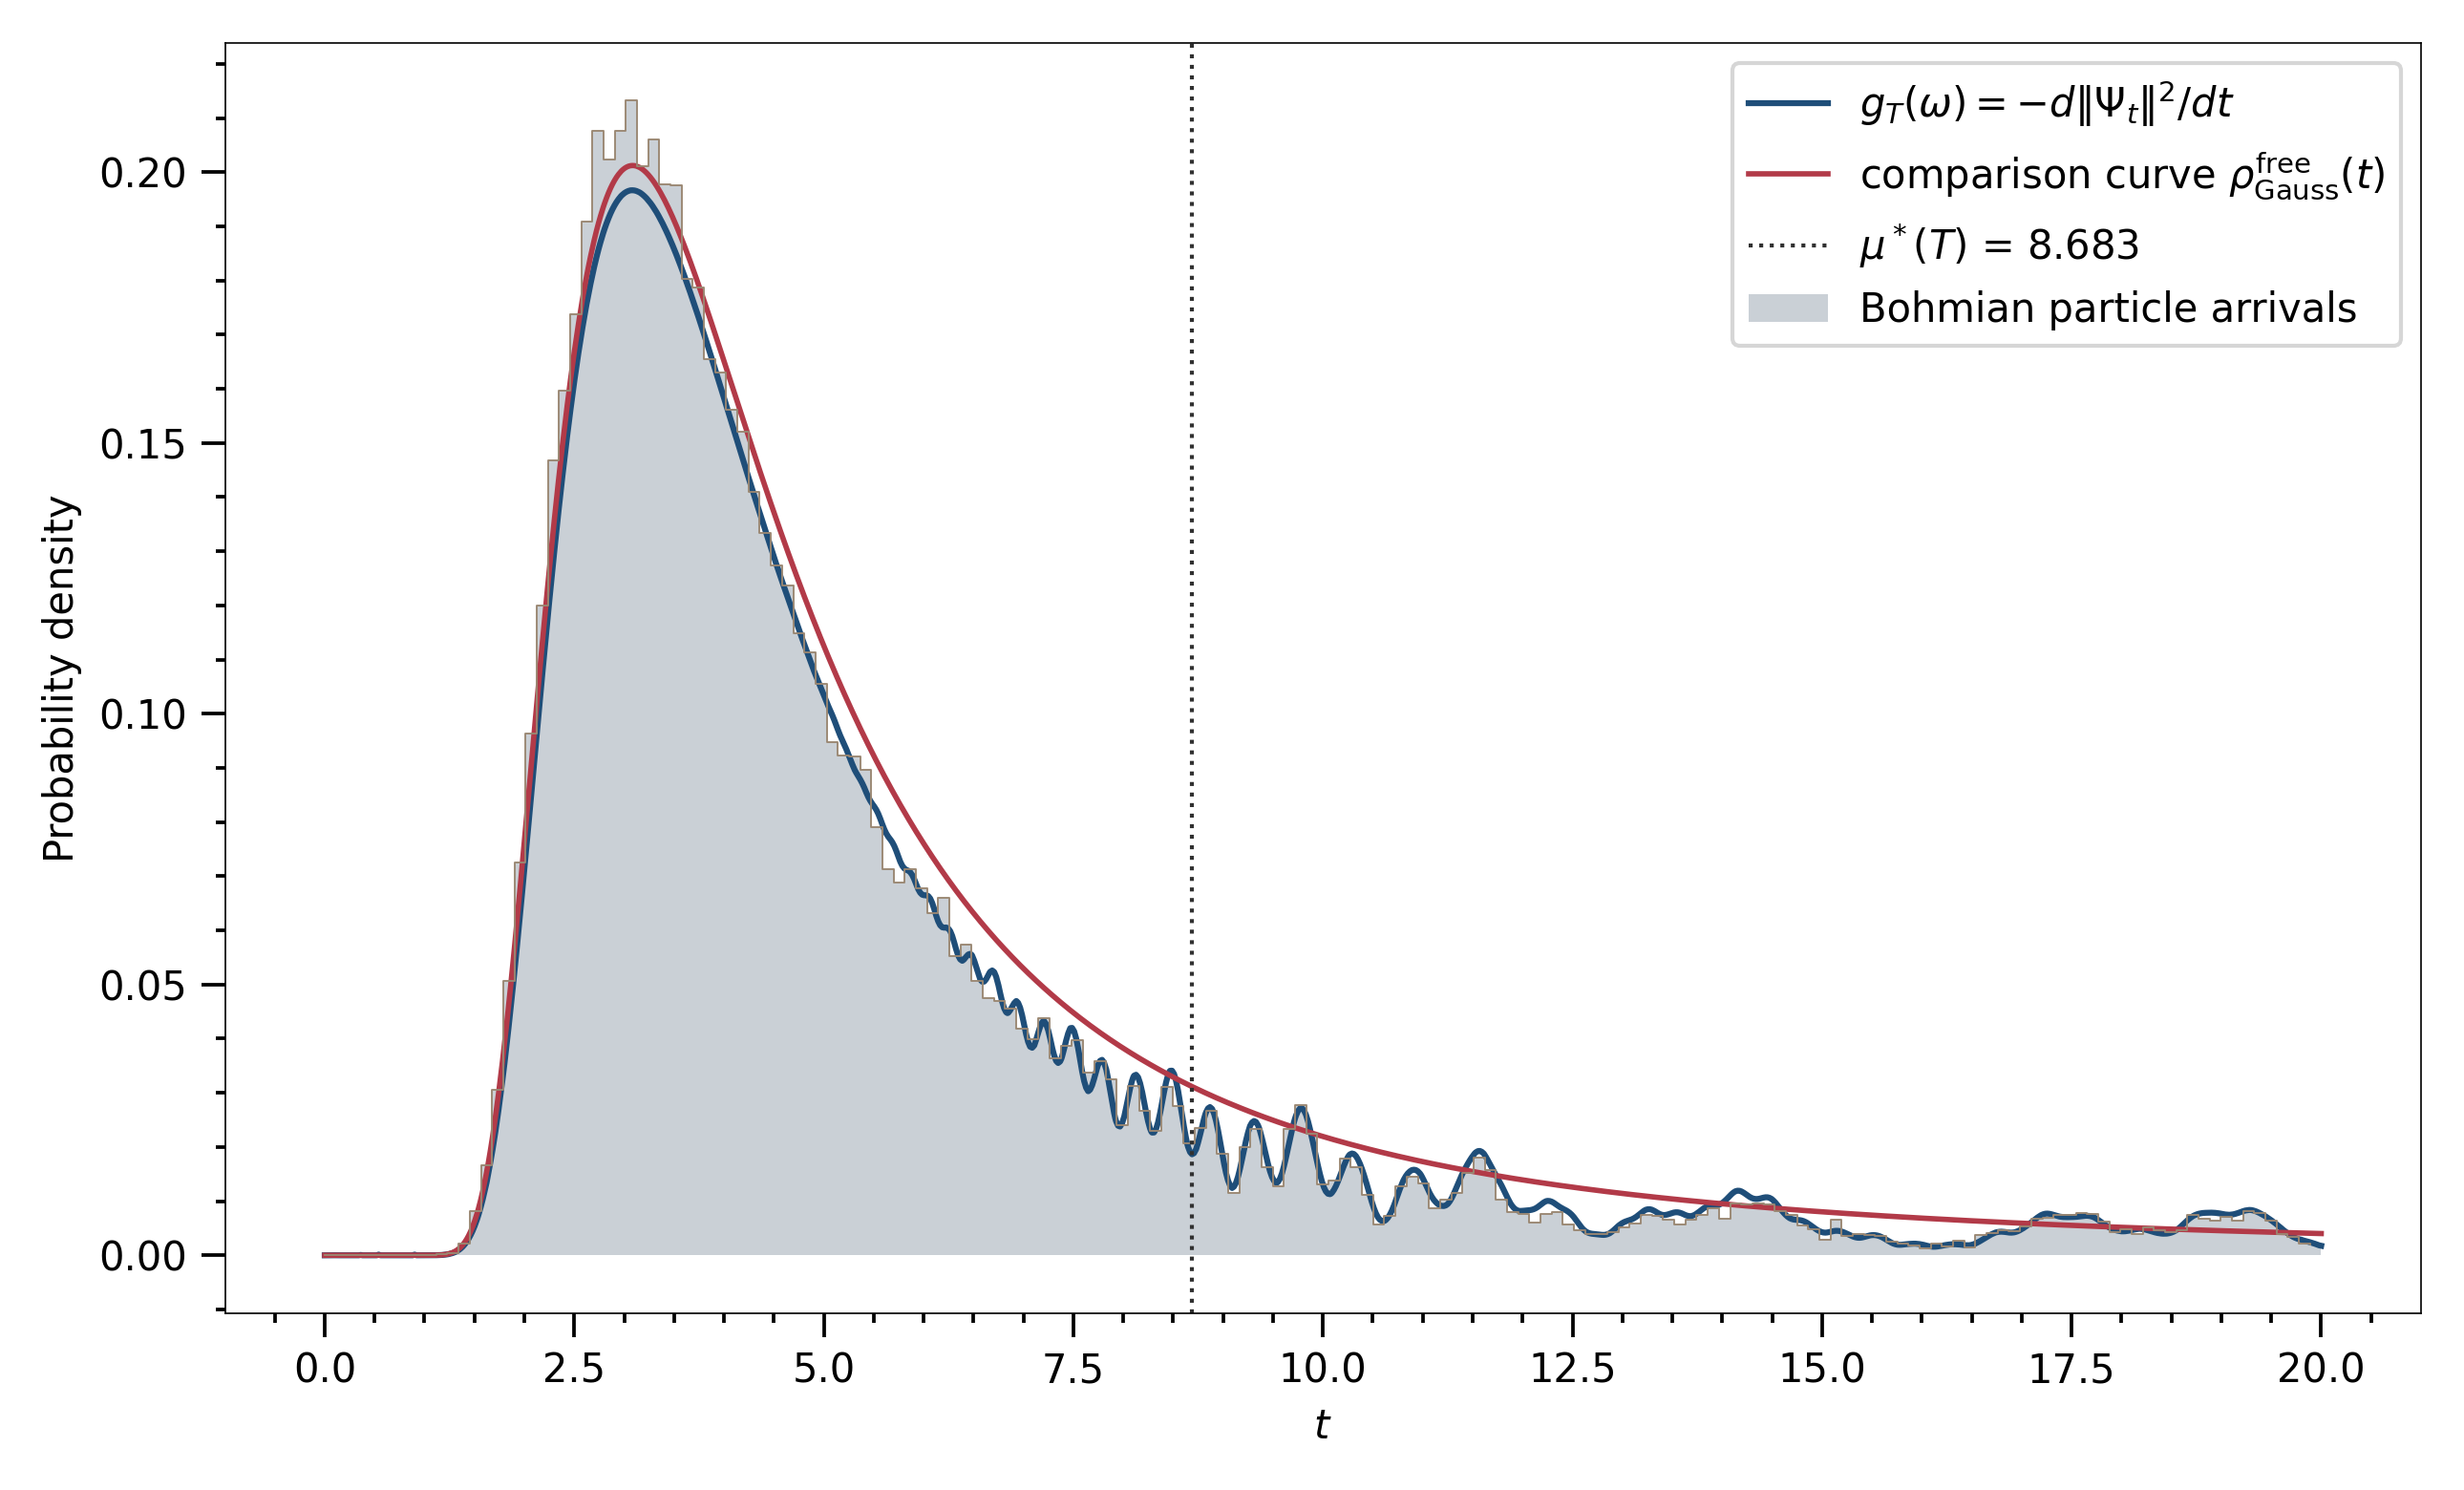}
    \par\vspace{0.3em}
    {\small (c) $k_z=2$}
  \end{minipage}\hfill
  \begin{minipage}[t]{0.48\linewidth}
    \centering
    \includegraphics[width=\linewidth]{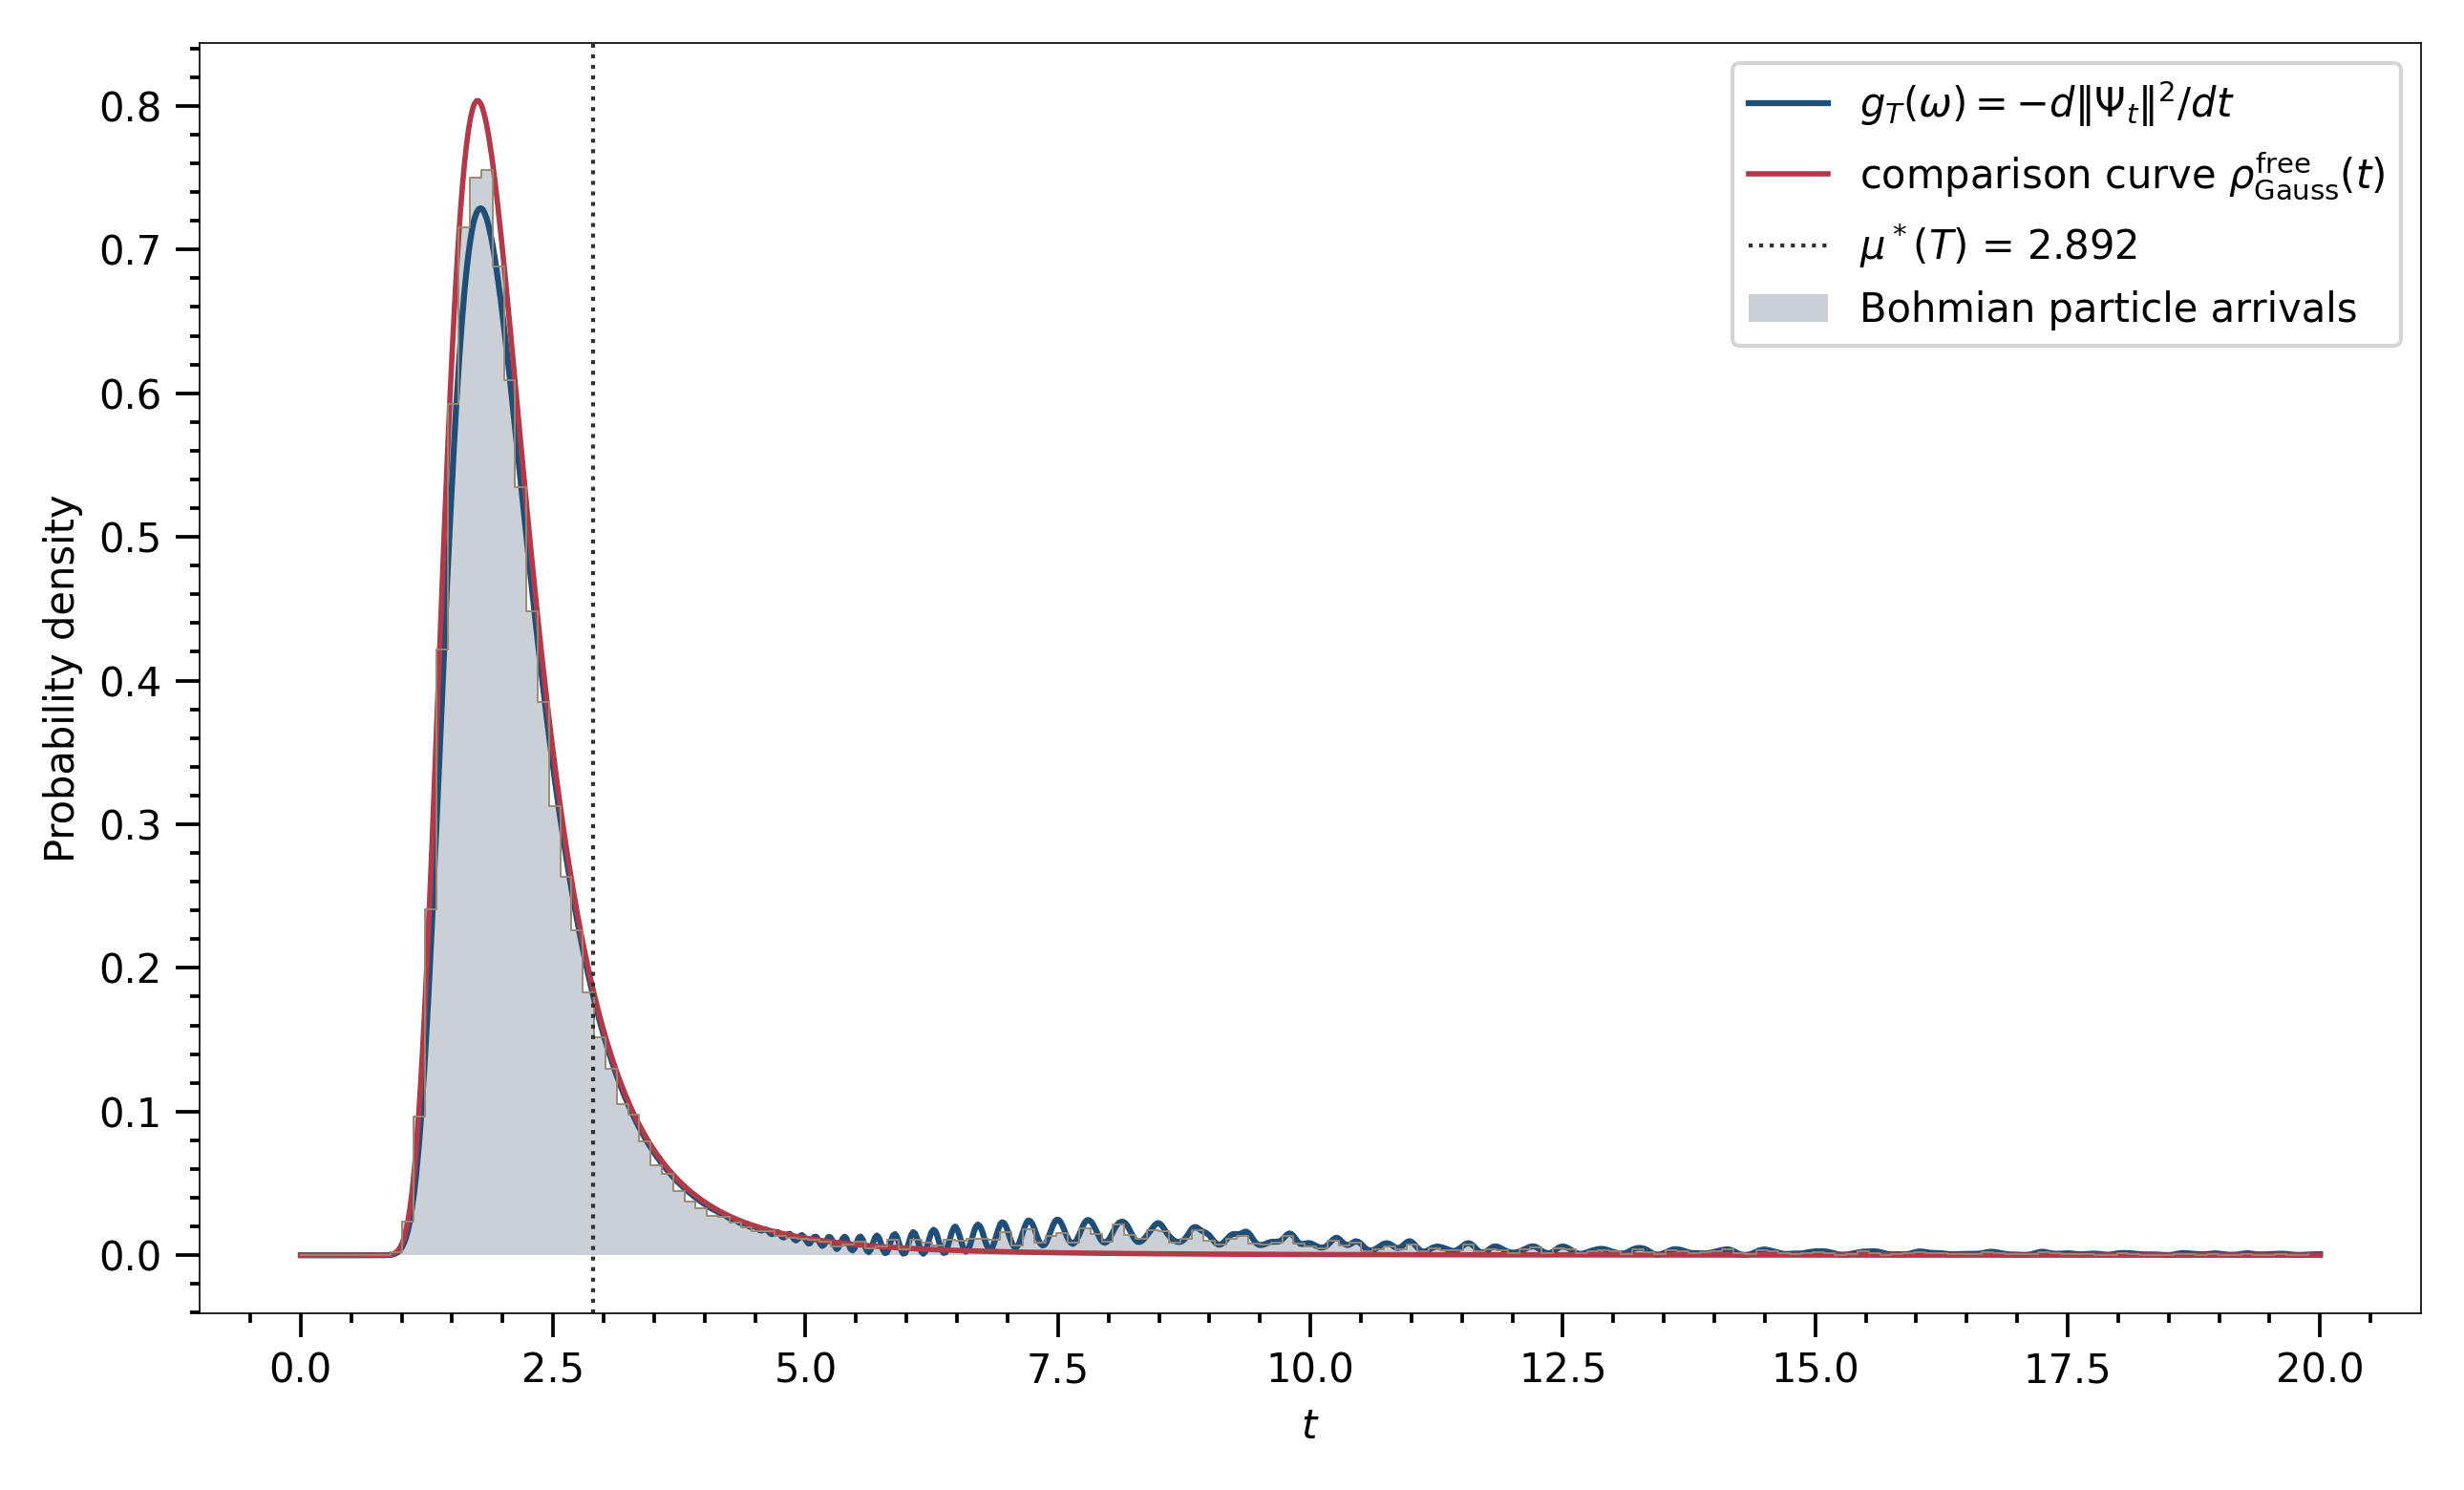}
    \par\vspace{0.3em}
    {\small (d) $k_z=5$}
  \end{minipage}
\caption{\(k_z\)-scan for the spinor ABC. The parameters \(\kappa=\pi\),
\(\sigma_\parallel=0.5\), and \(\omega=1\) are fixed.}
  \label{fig:SM_kz_scan}
\end{figure}

\subsection{Large-box check}
\label{subsec:SM_large_box}

We repeated representative spinor-ABC runs in a longer box, \(L_z=100\), with
\(z_c=50\), \(k_z=\kappa=\pi\), and \(\sigma_\parallel=0.5\). Increasing \(\omega\) again
suppresses the prompt roof-flux peak and enhances a delayed oscillatory sector.
Thus the confinement-induced delayed sector is not only a short-box artifact.

\begin{figure}[H]
  \centering
  \begin{minipage}[t]{0.48\linewidth}
    \centering
    \includegraphics[width=\linewidth]{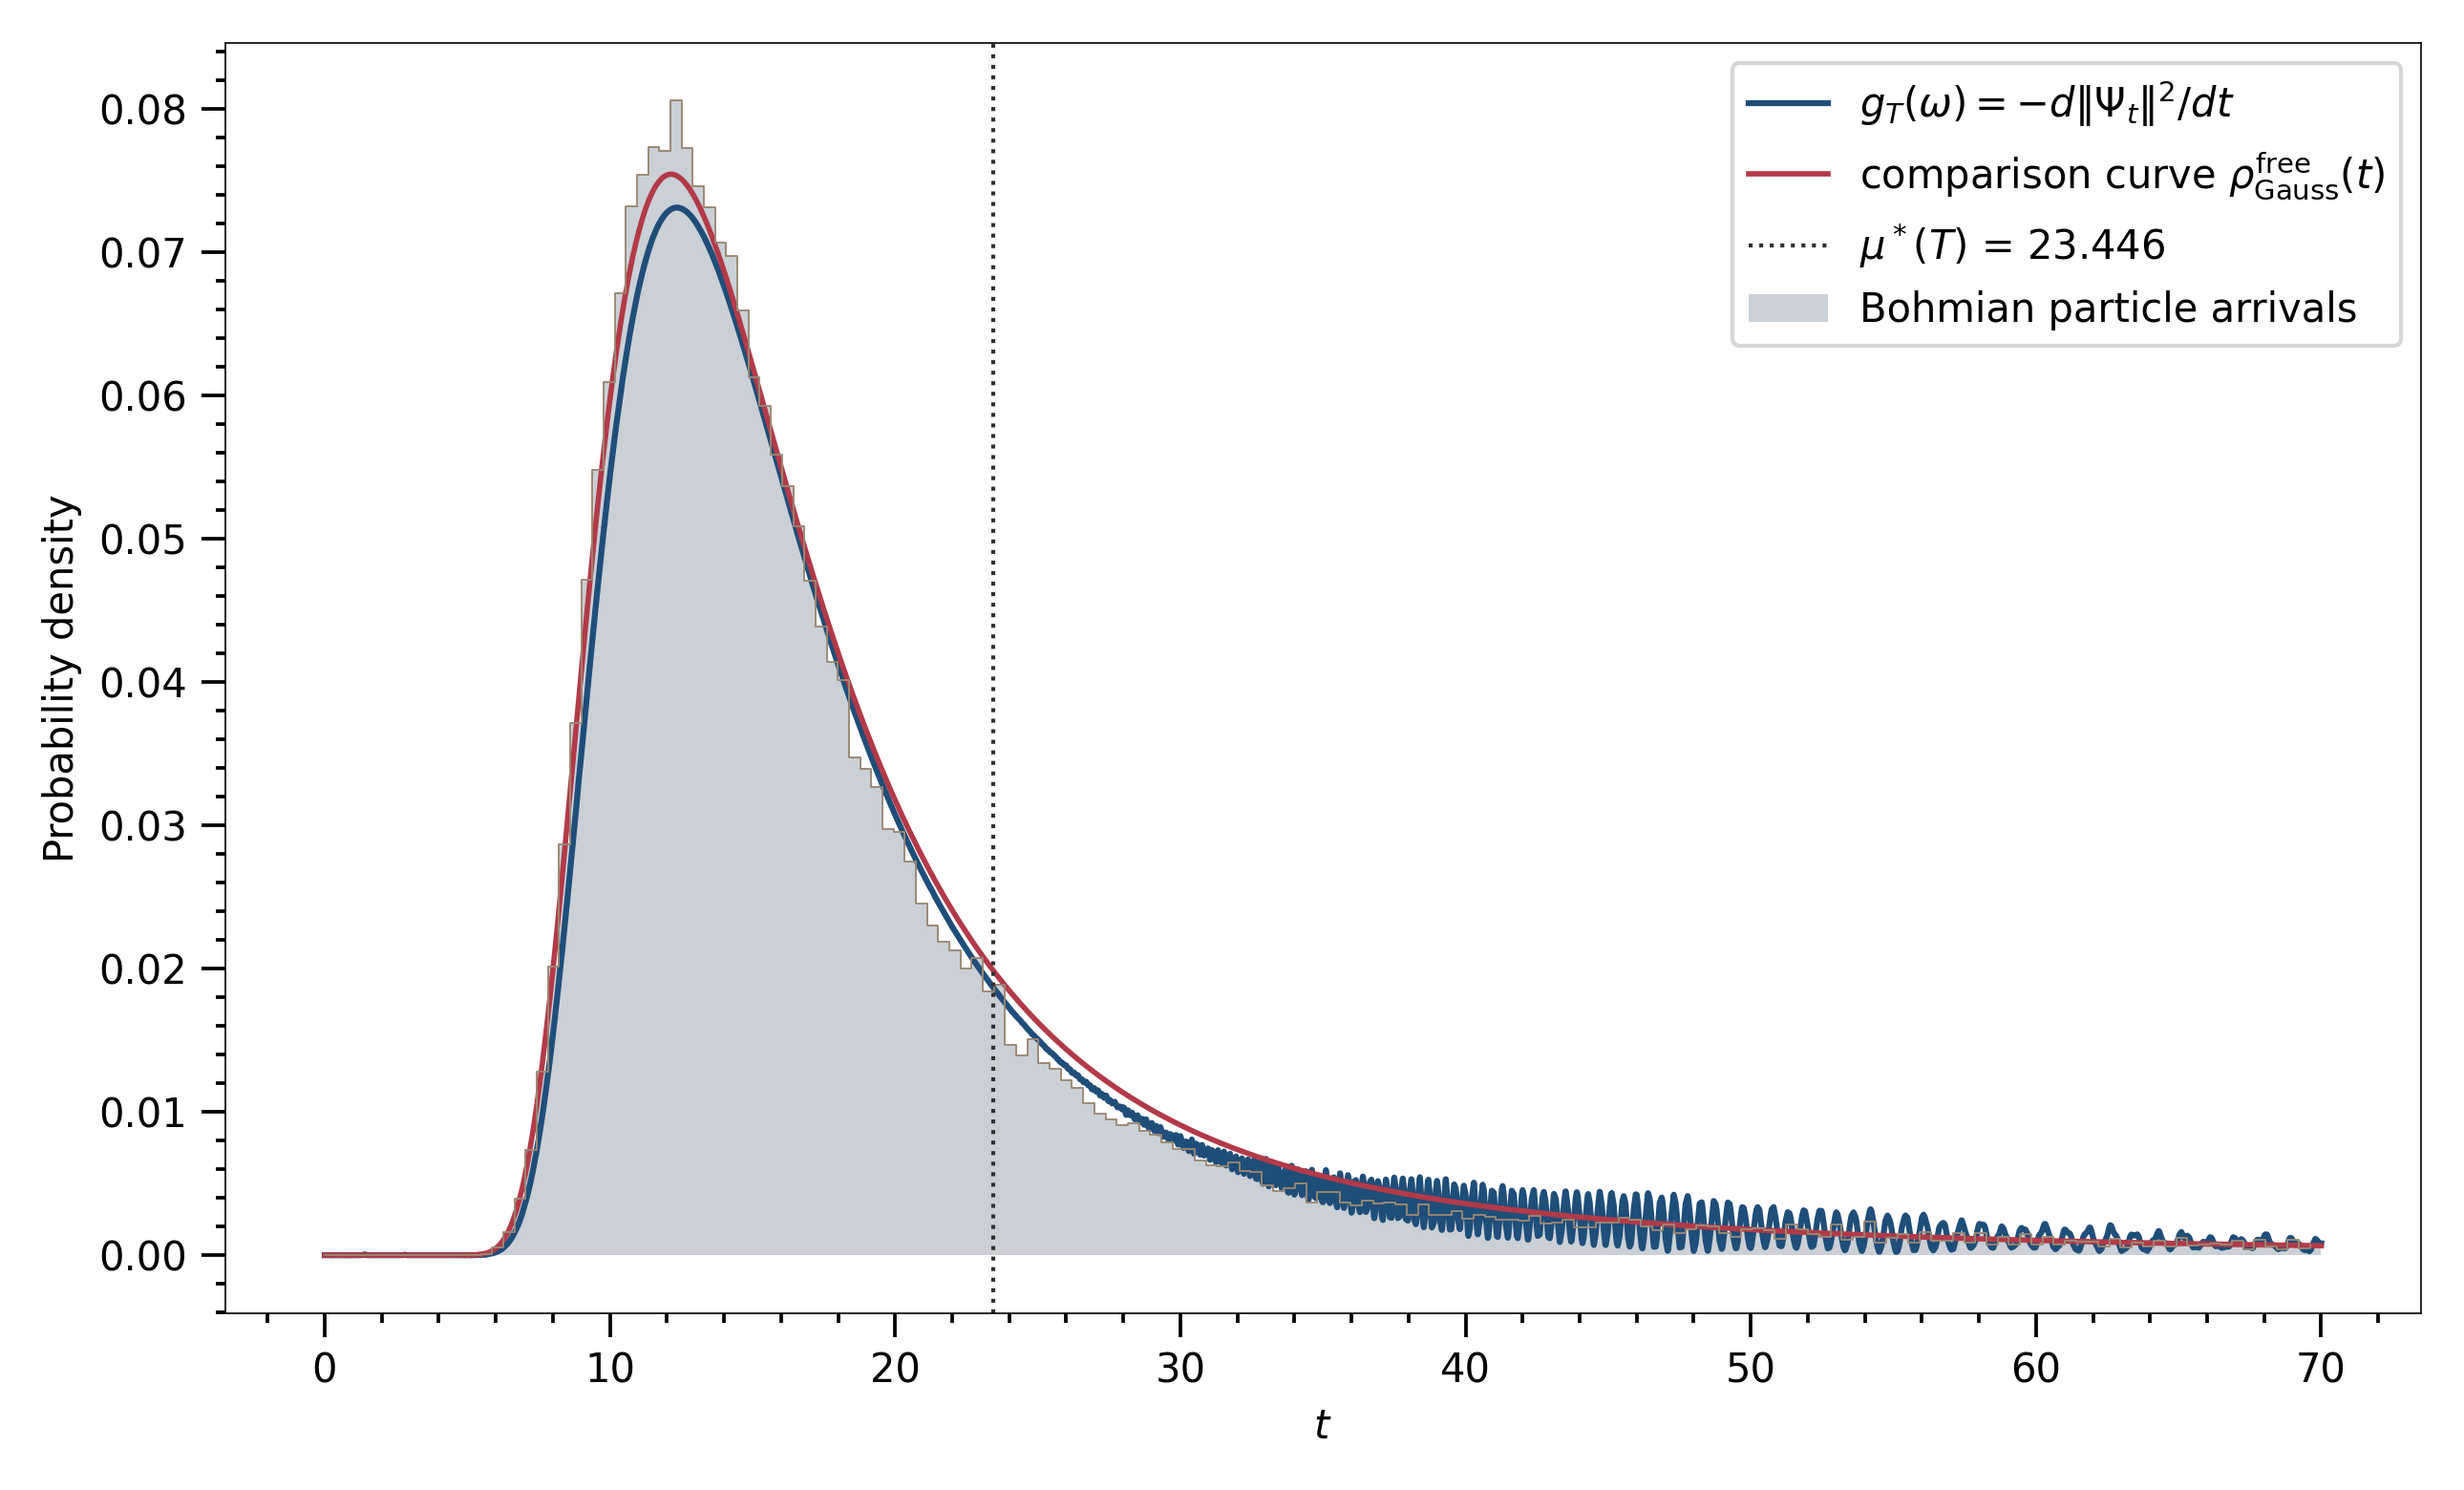}
    \par\vspace{0.3em}
    {\small (a) $\omega=1$}
  \end{minipage}\hfill
  \begin{minipage}[t]{0.48\linewidth}
    \centering
    \includegraphics[width=\linewidth]{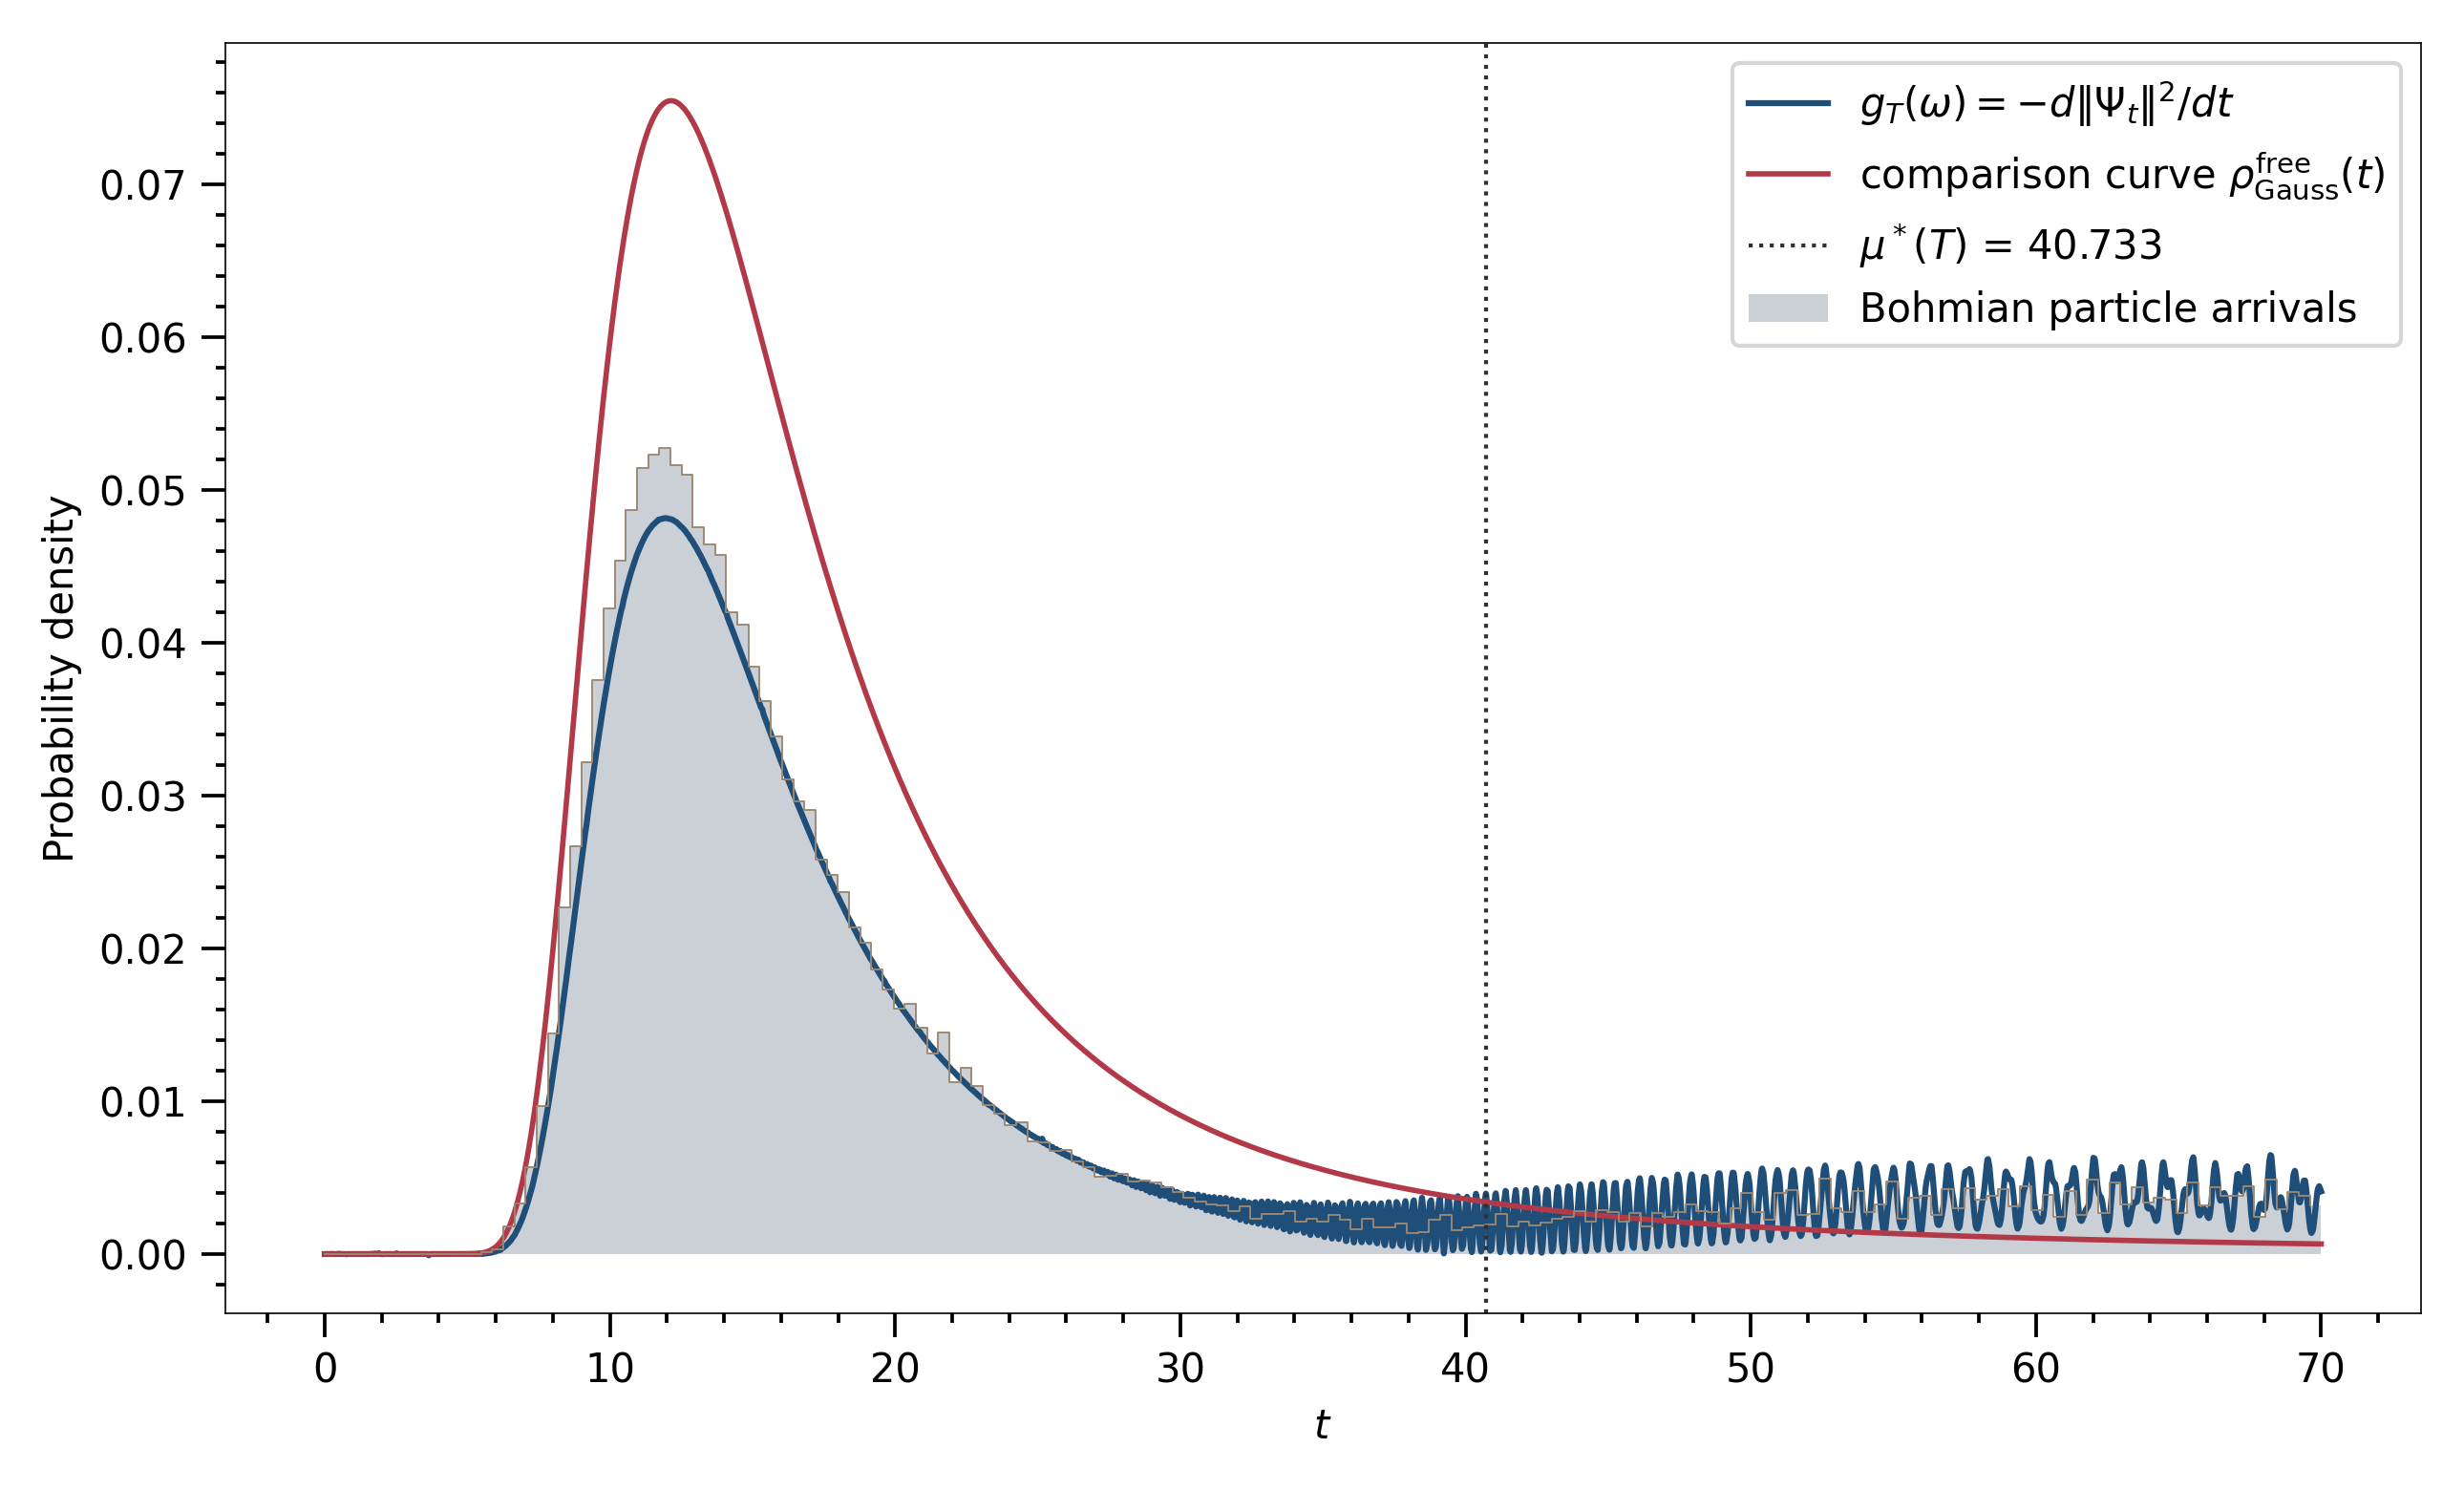}
    \par\vspace{0.3em}
    {\small (b) $\omega=100$}
  \end{minipage}
\caption{Large-box spinor-ABC check. Only \(\omega\) is varied; the delayed sector persists.}
  \label{fig:SM_large_box}
\end{figure}

Overall, the scans show that source and detector parameters change the numerical
coefficients, detected fractions, and detailed oscillatory tails. They do not
alter the local origin of the confinement dependence:
\begin{equation}
        R=|\boldsymbol\xi|\sim\sqrt{\omega}.
\end{equation}

\section{Physical scales}
\label{sec:SM_physical_scales}

The analysis above is dimensionless. Let \(a_0\) be the physical length represented by one dimensionless unit. Then
\begin{equation}
r_{\rm phys}=a_0 r,\qquad t_{\rm phys}=T_*t,\qquad
T_*=\frac{m_{\rm phys}a_0^2}{\hbar}.
\end{equation}
The transverse trap frequency and longitudinal wave numbers scale as
\begin{equation}
\Omega_\perp=\frac{\omega}{T_*},\qquad
k_{z,{\rm phys}}=\frac{k_z}{a_0},\qquad
\kappa_{\rm phys}=\frac{\kappa}{a_0}.
\end{equation}
The physical transverse oscillator length is
\begin{equation}
\ell_{\perp,{\rm phys}}=\frac{a_0}{\sqrt{\omega}}.
\end{equation}
As an illustrative scale, for single \(^{87}{\rm Rb}\) atoms and \(a_0=2\,\mu{\rm m}\), one obtains
\begin{equation}
T_*\simeq 5.47\,{\rm ms}.
\end{equation}
Thus the observation window \(T=20\) corresponds to approximately \(109\,{\rm ms}\). The values \(\omega=1,100,300\) correspond to transverse oscillator lengths approximately \(2.0\,\mu{\rm m}\), \(0.20\,\mu{\rm m}\), and \(0.115\,\mu{\rm m}\), respectively.

These numbers are reference scales only; the main text does not propose a complete detector design. The experimentally relevant signature is the confinement-controlled deformation of the detector-present roof-flux distribution: increasing \(\omega\) suppresses the early peak, reduces the detected fraction in a fixed observation window, and enhances the delayed oscillatory sector. Over the pre-saturation regime studied here, this enters the finite-window statistic through the local scale \(\sqrt{\omega}\).

A literal implementation of the spinor ABC would require an effective absorbing boundary whose entrance response contains the tangential spin--momentum branches
\begin{equation}
i\kappa\pm|\boldsymbol\xi|.
\end{equation}
Generic spin-dependent loss or bulk spin--orbit terms should not be expected to reproduce this response without engineering the corresponding boundary impedance. The inverse-engineered impedance layer in Sec.~\ref{subsec:SM_layer_mimics} should be viewed only as a proof-of-principle design target: it approaches the spinor-ABC response precisely because the two branch impedances are inserted by construction.

\end{document}
